# Supplementary material for: Quantum Chemical and Trajectory Surface Hopping Molecular Dynamics Study of Iodine-based BODIPY Photosensitizer
Source: arXiv:2411.10893 source file (2025-01-13)
Supplement: Supplementary file 1 [file Supporting_Information_final.pdf]

# Supporting Information

## Quantum Chemical and Trajectory Surface Hopping Molecular Dynamics

### Study of Iodine-based BODIPY Photosensitizer

Mirza Wasif Baig,<sup>1,2</sup> Marek Pederzoli,<sup>1</sup> Mojmír Kývala,<sup>3\*</sup> Jiří Pittner,<sup>1\*</sup>

<sup>1</sup>*J. Heyrovský Institute of Physical Chemistry of the Czech Academy of Sciences, Dolejškova 3, 18223 Prague 8, Czech Republic*

<sup>2</sup>*Faculty of Science, Department of Physical and Macromolecular Chemistry, Charles University, Hlavova 8, 12840 Prague, Czech Republic*

<sup>3</sup>*Institute of Organic Chemistry and Biochemistry of the Czech Academy of Sciences, Flemingovo Nám. 2, 16000 Prague 6, Czech Republic*

### List of electronic structure methods used in the manuscript.

- DHK2 CASSCF and DHK2 CASPT2 using TZP contracted ANO-RCC basis set
- ADC(2) using dhf-TZVP basis set
- TD-DFT with three different functionals B3LYP, BHLYP and M06-2X using aug-cc-pVDZ, aug-cc-pVDZ-PP and dhf-TZVP basis sets
- TD-DFT(TDA) with B3LYP and BHLYP functionals using dhf-TZVP basis set
- sf-X2C-S-TD-DFT with B3LYP, BHLYP(TDA) and M06-2X functionals employing x2c-TZVPPall basis set.

**Table S1a.** Vertical excitation energies [eV] for singlets and triplets of monoiodinated BODIPY in the position 2 at CASPT2(18,15)/ANO-RCC level in optimized  $S_0$  geometry

| State           | Character            | Excitation energy [eV] | Symmetry |
|-----------------|----------------------|------------------------|----------|
| S <sub>1</sub>  | 1( $\pi, \pi^*$ )    | 2.57                   | 2SA'     |
| S <sub>2</sub>  | 2( $\pi, \pi^*$ )    | 3.65                   | 3SA'     |
| S <sub>3</sub>  | 3( $\pi, \pi^*$ )    | 3.68                   | 4SA'     |
| S <sub>4</sub>  | 4( $\pi, \pi^*$ )    | 4.28                   | 5SA'     |
| S <sub>5</sub>  | 1( $\pi, \sigma^*$ ) | 4.84                   | 1SA''    |
| S <sub>6</sub>  | 2( $\pi, \sigma^*$ ) | 4.85                   | 2SA''    |
| S <sub>7</sub>  | 5( $\pi, \pi^*$ )    | 5.48                   | 6SA'     |
| S <sub>8</sub>  | 6( $\pi, \pi^*$ )    | 5.55                   | 3SA''    |
| S <sub>9</sub>  | 1(n, $\pi^*$ )       | 5.95                   | 7SA'     |
| S <sub>10</sub> | 7( $\pi, \pi^*$ )    | 6.18                   | 8SA'     |

| State           | Character            | Excitation energy<br>[eV] | Symmetry |
|-----------------|----------------------|---------------------------|----------|
| T <sub>1</sub>  | 1( $\pi, \pi^*$ )    | 1.90                      | 1TA'     |
| T <sub>2</sub>  | 2( $\pi, \pi^*$ )    | 2.96                      | 2TA'     |
| T <sub>3</sub>  | 3( $\pi, \pi^*$ )    | 3.19                      | 3TA'     |
| T <sub>4</sub>  | 4( $\pi, \pi^*$ )    | 3.87                      | 4TA'     |
| T <sub>5</sub>  | 1( $\pi, \sigma^*$ ) | 4.31                      | 1TA''    |
| T <sub>6</sub>  | 1(n, $\sigma^*$ )    | 4.69                      | 5TA'     |
| T <sub>7</sub>  | 5( $\pi, \pi^*$ )    | 4.94                      | 2TA''    |
| T <sub>8</sub>  | 2( $\pi, \sigma^*$ ) | 5.10                      | 6TA'     |
| T <sub>9</sub>  | 6( $\pi, \pi^*$ )    | 5.37                      | 7TA'     |
| T <sub>10</sub> | 7( $\pi, \pi^*$ )    | 5.56                      | 3TA''    |

**Table S1b.** Vertical excitation energies [eV] for singlets and triplets of monoiodinated BODIPY in the position 2 at ADC(2)/dhf-TZVP level in optimized S<sub>0</sub> geometry

| State           | Character               | Excitation energy [eV] | Symmetry | Oscillator Strength | Orbital overlap |
|-----------------|-------------------------|------------------------|----------|---------------------|-----------------|
| S <sub>1</sub>  | 1( $\pi$ , $\pi^*$ )    | 2.64                   | 2SA'     | 0.53                | 0.67            |
| S <sub>2</sub>  | 2( $\pi$ , $\pi^*$ )    | 3.68                   | 3SA'     | 0.23                | 0.57            |
| S <sub>3</sub>  | 3( $\pi$ , $\pi^*$ )    | 3.82                   | 4SA'     | 0.15                | 0.56            |
| S <sub>4</sub>  | 1(n, $\pi^*$ )          | 4.71                   | 1SA''    | 0.00                | 0.15            |
| S <sub>5</sub>  | 1( $\pi$ , $\sigma^*$ ) | 4.81                   | 2SA''    | 0.00                | 0.41            |
| S <sub>6</sub>  | 4( $\pi$ , $\pi^*$ )    | 5.03                   | 5SA'     | 0.02                | 0.74            |
| S <sub>7</sub>  | 1(n, $\sigma^*$ )       | 5.58                   | 6SA'     | 0.01                | 0.57            |
| S <sub>8</sub>  | 5( $\pi$ , $\pi^*$ )    | 5.62                   | 7SA'     | 0.02                | 0.64            |
| S <sub>9</sub>  | 1( $\sigma$ , $\pi^*$ ) | 5.72                   | 8SA'     | 0.00                | 0.42            |
| S <sub>10</sub> | 2( $\pi$ , $\sigma^*$ ) | 5.93                   | 3SA''    | 0.18                | 0.42            |

| State           | Character               | Excitation energy [eV] | Symmetry | Orbital overlap |
|-----------------|-------------------------|------------------------|----------|-----------------|
| T <sub>1</sub>  | 1( $\pi$ , $\pi^*$ )    | 1.96                   | 1TA'     | 0.69            |
| T <sub>2</sub>  | 2( $\pi$ , $\pi^*$ )    | 2.99                   | 2TA'     | 0.56            |
| T <sub>3</sub>  | 3( $\pi$ , $\pi^*$ )    | 3.27                   | 3TA'     | 0.58            |
| T <sub>4</sub>  | 4( $\pi$ , $\pi^*$ )    | 4.03                   | 4TA'     | 0.72            |
| T <sub>5</sub>  | 1(n, $\pi^*$ )          | 4.34                   | 1TA''    | 0.43            |
| T <sub>6</sub>  | 1( $\pi$ , $\sigma^*$ ) | 4.70                   | 2TA''    | 0.15            |
| T <sub>7</sub>  | 5( $\pi$ , $\pi^*$ )    | 4.93                   | 5TA'     | 0.54            |
| T <sub>8</sub>  | 1(n, $\sigma^*$ )       | 5.39                   | 6TA'     | 0.67            |
| T <sub>9</sub>  | 6( $\pi$ , $\pi^*$ )    | 5.49                   | 7TA'     | 0.71            |
| T <sub>10</sub> | 2( $\pi$ , $\sigma^*$ ) | 5.66                   | 8TA'     | 0.42            |

**Table S1c.** Vertical excitation energies [eV] for singlets and triplets of monoiodinated BODIPY in the position 2 at TD-DFT/B3LYP-D3/dhf-TZVP level in optimized  $S_0$  geometry

| State | Character          | Excitation energy [eV] | Symmetry | Oscillator Strength | Orbital overlap |
|-------|--------------------|------------------------|----------|---------------------|-----------------|
| $S_1$ | $1(\pi, \pi^*)$    | 2.76                   | $2SA'$   | 0.28                | 0.67            |
| $S_2$ | $2(\pi, \pi^*)$    | 3.43                   | $3SA'$   | 0.32                | 0.62            |
| $S_3$ | $1(n, \pi^*)$      | 3.53                   | $1SA''$  | 0.00                | 0.16            |
| $S_4$ | $3(\pi, \pi^*)$    | 3.66                   | $4SA'$   | 0.13                | 0.53            |
| $S_5$ | $1(\pi, \sigma^*)$ | 4.33                   | $2SA''$  | 0.00                | 0.43            |
| $S_6$ | $4(\pi, \pi^*)$    | 4.42                   | $5SA'$   | 0.00                | 0.69            |
| $S_7$ | $2(\pi, \sigma^*)$ | 5.09                   | $3SA''$  | 0.00                | 0.48            |
| $S_8$ | $1(n, \sigma^*)$   | 5.29                   | $6SA'$   | 0.00                | 0.6             |
| $S_9$ | $5(\pi, \pi^*)$    | 5.31                   | $7SA'$   | 0.02                | 0.74            |

| State    | Character          | Excitation energy [eV] | Symmetry | Orbital overlap |
|----------|--------------------|------------------------|----------|-----------------|
| $T_1$    | $1(\pi, \pi^*)$    | 1.54                   | $1TA'$   | 0.68            |
| $T_2$    | $2(\pi, \pi^*)$    | 2.48                   | $2TA'$   | 0.63            |
| $T_3$    | $3(\pi, \pi^*)$    | 2.84                   | $3TA'$   | 0.53            |
| $T_4$    | $4(\pi, \pi^*)$    | 3.45                   | $4TA'$   | 0.70            |
| $T_5$    | $1(n, \pi^*)$      | 3.51                   | $1TA''$  | 0.16            |
| $T_6$    | $1(\pi, \sigma^*)$ | 3.90                   | $2TA''$  | 0.44            |
| $T_7$    | $5(\pi, \pi^*)$    | 4.35                   | $5TA'$   | 0.73            |
| $T_8$    | $1(n, \sigma^*)$   | 4.57                   | $6TA'$   | 0.59            |
| $T_9$    | $6(\pi, \pi^*)$    | 4.76                   | $7TA'$   | 0.76            |
| $T_{10}$ | $2(\pi, \sigma^*)$ | 4.91                   | $3TA''$  | 0.47            |

**Table S1d.** Vertical excitation energies [eV] for singlets and triplets of monoiodinated BODIPY in the position 2 at TD-DFT/BHLYP-D3/dhf-TZVP level in optimized  $S_0$  geometry

| State           | Character               | Excitation energy [eV] | Symmetry | Oscillator Strength | Orbital overlap |
|-----------------|-------------------------|------------------------|----------|---------------------|-----------------|
| S <sub>1</sub>  | 1( $\pi$ , $\pi^*$ )    | 3.04                   | 2SA'     | 0.59                | 0.69            |
| S <sub>2</sub>  | 2( $\pi$ , $\pi^*$ )    | 3.95                   | 3SA'     | 0.16                | 0.58            |
| S <sub>3</sub>  | 3( $\pi$ , $\pi^*$ )    | 4.24                   | 4SA'     | 0.06                | 0.54            |
| S <sub>4</sub>  | 1( $\pi$ , $\sigma^*$ ) | 4.70                   | 1SA''    | 0.00                | 0.41            |
| S <sub>5</sub>  | 1(n, $\pi^*$ )          | 4.74                   | 2SA''    | 0.00                | 0.15            |
| S <sub>6</sub>  | 4( $\pi$ , $\pi^*$ )    | 5.33                   | 5SA'     | 0.00                | 0.71            |
| S <sub>7</sub>  | 1(n, $\sigma^*$ )       | 5.56                   | 6SA'     | 0.00                | 0.58            |
| S <sub>8</sub>  | 2( $\pi$ , $\sigma^*$ ) | 5.90                   | 3SA''    | 0.00                | 0.46            |
| S <sub>9</sub>  | 5( $\pi$ , $\pi^*$ )    | 5.98                   | 7SA'     | 0.05                | 0.73            |
| S <sub>10</sub> | 6( $\pi$ , $\pi^*$ )    | 6.39                   | 8SA'     | 0.14                | 0.76            |

| State           | Character               | Excitation energy | Symmetry | Orbital overlap |
|-----------------|-------------------------|-------------------|----------|-----------------|
| T <sub>1</sub>  | 1( $\pi$ , $\pi^*$ )    | 1.19              | 1TA'     | 0.68            |
| T <sub>2</sub>  | 2( $\pi$ , $\pi^*$ )    | 2.73              | 2TA'     | 0.59            |
| T <sub>3</sub>  | 3( $\pi$ , $\pi^*$ )    | 2.97              | 3TA'     | 0.57            |
| T <sub>4</sub>  | 4( $\pi$ , $\pi^*$ )    | 3.45              | 4TA'     | 0.70            |
| T <sub>5</sub>  | 1( $\pi$ , $\sigma^*$ ) | 4.12              | 1TA''    | 0.43            |
| T <sub>6</sub>  | 1(n, $\pi^*$ )          | 4.70              | 2TA''    | 0.15            |
| T <sub>7</sub>  | 1(n, $\sigma^*$ )       | 4.74              | 5TA'     | 0.58            |
| T <sub>8</sub>  | 5( $\pi$ , $\pi^*$ )    | 4.86              | 6TA'     | 0.74            |
| T <sub>9</sub>  | 6( $\pi$ , $\pi^*$ )    | 5.22              | 7TA'     | 0.70            |
| T <sub>10</sub> | 7( $\pi$ , $\pi^*$ )    | 5.38              | 8TA'     | 0.70            |

**Table S1e.** Vertical excitation energies [eV] for singlets and triplets of monoiodinated BODIPY in the position 2 at TD-DFT/M06-2X-D3/dhf-TZVP level in optimized  $S_0$  geometry

| State    | Character          | Excitation energy [eV] | Symmetry | Oscillator Strength | Orbital overlap |
|----------|--------------------|------------------------|----------|---------------------|-----------------|
| $S_1$    | $1(\pi, \pi^*)$    | 2.99                   | $2SA'$   | 0.52                | 0.68            |
| $S_2$    | $2(\pi, \pi^*)$    | 3.90                   | $3SA'$   | 0.17                | 0.59            |
| $S_3$    | $3(\pi, \pi^*)$    | 4.17                   | $4SA'$   | 0.06                | 0.54            |
| $S_4$    | $1(n, \pi^*)$      | 4.62                   | $1SA''$  | 0.00                | 0.16            |
| $S_5$    | $1(\pi, \sigma^*)$ | 4.75                   | $2SA''$  | 0.00                | 0.43            |
| $S_6$    | $4(\pi, \pi^*)$    | 5.27                   | $5SA'$   | 0.00                | 0.70            |
| $S_7$    | $1(n, \sigma^*)$   | 5.51                   | $6SA'$   | 0.00                | 0.59            |
| $S_8$    | $2(\pi, \sigma^*)$ | 5.91                   | $3SA''$  | 0.00                | 0.46            |
| $S_9$    | $5(\pi, \pi^*)$    | 5.97                   | $7SA'$   | 0.06                | 0.74            |
| $S_{10}$ | $1(\sigma, \pi^*)$ | 6.17                   | $4SA''$  | 0.14                | 0.39            |

| State    | Character          | Excitation energy [eV] | Symmetry | Orbital overlap |
|----------|--------------------|------------------------|----------|-----------------|
| $T_1$    | $1(\pi, \pi^*)$    | 1.52                   | $1TA'$   | 0.68            |
| $T_2$    | $2(\pi, \pi^*)$    | 3.02                   | $2TA'$   | 0.59            |
| $T_3$    | $3(\pi, \pi^*)$    | 3.30                   | $3TA'$   | 0.55            |
| $T_4$    | $4(\pi, \pi^*)$    | 3.86                   | $4TA'$   | 0.72            |
| $T_5$    | $1(\pi, \sigma^*)$ | 4.31                   | $1TA''$  | 0.44            |
| $T_6$    | $1(n, \pi^*)$      | 4.59                   | $2TA''$  | 0.16            |
| $T_7$    | $1(n, \sigma^*)$   | 4.87                   | $5TA'$   | 0.59            |
| $T_8$    | $5(\pi, \pi^*)$    | 5.25                   | $6TA'$   | 0.72            |
| $T_9$    | $6(\pi, \pi^*)$    | 5.42                   | $7TA'$   | 0.75            |
| $T_{10}$ | $7(\pi, \pi^*)$    | 5.74                   | $8TA'$   | 0.73            |

**Table S1f.** Vertical excitation energies [eV] for singlets and triplets of monoiodinated BODIPY in the position 2 at TD-DFT(TDA)/B3LYP-D3/dhf-TZVP level in optimized  $S_0$  geometry

| State           | Character               | Excitation energy [eV] | Symmetry | Oscillator Strength | Orbital overlap |
|-----------------|-------------------------|------------------------|----------|---------------------|-----------------|
| S <sub>1</sub>  | 1( $\pi$ , $\pi^*$ )    | 2.94                   | 2SA'     | 0.25                | 0.66            |
| S <sub>2</sub>  | 1(n, $\pi^*$ )          | 3.53                   | 1SA''    | 0.00                | 0.16            |
| S <sub>3</sub>  | 2( $\pi$ , $\pi^*$ )    | 3.68                   | 3SA'     | 0.02                | 0.57            |
| S <sub>4</sub>  | 3( $\pi$ , $\pi^*$ )    | 3.91                   | 4SA'     | 0.06                | 0.6             |
| S <sub>5</sub>  | 1( $\pi$ , $\sigma^*$ ) | 4.37                   | 2SA''    | 0.00                | 0.43            |
| S <sub>6</sub>  | 4( $\pi$ , $\pi^*$ )    | 4.48                   | 5SA'     | 0.00                | 0.69            |
| S <sub>7</sub>  | 2( $\pi$ , $\sigma^*$ ) | 5.10                   | 3SA''    | 0.00                | 0.48            |
| S <sub>8</sub>  | 1( $\sigma$ , $\pi^*$ ) | 5.32                   | 4SA''    | 0.00                | 0.36            |
| S <sub>9</sub>  | 1(n, $\sigma^*$ )       | 5.35                   | 6SA'     | 0.00                | 0.59            |
| S <sub>10</sub> | 5( $\pi$ , $\pi^*$ )    | 5.44                   | 7SA'     | 0.01                | 0.74            |

| State           | Character               | Excitation energy [eV] | Symmetry | Orbital overlap |
|-----------------|-------------------------|------------------------|----------|-----------------|
| T <sub>1</sub>  | 1( $\pi$ , $\pi^*$ )    | 1.66                   | 1TA'     | 0.68            |
| T <sub>2</sub>  | 2( $\pi$ , $\pi^*$ )    | 2.58                   | 2TA'     | 0.63            |
| T <sub>3</sub>  | 3( $\pi$ , $\pi^*$ )    | 2.94                   | 3TA'     | 0.53            |
| T <sub>4</sub>  | 1(n, $\pi^*$ )          | 3.51                   | 1TA''    | 0.16            |
| T <sub>5</sub>  | 4( $\pi$ , $\pi^*$ )    | 3.58                   | 4TA'     | 0.70            |
| T <sub>6</sub>  | 1( $\pi$ , $\sigma^*$ ) | 3.94                   | 2TA''    | 0.44            |
| T <sub>7</sub>  | 5( $\pi$ , $\pi^*$ )    | 4.39                   | 5TA'     | 0.73            |
| T <sub>8</sub>  | 1(n, $\sigma^*$ )       | 4.62                   | 6TA'     | 0.59            |
| T <sub>9</sub>  | 6( $\pi$ , $\pi^*$ )    | 4.87                   | 7TA'     | 0.76            |
| T <sub>10</sub> | 1( $\pi$ , $\sigma^*$ ) | 4.92                   | 3TA''    | 0.47            |



**Table S1g.** Vertical excitation energies [eV] for singlets and triplets of monoiodinated BODIPY in the position 2 at TD-DFT(TDA)/BHLYP-D3/dhf-TZVP level in optimized S<sub>0</sub> geometry

| State           | Character               | Excitation energy [eV] | Symmetry | Oscillator Strength | Orbital overlap |
|-----------------|-------------------------|------------------------|----------|---------------------|-----------------|
| S <sub>1</sub>  | 1( $\pi$ , $\pi^*$ )    | 3.32                   | 2SA'     | 0.10                | 0.68            |
| S <sub>2</sub>  | 2( $\pi$ , $\pi^*$ )    | 4.13                   | 3SA'     | 0.04                | 0.59            |
| S <sub>3</sub>  | 3( $\pi$ , $\pi^*$ )    | 4.39                   | 4SA'     | 0.00                | 0.54            |
| S <sub>4</sub>  | 1(n, $\pi^*$ )          | 4.74                   | 1SA''    | 0.00                | 0.23            |
| S <sub>5</sub>  | 1( $\pi$ , $\sigma^*$ ) | 4.76                   | 2SA''    | 0.00                | 0.34            |
| S <sub>6</sub>  | 4( $\pi$ , $\pi^*$ )    | 5.43                   | 5SA'     | 0.00                | 0.71            |
| S <sub>7</sub>  | 1(n, $\sigma^*$ )       | 5.63                   | 6SA'     | 0.00                | 0.58            |
| S <sub>8</sub>  | 2( $\pi$ , $\sigma^*$ ) | 5.91                   | 3SA''    | 0.00                | 0.46            |
| S <sub>9</sub>  | 5( $\pi$ , $\pi^*$ )    | 6.13                   | 7SA'     | 0.00                | 0.74            |
| S <sub>10</sub> | 1( $\sigma$ , $\pi^*$ ) | 6.55                   | 4SA''    | 0.00                | 0.37            |

| State           | Character               | Excitation energy [eV] | Symmetry | Orbital overlap |
|-----------------|-------------------------|------------------------|----------|-----------------|
| T <sub>1</sub>  | 1( $\pi$ , $\pi^*$ )    | 1.63                   | 1TA'     | 0.68            |
| T <sub>2</sub>  | 2( $\pi$ , $\pi^*$ )    | 3.00                   | 2TA'     | 0.59            |
| T <sub>3</sub>  | 3( $\pi$ , $\pi^*$ )    | 3.26                   | 3TA'     | 0.55            |
| T <sub>4</sub>  | 4( $\pi$ , $\pi^*$ )    | 3.73                   | 4TA'     | 0.72            |
| T <sub>5</sub>  | 1( $\pi$ , $\sigma^*$ ) | 4.19                   | 1TA''    | 0.44            |
| T <sub>6</sub>  | 1(n, $\pi^*$ )          | 4.71                   | 2TA''    | 0.15            |
| T <sub>7</sub>  | 1(n, $\sigma^*$ )       | 4.82                   | 5TA'     | 0.58            |
| T <sub>8</sub>  | 5( $\pi$ , $\pi^*$ )    | 5.12                   | 6TA'     | 0.75            |
| T <sub>9</sub>  | 6( $\pi$ , $\pi^*$ )    | 5.34                   | 7TA'     | 0.71            |
| T <sub>10</sub> | 7( $\pi$ , $\pi^*$ )    | 5.54                   | 8TA'     | 0.72            |

**Table S2a.** Vertical excitation energies [eV] for singlets and triplets of I-BODIPY at ADC(2)/dhf-TZVP level in optimized  $S_0$  geometry

| State          | Character               | Excitation energy [eV] | Oscillator Strength | Orbital overlap |
|----------------|-------------------------|------------------------|---------------------|-----------------|
| S <sub>1</sub> | 1( $\pi$ , $\pi^*$ )    | 2.56                   | 0.58                | 0.67            |
| S <sub>2</sub> | 2( $\pi$ , $\pi^*$ )    | 3.22                   | 0.22                | 0.47            |
| S <sub>3</sub> | 3( $\pi$ , $\pi^*$ )    | 3.49                   | 0.11                | 0.59            |
| S <sub>4</sub> | 1( $\pi$ , $\sigma^*$ ) | 4.39                   | 0.00                | 0.37            |
| S <sub>5</sub> | 1(n, $\pi^*$ )          | 4.52                   | 0.00                | 0.15            |
| S <sub>6</sub> | 2( $\pi$ , $\sigma^*$ ) | 4.59                   | 0.00                | 0.52            |
| S <sub>7</sub> | 2(n, $\pi^*$ )          | 4.83                   | 0.01                | 0.24            |
| S <sub>8</sub> | 4( $\pi$ , $\pi^*$ )    | 4.84                   | 0.07                | 0.54            |

| State          | Character               | Excitation energy [eV] | Orbital overlap |
|----------------|-------------------------|------------------------|-----------------|
| T <sub>1</sub> | 1( $\pi$ , $\pi^*$ )    | 1.91                   | 0.69            |
| T <sub>2</sub> | 2( $\pi$ , $\pi^*$ )    | 2.78                   | 0.50            |
| T <sub>3</sub> | 3( $\pi$ , $\pi^*$ )    | 3.00                   | 0.54            |
| T <sub>4</sub> | 4( $\pi$ , $\pi^*$ )    | 3.92                   | 0.64            |
| T <sub>5</sub> | 1( $\pi$ , $\sigma^*$ ) | 4.09                   | 0.47            |
| T <sub>6</sub> | 2( $\pi$ , $\sigma^*$ ) | 4.22                   | 0.44            |
| T <sub>7</sub> | 1(n, $\pi^*$ )          | 4.52                   | 0.15            |
| T <sub>8</sub> | 1(n, $\sigma^*$ )       | 4.71                   | 0.50            |
| T <sub>9</sub> | 2(n, $\pi^*$ )          | 4.81                   | 0.21            |

**Table S2b.** Vertical excitation energies [eV] for singlets and triplets of I-BODIPY at ADC(2)/dhf-TZVP level in optimized S<sub>1</sub> geometry

| State          | Character               | Excitation energy [eV] | Oscillator Strength | Orbital overlap |
|----------------|-------------------------|------------------------|---------------------|-----------------|
| S <sub>1</sub> | 1( $\pi$ , $\pi^*$ )    | 2.13                   | 0.17                | 0.56            |
| S <sub>2</sub> | 2( $\pi$ , $\pi^*$ )    | 2.64                   | 0.42                | 0.52            |
| S <sub>3</sub> | 3( $\pi$ , $\pi^*$ )    | 3.37                   | 0.07                | 0.63            |
| S <sub>4</sub> | 1(n, $\pi^*$ )          | 4.16                   | 0.00                | 0.13            |
| S <sub>5</sub> | 2(n, $\pi^*$ )          | 4.41                   | 0.00                | 0.18            |
| S <sub>6</sub> | 1( $\pi$ , $\sigma^*$ ) | 4.47                   | 0.00                | 0.48            |
| S <sub>7</sub> | 4( $\pi$ , $\pi^*$ )    | 4.56                   | 0.14                | 0.61            |
| S <sub>8</sub> | 2( $\pi$ , $\sigma^*$ ) | 4.69                   | 0.00                | 0.39            |

| State          | Character               | Excitation energy [eV] | Orbital overlap |
|----------------|-------------------------|------------------------|-----------------|
| T <sub>1</sub> | 1( $\pi$ , $\pi^*$ )    | 1.82                   | 0.61            |
| T <sub>2</sub> | 2( $\pi$ , $\pi^*$ )    | 2.19                   | 0.47            |
| T <sub>3</sub> | 3( $\pi$ , $\pi^*$ )    | 2.78                   | 0.63            |
| T <sub>4</sub> | 4( $\pi$ , $\pi^*$ )    | 3.62                   | 0.66            |
| T <sub>5</sub> | 1( $\pi$ , $\sigma^*$ ) | 4.11                   | 0.50            |
| T <sub>6</sub> | 1(n, $\pi^*$ )          | 4.16                   | 0.13            |
| T <sub>7</sub> | 2( $\pi$ , $\sigma^*$ ) | 4.31                   | 0.39            |
| T <sub>8</sub> | 2(n, $\pi^*$ )          | 4.40                   | 0.19            |
| T <sub>9</sub> | 1(n, $\sigma^*$ )       | 4.85                   | 0.49            |

**Table S2c.** Vertical excitation energies [eV] for singlets and triplets of I-BODIPY at ADC(2)/dhf-TZVP level in optimized T<sub>2</sub> geometry

| State          | Character               | Excitation energy [eV] | Oscillator Strength | Orbital overlap |
|----------------|-------------------------|------------------------|---------------------|-----------------|
| S <sub>1</sub> | 1( $\pi$ , $\pi^*$ )    | 2.52                   | 0.56                | 0.33            |
| S <sub>2</sub> | 2( $\pi$ , $\pi^*$ )    | 3.18                   | 0.22                | 0.47            |
| S <sub>3</sub> | 3( $\pi$ , $\pi^*$ )    | 3.45                   | 0.10                | 0.60            |
| S <sub>4</sub> | 1( $\pi$ , $\sigma^*$ ) | 4.31                   | 0.00                | 0.60            |
| S <sub>5</sub> | 1(n, $\pi^*$ )          | 4.50                   | 0.00                | 0.15            |
| S <sub>6</sub> | 2( $\pi$ , $\sigma^*$ ) | 4.51                   | 0.00                | 0.52            |
| S <sub>7</sub> | 4( $\pi$ , $\pi^*$ )    | 4.79                   | 0.07                | 0.52            |
| S <sub>8</sub> | 2(n, $\pi^*$ )          | 4.80                   | 0.01                | 0.26            |

| State          | Character               | Excitation energy [eV] | Orbital overlap |
|----------------|-------------------------|------------------------|-----------------|
| T <sub>1</sub> | 1( $\pi$ , $\pi^*$ )    | 1.88                   | 0.69            |
| T <sub>2</sub> | 2( $\pi$ , $\pi^*$ )    | 2.76                   | 0.50            |
| T <sub>3</sub> | 3( $\pi$ , $\pi^*$ )    | 2.97                   | 0.54            |
| T <sub>4</sub> | 4( $\pi$ , $\pi^*$ )    | 3.87                   | 0.64            |
| T <sub>5</sub> | 1( $\pi$ , $\sigma^*$ ) | 4.01                   | 0.46            |
| T <sub>6</sub> | 2( $\pi$ , $\sigma^*$ ) | 4.13                   | 0.43            |
| T <sub>7</sub> | 1(n, $\pi^*$ )          | 4.50                   | 0.14            |
| T <sub>8</sub> | 1(n, $\sigma^*$ )       | 4.62                   | 0.47            |
| T <sub>9</sub> | 2(n, $\pi^*$ )          | 4.78                   | 0.21            |

**Table S3a.** Vertical excitation energies [eV] for singlets and triplets of I-BODIPY at TD-DFT/B3LYP-D3/dhf-TZVP level in optimized  $S_0$  geometry

| State    | Character          | Excitation energy [eV] | Oscillator Strength | Orbital overlap |
|----------|--------------------|------------------------|---------------------|-----------------|
| $S_1$    | $1(\pi, \pi^*)$    | 2.75                   | 0.33                | 0.65            |
| $S_2$    | $2(\pi, \pi^*)$    | 3.01                   | 0.37                | 0.55            |
| $S_3$    | $3(\pi, \pi^*)$    | 3.36                   | 0.08                | 0.54            |
| $S_4$    | $1(n, \pi^*)$      | 3.52                   | 0.00                | 0.17            |
| $S_5$    | $1(\pi, \sigma^*)$ | 3.79                   | 0.00                | 0.35            |
| $S_6$    | $2(n, \pi^*)$      | 3.92                   | 0.00                | 0.24            |
| $S_7$    | $4(\pi, \pi^*)$    | 4.11                   | 0.05                | 0.58            |
| $S_8$    | $2(\pi, \sigma^*)$ | 4.12                   | 0.00                | 0.61            |
| $S_9$    | $3(\pi, \sigma^*)$ | 4.66                   | 0.00                | 0.40            |
| $S_{10}$ | $1(n, \sigma^*)$   | 4.85                   | 0.00                | 0.58            |

| State    | Character          | Excitation energy [eV] | Orbital overlap |
|----------|--------------------|------------------------|-----------------|
| $T_1$    | $1(\pi, \pi^*)$    | 1.44                   | 0.70            |
| $T_2$    | $2(\pi, \pi^*)$    | 1.89                   | 0.51            |
| $T_3$    | $3(\pi, \pi^*)$    | 2.41                   | 0.53            |
| $T_4$    | $4(\pi, \pi^*)$    | 3.04                   | 0.62            |
| $T_5$    | $1(n, \pi^*)$      | 3.17                   | 0.17            |
| $T_6$    | $2(n, \pi^*)$      | 3.54                   | 0.40            |
| $T_7$    | $1(\pi, \sigma^*)$ | 3.65                   | 0.55            |
| $T_8$    | $2(\pi, \sigma^*)$ | 3.86                   | 0.24            |
| $T_9$    | $5(\pi, \pi^*)$    | 3.99                   | 0.68            |
| $T_{10}$ | $6(\pi, \pi^*)$    | 4.19                   | 0.56            |

**Table S3b.** Vertical excitation energies [eV] for singlets and triplets of I-BODIPY at TD-DFT/B3LYP-D3/dhf-TZVP level in optimized S<sub>1</sub> geometry

| State           | Character               | Excitation energy [eV] | Oscillator Strength | Orbital overlap |
|-----------------|-------------------------|------------------------|---------------------|-----------------|
| S <sub>1</sub>  | 1( $\pi$ , $\pi^*$ )    | 2.25                   | 0.06                | 0.60            |
| S <sub>2</sub>  | 2( $\pi$ , $\pi^*$ )    | 2.77                   | 0.55                | 0.62            |
| S <sub>3</sub>  | 1(n, $\pi^*$ )          | 3.19                   | 0.00                | 0.16            |
| S <sub>4</sub>  | 3( $\pi$ , $\pi^*$ )    | 3.26                   | 0.04                | 0.54            |
| S <sub>5</sub>  | 2(n, $\pi^*$ )          | 3.58                   | 0.00                | 0.20            |
| S <sub>6</sub>  | 4( $\pi$ , $\pi^*$ )    | 3.88                   | 0.09                | 0.62            |
| S <sub>7</sub>  | 1( $\pi$ , $\sigma^*$ ) | 3.98                   | 0.00                | 0.35            |
| S <sub>8</sub>  | 2( $\pi$ , $\sigma^*$ ) | 4.20                   | 0.00                | 0.52            |
| S <sub>9</sub>  | 5( $\pi$ , $\pi^*$ )    | 4.41                   | 0.02                | 0.47            |
| S <sub>10</sub> | 1( $\pi$ , $\sigma^*$ ) | 4.64                   | 0.00                | 0.48            |

| State           | Character               | Excitation energy [eV] | Orbital overlap |
|-----------------|-------------------------|------------------------|-----------------|
| T <sub>1</sub>  | 1( $\pi$ , $\pi^*$ )    | 1.51                   | 0.60            |
| T <sub>2</sub>  | 2( $\pi$ , $\pi^*$ )    | 2.40                   | 0.62            |
| T <sub>3</sub>  | 3( $\pi$ , $\pi^*$ )    | 2.59                   | 0.54            |
| T <sub>4</sub>  | 4( $\pi$ , $\pi^*$ )    | 3.33                   | 0.63            |
| T <sub>5</sub>  | 1(n, $\pi^*$ )          | 3.50                   | 0.16            |
| T <sub>6</sub>  | 1( $\pi$ , $\sigma^*$ ) | 3.58                   | 0.20            |
| T <sub>7</sub>  | 2( $\pi$ , $\sigma^*$ ) | 3.72                   | 0.45            |
| T <sub>8</sub>  | 2(n, $\pi^*$ )          | 3.89                   | 0.45            |
| T <sub>9</sub>  | 5( $\pi$ , $\pi^*$ )    | 4.20                   | 0.56            |
| T <sub>10</sub> | 1(n, $\sigma^*$ )       | 4.30                   | 0.60            |

**Table S3c.** Vertical excitation energies [eV] for singlets and triplets of I-BODIPY at TD-DFT/B3LYP-D3/dhf-TZVP level in optimized T<sub>2</sub> geometry

| State           | Character               | Excitation energy [eV] | Oscillator Strength | Orbital overlap |
|-----------------|-------------------------|------------------------|---------------------|-----------------|
| S <sub>1</sub>  | 1( $\pi$ , $\pi^*$ )    | 2.72                   | 0.33                | 0.65            |
| S <sub>2</sub>  | 2( $\pi$ , $\pi^*$ )    | 2.98                   | 0.36                | 0.55            |
| S <sub>3</sub>  | 3( $\pi$ , $\pi^*$ )    | 3.32                   | 0.08                | 0.54            |
| S <sub>4</sub>  | 1(n, $\pi^*$ )          | 3.50                   | 0.00                | 0.16            |
| S <sub>5</sub>  | 1( $\pi$ , $\sigma^*$ ) | 3.71                   | 0.00                | 0.35            |
| S <sub>6</sub>  | 2(n, $\pi^*$ )          | 3.88                   | 0.00                | 0.22            |
| S <sub>7</sub>  | 2( $\pi$ , $\sigma^*$ ) | 4.05                   | 0.00                | 0.61            |
| S <sub>8</sub>  | 4( $\pi$ , $\pi^*$ )    | 4.07                   | 0.03                | 0.58            |
| S <sub>9</sub>  | 3( $\pi$ , $\sigma^*$ ) | 4.56                   | 0.00                | 0.41            |
| S <sub>10</sub> | 1(n, $\sigma^*$ )       | 4.77                   | 0.00                | 0.57            |

| State           | Character               | Excitation energy [eV] | Orbital overlap |
|-----------------|-------------------------|------------------------|-----------------|
| T <sub>1</sub>  | 1( $\pi$ , $\pi^*$ )    | 1.47                   | 0.70            |
| T <sub>2</sub>  | 2( $\pi$ , $\pi^*$ )    | 2.37                   | 0.51            |
| T <sub>3</sub>  | 3( $\pi$ , $\pi^*$ )    | 2.56                   | 0.53            |
| T <sub>4</sub>  | 4( $\pi$ , $\pi^*$ )    | 3.28                   | 0.62            |
| T <sub>5</sub>  | 1(n, $\pi^*$ )          | 3.48                   | 0.16            |
| T <sub>6</sub>  | 1( $\pi$ , $\sigma^*$ ) | 3.50                   | 0.40            |
| T <sub>7</sub>  | 2( $\pi$ , $\sigma^*$ ) | 3.63                   | 0.55            |
| T <sub>8</sub>  | 2(n, $\pi^*$ )          | 3.85                   | 0.22            |
| T <sub>9</sub>  | 5( $\pi$ , $\pi^*$ )    | 4.14                   | 0.68            |
| T <sub>10</sub> | 1(n, $\sigma^*$ )       | 4.22                   | 0.56            |

**Table S4a.** Vertical excitation energies [eV] for singlets and triplets of I-BODIPY at TD-DFT/BHLYP-D3/dhf-TZVP level in optimized  $S_0$  geometry

| State    | Character          | Excitation energy [eV] | Oscillator Strength | Orbital Overlap |
|----------|--------------------|------------------------|---------------------|-----------------|
| $S_1$    | $1(\pi, \pi^*)$    | 2.96                   | 0.74                | 0.70            |
| $S_2$    | $2(\pi, \pi^*)$    | 3.66                   | 0.10                | 0.48            |
| $S_3$    | $3(\pi, \pi^*)$    | 3.93                   | 0.08                | 0.55            |
| $S_4$    | $1(\pi, \sigma^*)$ | 4.37                   | 0.00                | 0.38            |
| $S_5$    | $2(\pi, \sigma^*)$ | 4.54                   | 0.00                | 0.55            |
| $S_6$    | $1(n, \pi^*)$      | 4.65                   | 0.00                | 0.16            |
| $S_7$    | $2(n, \pi^*)$      | 5.04                   | 0.00                | 0.23            |
| $S_8$    | $4(\pi, \pi^*)$    | 5.05                   | 0.03                | 0.54            |
| $S_9$    | $1(n, \sigma^*)$   | 5.31                   | 0.00                | 0.55            |
| $S_{10}$ | $3(\pi, \sigma^*)$ | 5.38                   | 0.00                | 0.46            |

| State    | Character          | Excitation energy [eV] | Orbital Overlap |
|----------|--------------------|------------------------|-----------------|
| $T_1$    | $1(\pi, \pi^*)$    | 1.14                   | 0.69            |
| $T_2$    | $2(\pi, \pi^*)$    | 2.61                   | 0.54            |
| $T_3$    | $3(\pi, \pi^*)$    | 2.88                   | 0.51            |
| $T_4$    | $4(\pi, \pi^*)$    | 3.45                   | 0.66            |
| $T_5$    | $1(\pi, \sigma^*)$ | 3.91                   | 0.50            |
| $T_6$    | $2(\pi, \sigma^*)$ | 4.07                   | 0.47            |
| $T_7$    | $1(n, \sigma^*)$   | 4.56                   | 0.55            |
| $T_8$    | $1(n, \pi^*)$      | 4.62                   | 0.16            |
| $T_9$    | $5(\pi, \pi^*)$    | 4.67                   | 0.65            |
| $T_{10}$ | $2(n, \sigma^*)$   | 4.74                   | 0.58            |



**Table S4b.** Vertical excitation energies [eV] for singlets and triplets of I-BODIPY at TD-DFT/BHLYP-D3/dhf-TZVP level in optimized S<sub>1</sub> geometry

| State           | Character               | Excitation energy [eV] | Oscillator Strength | Orbital Overlap |
|-----------------|-------------------------|------------------------|---------------------|-----------------|
| S <sub>1</sub>  | 1( $\pi$ , $\pi^*$ )    | 2.79                   | 0.99                | 0.60            |
| S <sub>2</sub>  | 2( $\pi$ , $\pi^*$ )    | 3.16                   | 0.00                | 0.55            |
| S <sub>3</sub>  | 3( $\pi$ , $\pi^*$ )    | 3.77                   | 0.27                | 0.58            |
| S <sub>4</sub>  | 1(n, $\pi^*$ )          | 4.34                   | 0.38                | 0.15            |
| S <sub>5</sub>  | 1( $\pi$ , $\sigma^*$ ) | 4.48                   | 0.02                | 0.49            |
| S <sub>6</sub>  | 2( $\pi$ , $\sigma^*$ ) | 4.64                   | 0.00                | 0.42            |
| S <sub>7</sub>  | 2(n, $\pi^*$ )          | 4.69                   | 0.00                | 0.18            |
| S <sub>8</sub>  | 4( $\pi$ , $\pi^*$ )    | 4.78                   | 0.30                | 0.60            |
| S <sub>9</sub>  | 3( $\pi$ , $\sigma^*$ ) | 5.31                   | 0.00                | 0.40            |
| S <sub>10</sub> | 5( $\pi$ , $\pi^*$ )    | 5.38                   | 0.00                | 0.49            |

| State           | Character               | Excitation energy [eV] | Orbital Overlap |
|-----------------|-------------------------|------------------------|-----------------|
| T <sub>1</sub>  | 1( $\pi$ , $\pi^*$ )    | 1.12                   | 0.59            |
| T <sub>2</sub>  | 2( $\pi$ , $\pi^*$ )    | 2.29                   | 0.57            |
| T <sub>3</sub>  | 3( $\pi$ , $\pi^*$ )    | 2.50                   | 0.56            |
| T <sub>4</sub>  | 4( $\pi$ , $\pi^*$ )    | 3.19                   | 0.63            |
| T <sub>5</sub>  | 1( $\pi$ , $\sigma^*$ ) | 3.96                   | 0.52            |
| T <sub>6</sub>  | 2( $\pi$ , $\sigma^*$ ) | 4.13                   | 0.43            |
| T <sub>7</sub>  | 1(n, $\pi^*$ )          | 4.32                   | 0.15            |
| T <sub>8</sub>  | 5( $\pi$ , $\pi^*$ )    | 4.50                   | 0.57            |
| T <sub>9</sub>  | 2(n, $\pi^*$ )          | 4.65                   | 0.18            |
| T <sub>10</sub> | 1(n, $\sigma^*$ )       | 4.70                   | 0.53            |

**Table S4c.** Vertical excitation energies [eV] for singlets and triplets of I-BODIPY at TD-DFT/BHLYP-D3/dhf-TZVP level in optimized T<sub>2</sub> geometry

| State           | Character               | Excitation energy [eV] | Oscillator Strength | Orbital Overlap |
|-----------------|-------------------------|------------------------|---------------------|-----------------|
| S <sub>1</sub>  | 1( $\pi$ , $\pi^*$ )    | 2.92                   | 0.73                | 0.70            |
| S <sub>2</sub>  | 2( $\pi$ , $\pi^*$ )    | 3.64                   | 0.10                | 0.48            |
| S <sub>3</sub>  | 3( $\pi$ , $\pi^*$ )    | 3.90                   | 0.08                | 0.55            |
| S <sub>4</sub>  | 1( $\pi$ , $\sigma^*$ ) | 4.29                   | 0.00                | 0.38            |
| S <sub>5</sub>  | 2( $\pi$ , $\sigma^*$ ) | 4.46                   | 0.00                | 0.55            |
| S <sub>6</sub>  | 1(n, $\pi^*$ )          | 4.63                   | 0.00                | 0.16            |
| S <sub>7</sub>  | 4( $\pi$ , $\pi^*$ )    | 5.01                   | 0.03                | 0.55            |
| S <sub>8</sub>  | 2(n, $\pi^*$ )          | 5.02                   | 0.00                | 0.21            |
| S <sub>9</sub>  | 1(n, $\sigma^*$ )       | 5.22                   | 0.00                | 0.55            |
| S <sub>10</sub> | 3( $\pi$ , $\sigma^*$ ) | 5.28                   | 0.00                | 0.46            |

| State           | Character               | Excitation energy [eV] | Orbital Overlap |
|-----------------|-------------------------|------------------------|-----------------|
| T <sub>1</sub>  | 1( $\pi$ , $\pi^*$ )    | 1.09                   | 0.69            |
| T <sub>2</sub>  | 2( $\pi$ , $\pi^*$ )    | 2.56                   | 0.54            |
| T <sub>3</sub>  | 3( $\pi$ , $\pi^*$ )    | 2.85                   | 0.51            |
| T <sub>4</sub>  | 4( $\pi$ , $\pi^*$ )    | 3.39                   | 0.66            |
| T <sub>5</sub>  | 1( $\pi$ , $\sigma^*$ ) | 3.83                   | 0.50            |
| T <sub>6</sub>  | 2( $\pi$ , $\sigma^*$ ) | 3.98                   | 0.47            |
| T <sub>7</sub>  | 1(n, $\sigma^*$ )       | 4.47                   | 0.55            |
| T <sub>8</sub>  | 5( $\pi$ , $\pi^*$ )    | 4.60                   | 0.64            |
| T <sub>9</sub>  | 1(n, $\pi^*$ )          | 4.60                   | 0.17            |
| T <sub>10</sub> | 2(n, $\sigma^*$ )       | 4.65                   | 0.58            |

**Table S5a.** Vertical excitation energies [eV] for singlets and triplets of I-BODIPY at TD-DFT/M06-2X-D3/dhf-TZVP level in optimized  $S_0$  geometry

| State    | Character          | Excitation energy [eV] | Oscillator Strength | Orbital overlap |
|----------|--------------------|------------------------|---------------------|-----------------|
| $S_1$    | $1(\pi, \pi^*)$    | 2.91                   | 0.66                | 0.70            |
| $S_2$    | $2(\pi, \pi^*)$    | 3.57                   | 0.11                | 0.48            |
| $S_3$    | $3(\pi, \pi^*)$    | 3.83                   | 0.07                | 0.54            |
| $S_4$    | $1(\pi, \sigma^*)$ | 4.40                   | 0.00                | 0.39            |
| $S_5$    | $1(n, \pi^*)$      | 4.54                   | 0.00                | 0.18            |
| $S_6$    | $2(\pi, \sigma^*)$ | 4.56                   | 0.00                | 0.54            |
| $S_7$    | $2(n, \pi^*)$      | 4.89                   | 0.00                | 0.21            |
| $S_8$    | $4(\pi, \pi^*)$    | 5.00                   | 0.02                | 0.57            |
| $S_9$    | $1(n, \sigma^*)$   | 5.25                   | 0.00                | 0.56            |
| $S_{10}$ | $3(\pi, \sigma^*)$ | 5.38                   | 0.00                | 0.47            |

| State    | Character          | Excitation energy [eV] | Orbital overlap |
|----------|--------------------|------------------------|-----------------|
| $T_1$    | $1(\pi, \pi^*)$    | 1.51                   | 0.70            |
| $T_2$    | $2(\pi, \pi^*)$    | 2.87                   | 0.52            |
| $T_3$    | $3(\pi, \pi^*)$    | 3.08                   | 0.51            |
| $T_4$    | $4(\pi, \pi^*)$    | 3.81                   | 0.66            |
| $T_5$    | $1(\pi, \sigma^*)$ | 4.06                   | 0.50            |
| $T_6$    | $2(\pi, \sigma^*)$ | 4.21                   | 0.48            |
| $T_7$    | $1(n, \pi^*)$      | 4.52                   | 0.17            |
| $T_8$    | $1(n, \sigma^*)$   | 4.66                   | 0.56            |
| $T_9$    | $2(n, \sigma^*)$   | 4.86                   | 0.58            |
| $T_{10}$ | $2(n, \pi^*)$      | 4.87                   | 0.21            |

**Table S5b.** Vertical excitation energies [eV] for singlets and triplets of I-BODIPY at TD-DFT/M06-2X-D3/dhf-TZVP level in optimized  $S_1$  geometry

| State    | Character          | Excitation energy [eV] | Oscillator Strength | Orbital overlap |
|----------|--------------------|------------------------|---------------------|-----------------|
| $S_1$    | $1(\pi, \pi^*)$    | 2.72                   | 0.34                | 0.59            |
| $S_2$    | $2(\pi, \pi^*)$    | 3.09                   | 0.34                | 0.56            |
| $S_3$    | $3(\pi, \pi^*)$    | 3.67                   | 0.06                | 0.57            |
| $S_4$    | $1(n, \pi^*)$      | 4.24                   | 0.00                | 0.16            |
| $S_5$    | $1(\pi, \sigma^*)$ | 4.50                   | 0.00                | 0.47            |
| $S_6$    | $2(n, \pi^*)$      | 4.54                   | 0.00                | 0.19            |
| $S_7$    | $1(\pi, \sigma^*)$ | 4.67                   | 0.00                | 0.44            |
| $S_8$    | $4(\pi, \pi^*)$    | 4.73                   | 0.05                | 0.60            |
| $S_9$    | $2(\pi, \sigma^*)$ | 5.32                   | 0.00                | 0.41            |
| $S_{10}$ | $5(\pi, \pi^*)$    | 5.34                   | 0.02                | 0.47            |

| State    | Character          | Excitation energy [eV] | Orbital overlap |
|----------|--------------------|------------------------|-----------------|
| $T_1$    | $1(\pi, \pi^*)$    | 1.52                   | 0.59            |
| $T_2$    | $2(\pi, \pi^*)$    | 2.45                   | 0.57            |
| $T_3$    | $3(\pi, \pi^*)$    | 2.77                   | 0.57            |
| $T_4$    | $4(\pi, \pi^*)$    | 3.55                   | 0.63            |
| $T_5$    | $1(\pi, \sigma^*)$ | 4.12                   | 0.52            |
| $T_6$    | $1(n, \pi^*)$      | 4.23                   | 0.16            |
| $T_7$    | $2(\pi, \sigma^*)$ | 4.30                   | 0.43            |
| $T_8$    | $2(n, \pi^*)$      | 4.52                   | 0.19            |
| $T_9$    | $1(n, \sigma^*)$   | 4.81                   | 0.54            |
| $T_{10}$ | $5(\pi, \pi^*)$    | 4.89                   | 0.56            |

**Table S5c.** Vertical excitation energies [eV] for singlets and triplets of I-BODIPY at TD-DFT/M06-2X-D3/dhf-TZVP level in optimized T<sub>2</sub> geometry

| State           | Character               | Excitation energy [eV] | Oscillator Strength | Orbital overlap |
|-----------------|-------------------------|------------------------|---------------------|-----------------|
| S <sub>1</sub>  | 1( $\pi$ , $\pi^*$ )    | 2.88                   | 0.65                | 0.70            |
| S <sub>2</sub>  | 2( $\pi$ , $\pi^*$ )    | 3.55                   | 0.11                | 0.48            |
| S <sub>3</sub>  | 3( $\pi$ , $\pi^*$ )    | 3.79                   | 0.07                | 0.54            |
| S <sub>4</sub>  | 1( $\pi$ , $\sigma^*$ ) | 4.31                   | 0.00                | 0.39            |
| S <sub>5</sub>  | 2( $\pi$ , $\sigma^*$ ) | 4.48                   | 0.00                | 0.55            |
| S <sub>6</sub>  | 1(n, $\pi^*$ )          | 4.52                   | 0.00                | 0.17            |
| S <sub>7</sub>  | 2(n, $\pi^*$ )          | 4.87                   | 0.00                | 0.20            |
| S <sub>8</sub>  | 4( $\pi$ , $\pi^*$ )    | 4.95                   | 0.02                | 0.56            |
| S <sub>9</sub>  | 1(n, $\sigma^*$ )       | 5.16                   | 0.00                | 0.55            |
| S <sub>10</sub> | 3( $\pi$ , $\sigma^*$ ) | 5.27                   | 0.00                | 0.48            |

| State           | Character               | Excitation energy [eV] | Orbital overlap |
|-----------------|-------------------------|------------------------|-----------------|
| T <sub>1</sub>  | 1( $\pi$ , $\pi^*$ )    | 1.47                   | 0.70            |
| T <sub>2</sub>  | 2( $\pi$ , $\pi^*$ )    | 2.84                   | 0.52            |
| T <sub>3</sub>  | 3( $\pi$ , $\pi^*$ )    | 3.06                   | 0.50            |
| T <sub>4</sub>  | 4( $\pi$ , $\pi^*$ )    | 3.75                   | 0.66            |
| T <sub>5</sub>  | 1( $\pi$ , $\sigma^*$ ) | 3.98                   | 0.50            |
| T <sub>6</sub>  | 2( $\pi$ , $\sigma^*$ ) | 4.12                   | 0.48            |
| T <sub>7</sub>  | 1(n, $\pi^*$ )          | 4.50                   | 0.17            |
| T <sub>8</sub>  | 1(n, $\sigma^*$ )       | 4.57                   | 0.55            |
| T <sub>9</sub>  | 2(n, $\sigma^*$ )       | 4.76                   | 0.59            |
| T <sub>10</sub> | 2(n, $\pi^*$ )          | 4.84                   | 0.20            |

**Table S6a.** Vertical excitation energies [eV] for singlets and triplets of I-BODIPY at TD-DFT(TDA)/B3LYP-D3/dhf-TZVP level in optimized  $S_0$  geometry

| State           | Character               | Excitation energy [eV] | Oscillator Strength | Orbital overlap |
|-----------------|-------------------------|------------------------|---------------------|-----------------|
| S <sub>1</sub>  | 1( $\pi$ , $\pi^*$ )    | 2.90                   | 0.00                | 0.56            |
| S <sub>2</sub>  | 2( $\pi$ , $\pi^*$ )    | 3.24                   | 0.12                | 0.61            |
| S <sub>3</sub>  | 3( $\pi$ , $\pi^*$ )    | 3.50                   | 0.02                | 0.55            |
| S <sub>4</sub>  | 1(n, $\pi^*$ )          | 3.52                   | 0.00                | 0.17            |
| S <sub>5</sub>  | 1( $\pi$ , $\sigma^*$ ) | 3.80                   | 0.00                | 0.35            |
| S <sub>6</sub>  | 2(n, $\pi^*$ )          | 3.92                   | 0.00                | 0.24            |
| S <sub>7</sub>  | 2( $\pi$ , $\sigma^*$ ) | 4.16                   | 0.00                | 0.61            |
| S <sub>8</sub>  | 4( $\pi$ , $\pi^*$ )    | 4.22                   | 0.06                | 0.58            |
| S <sub>9</sub>  | 3( $\pi$ , $\sigma^*$ ) | 4.68                   | 0.00                | 0.40            |
| S <sub>10</sub> | 1(n, $\sigma^*$ )       | 4.89                   | 0.00                | 0.57            |

| State           | Character               | Excitation energy [eV] | Orbital overlap |
|-----------------|-------------------------|------------------------|-----------------|
| T <sub>1</sub>  | 1( $\pi$ , $\pi^*$ )    | 1.63                   | 0.71            |
| T <sub>2</sub>  | 2( $\pi$ , $\pi^*$ )    | 2.47                   | 0.51            |
| T <sub>3</sub>  | 3( $\pi$ , $\pi^*$ )    | 2.69                   | 0.53            |
| T <sub>4</sub>  | 4( $\pi$ , $\pi^*$ )    | 3.44                   | 0.62            |
| T <sub>5</sub>  | 1(n, $\pi^*$ )          | 3.50                   | 0.17            |
| T <sub>6</sub>  | 1( $\pi$ , $\sigma^*$ ) | 3.61                   | 0.40            |
| T <sub>7</sub>  | 2( $\pi$ , $\sigma^*$ ) | 3.75                   | 0.56            |
| T <sub>8</sub>  | 2(n, $\pi^*$ )          | 3.89                   | 0.24            |
| T <sub>9</sub>  | 5( $\pi$ , $\pi^*$ )    | 4.25                   | 0.69            |
| T <sub>10</sub> | 1(n, $\sigma^*$ )       | 4.34                   | 0.56            |

**Table S6b.** Vertical excitation energies [eV] for singlets and triplets of I-BODIPY at TD-DFT(TDA)/B3LYP-D3/dhf-TZVP level in optimized  $S_1$  geometry

| State    | Character          | Excitation energy [eV] | Oscillator Strength | Orbital overlap |
|----------|--------------------|------------------------|---------------------|-----------------|
| $S_1$    | $1(\pi, \pi^*)$    | 2.34                   | 0.03                | 0.60            |
| $S_2$    | $2(\pi, \pi^*)$    | 3.03                   | 0.10                | 0.61            |
| $S_3$    | $1(n, \pi^*)$      | 3.19                   | 0.00                | 0.16            |
| $S_4$    | $3(\pi, \pi^*)$    | 3.39                   | 0.02                | 0.54            |
| $S_5$    | $2(n, \pi^*)$      | 3.58                   | 0.00                | 0.20            |
| $S_6$    | $1(\pi, \sigma^*)$ | 3.99                   | 0.00                | 0.35            |
| $S_7$    | $4(\pi, \pi^*)$    | 4.00                   | 0.08                | 0.62            |
| $S_8$    | $2(\pi, \sigma^*)$ | 4.23                   | 0.00                | 0.53            |
| $S_9$    | $5(\pi, \pi^*)$    | 4.45                   | 0.01                | 0.47            |
| $S_{10}$ | $3(\pi, \sigma^*)$ | 4.67                   | 0.00                | 0.48            |

| State    | Character          | Excitation energy [eV] | Orbital overlap |
|----------|--------------------|------------------------|-----------------|
| $T_1$    | $1(\pi, \pi^*)$    | 1.56                   | 0.60            |
| $T_2$    | $2(\pi, \pi^*)$    | 1.96                   | 0.62            |
| $T_3$    | $3(\pi, \pi^*)$    | 2.52                   | 0.54            |
| $T_4$    | $4(\pi, \pi^*)$    | 3.16                   | 0.63            |
| $T_5$    | $1(n, \pi^*)$      | 3.18                   | 0.16            |
| $T_6$    | $2(n, \pi^*)$      | 3.55                   | 0.20            |
| $T_7$    | $1(\pi, \sigma^*)$ | 3.68                   | 0.45            |
| $T_8$    | $2(\pi, \sigma^*)$ | 3.89                   | 0.45            |
| $T_9$    | $5(\pi, \pi^*)$    | 4.03                   | 0.57            |
| $T_{10}$ | $6(\pi, \pi^*)$    | 4.22                   | 0.59            |

**Table S6c.** Vertical excitation energies [eV] for singlets and triplets of I-BODIPY at TD-DFT(TDA)/B3LYP-D3/dhf-TZVP level in optimized T<sub>2</sub> geometry

| State           | Character            | Excitation energy [eV] | Oscillator Strength | Orbital overlap |
|-----------------|----------------------|------------------------|---------------------|-----------------|
| S <sub>1</sub>  | 1( $\pi, \pi^*$ )    | 2.87                   | 0.00                | 0.56            |
| S <sub>2</sub>  | 2( $\pi, \pi^*$ )    | 3.21                   | 0.12                | 0.61            |
| S <sub>3</sub>  | 3( $\pi, \pi^*$ )    | 3.46                   | 0.02                | 0.56            |
| S <sub>4</sub>  | 1( $n, \pi^*$ )      | 3.50                   | 0.00                | 0.16            |
| S <sub>5</sub>  | 1( $\pi, \sigma^*$ ) | 3.72                   | 0.00                | 0.35            |
| S <sub>6</sub>  | 2( $n, \pi^*$ )      | 3.88                   | 0.00                | 0.22            |
| S <sub>7</sub>  | 2( $\pi, \sigma^*$ ) | 4.08                   | 0.00                | 0.61            |
| S <sub>8</sub>  | 4( $\pi, \pi^*$ )    | 4.17                   | 0.06                | 0.58            |
| S <sub>9</sub>  | 3( $\pi, \sigma^*$ ) | 4.57                   | 0.00                | 0.40            |
| S <sub>10</sub> | 1( $n, \sigma^*$ )   | 4.89                   | 0.00                | 0.57            |

| State           | Character            | Excitation energy [eV] | Orbital overlap |
|-----------------|----------------------|------------------------|-----------------|
| T <sub>1</sub>  | 1( $\pi, \pi^*$ )    | 1.60                   | 0.71            |
| T <sub>2</sub>  | 2( $\pi, \pi^*$ )    | 2.44                   | 0.51            |
| T <sub>3</sub>  | 3( $\pi, \pi^*$ )    | 2.65                   | 0.53            |
| T <sub>4</sub>  | 4( $\pi, \pi^*$ )    | 3.39                   | 0.62            |
| T <sub>5</sub>  | 1( $n, \pi^*$ )      | 3.48                   | 0.16            |
| T <sub>6</sub>  | 1( $\pi, \sigma^*$ ) | 3.53                   | 0.39            |
| T <sub>7</sub>  | 2( $\pi, \sigma^*$ ) | 3.66                   | 0.56            |
| T <sub>8</sub>  | 2( $n, \pi^*$ )      | 3.85                   | 0.22            |
| T <sub>9</sub>  | 5( $\pi, \pi^*$ )    | 4.19                   | 0.69            |
| T <sub>10</sub> | 1( $n, \sigma^*$ )   | 4.26                   | 0.56            |



**Table S7a.** Vertical excitation energies [eV] for singlets and triplets of I-BODIPY at TD-DFT(TDA)/BHLYP-D3/dhf-TZVP level in optimized  $S_0$  geometry

| State           | Character               | Excitation energy [eV] | Oscillator Strength | Orbital overlap |
|-----------------|-------------------------|------------------------|---------------------|-----------------|
| S <sub>1</sub>  | 1( $\pi$ , $\pi^*$ )    | 3.23                   | 0.29                | 0.69            |
| S <sub>2</sub>  | 2( $\pi$ , $\pi^*$ )    | 3.77                   | 0.06                | 0.48            |
| S <sub>3</sub>  | 3( $\pi$ , $\pi^*$ )    | 4.07                   | 0.01                | 0.55            |
| S <sub>4</sub>  | 1( $\pi$ , $\sigma^*$ ) | 4.41                   | 0.00                | 0.38            |
| S <sub>5</sub>  | 2( $\pi$ , $\sigma^*$ ) | 4.59                   | 0.00                | 0.56            |
| S <sub>6</sub>  | 1(n, $\pi^*$ )          | 4.65                   | 0.00                | 0.16            |
| S <sub>7</sub>  | 2(n, $\pi^*$ )          | 5.05                   | 0.00                | 0.20            |
| S <sub>8</sub>  | 4( $\pi$ , $\pi^*$ )    | 5.15                   | 0.02                | 0.57            |
| S <sub>9</sub>  | 1(n, $\sigma^*$ )       | 5.37                   | 0.00                | 0.55            |
| S <sub>10</sub> | 3( $\pi$ , $\sigma^*$ ) | 5.41                   | 0.00                | 0.46            |

| State           | Character               | Excitation energy [eV] | Orbital overlap |
|-----------------|-------------------------|------------------------|-----------------|
| T <sub>1</sub>  | 1( $\pi$ , $\pi^*$ )    | 1.61                   | 0.70            |
| T <sub>2</sub>  | 2( $\pi$ , $\pi^*$ )    | 2.88                   | 0.53            |
| T <sub>3</sub>  | 3( $\pi$ , $\pi^*$ )    | 3.10                   | 0.50            |
| T <sub>4</sub>  | 4( $\pi$ , $\pi^*$ )    | 3.71                   | 0.67            |
| T <sub>5</sub>  | 1( $\pi$ , $\sigma^*$ ) | 3.98                   | 0.50            |
| T <sub>6</sub>  | 2( $\pi$ , $\sigma^*$ ) | 4.13                   | 0.47            |
| T <sub>7</sub>  | 1(n, $\pi^*$ )          | 4.63                   | 0.16            |
| T <sub>8</sub>  | 1(n, $\sigma^*$ )       | 4.64                   | 0.55            |
| T <sub>9</sub>  | 2(n, $\sigma^*$ )       | 4.82                   | 0.58            |
| T <sub>10</sub> | 5( $\pi$ , $\pi^*$ )    | 4.93                   | 0.66            |

**Table S7b.** Vertical excitation energies [eV] for singlets and triplets of I-BODIPY at TD-DFT(TDA)/BHLYP-D3/dhf-TZVP level in optimized  $S_1$  geometry

| State    | Character          | Excitation energy [eV] | Oscillator Strength | Orbital overlap |
|----------|--------------------|------------------------|---------------------|-----------------|
| $S_1$    | $1(\pi, \pi^*)$    | 2.96                   | 0.08                | 0.60            |
| $S_2$    | $2(\pi, \pi^*)$    | 3.33                   | 0.19                | 0.56            |
| $S_3$    | $3(\pi, \pi^*)$    | 3.93                   | 0.02                | 0.58            |
| $S_4$    | $1(n, \pi^*)$      | 4.34                   | 0.00                | 0.15            |
| $S_5$    | $1(\pi, \sigma^*)$ | 4.53                   | 0.00                | 0.48            |
| $S_6$    | $2(\pi, \sigma^*)$ | 4.68                   | 0.00                | 0.43            |
| $S_7$    | $2(n, \pi^*)$      | 4.70                   | 0.00                | 0.18            |
| $S_8$    | $4(\pi, \pi^*)$    | 4.90                   | 0.04                | 0.60            |
| $S_9$    | $3(\pi, \sigma^*)$ | 5.33                   | 0.00                | 0.41            |
| $S_{10}$ | $5(\pi, \pi^*)$    | 5.48                   | 0.01                | 0.48            |

| State    | Character          | Excitation energy [eV] | Orbital overlap |
|----------|--------------------|------------------------|-----------------|
| $T_1$    | $1(\pi, \pi^*)$    | 1.60                   | 0.60            |
| $T_2$    | $2(\pi, \pi^*)$    | 2.50                   | 0.56            |
| $T_3$    | $3(\pi, \pi^*)$    | 2.77                   | 0.57            |
| $T_4$    | $4(\pi, \pi^*)$    | 3.46                   | 0.63            |
| $T_5$    | $1(\pi, \sigma^*)$ | 4.03                   | 0.52            |
| $T_6$    | $2(\pi, \sigma^*)$ | 4.20                   | 0.43            |
| $T_7$    | $1(n, \pi^*)$      | 4.32                   | 0.15            |
| $T_8$    | $2(n, \pi^*)$      | 4.66                   | 0.18            |
| $T_9$    | $1(n, \sigma^*)$   | 4.78                   | 0.53            |
| $T_{10}$ | $5(\pi, \pi^*)$    | 4.80                   | 0.57            |

**Table S7c.** Vertical excitation energies [eV] for singlets and triplets of I-BODIPY at TD-DFT(TDA)/BHLYP-D3/dhf-TZVP level in optimized T<sub>2</sub> geometry

| State           | Character               | Excitation energy [eV] | Oscillator Strength | Orbital overlap |
|-----------------|-------------------------|------------------------|---------------------|-----------------|
| S <sub>1</sub>  | 1( $\pi$ , $\pi^*$ )    | 3.20                   | 0.29                | 0.69            |
| S <sub>2</sub>  | 2( $\pi$ , $\pi^*$ )    | 3.75                   | 0.06                | 0.48            |
| S <sub>3</sub>  | 3( $\pi$ , $\pi^*$ )    | 4.04                   | 0.01                | 0.55            |
| S <sub>4</sub>  | 1( $\pi$ , $\sigma^*$ ) | 4.33                   | 0.00                | 0.38            |
| S <sub>5</sub>  | 2( $\pi$ , $\sigma^*$ ) | 4.51                   | 0.00                | 0.56            |
| S <sub>6</sub>  | 1(n, $\pi^*$ )          | 4.63                   | 0.00                | 0.16            |
| S <sub>7</sub>  | 2(n, $\pi^*$ )          | 5.02                   | 0.00                | 0.20            |
| S <sub>8</sub>  | 4( $\pi$ , $\pi^*$ )    | 5.11                   | 0.02                | 0.56            |
| S <sub>9</sub>  | 1(n, $\sigma^*$ )       | 5.28                   | 0.00                | 0.55            |
| S <sub>10</sub> | 3( $\pi$ , $\sigma^*$ ) | 5.31                   | 0.00                | 0.47            |

| State           | Character               | Excitation energy [eV] | Orbital overlap |
|-----------------|-------------------------|------------------------|-----------------|
| T <sub>1</sub>  | 1( $\pi$ , $\pi^*$ )    | 1.58                   | 0.70            |
| T <sub>2</sub>  | 2( $\pi$ , $\pi^*$ )    | 2.84                   | 0.53            |
| T <sub>3</sub>  | 3( $\pi$ , $\pi^*$ )    | 3.07                   | 0.50            |
| T <sub>4</sub>  | 4( $\pi$ , $\pi^*$ )    | 3.65                   | 0.67            |
| T <sub>5</sub>  | 1( $\pi$ , $\sigma^*$ ) | 3.90                   | 0.50            |
| T <sub>6</sub>  | 2( $\pi$ , $\sigma^*$ ) | 4.04                   | 0.47            |
| T <sub>7</sub>  | 1(n, $\sigma^*$ )       | 4.55                   | 0.55            |
| T <sub>8</sub>  | 1(n, $\pi^*$ )          | 4.61                   | 0.16            |
| T <sub>9</sub>  | 2(n, $\sigma^*$ )       | 4.73                   | 0.58            |
| T <sub>10</sub> | 5( $\pi$ , $\pi^*$ )    | 4.87                   | 0.66            |

**Table S8a.** Vertical excitation energies [eV] for singlets and triplets of I-BODIPY at sf-X2C-TD-DFT/B3LYP-D3/x2c-TZVPPall level in optimized  $S_0$  geometry

| State    | Character          | Excitation energy [eV] | Oscillator Strength |
|----------|--------------------|------------------------|---------------------|
| $S_1$    | $1(\pi, \pi^*)$    | 2.74                   | 0.30                |
| $S_2$    | $2(\pi, \pi^*)$    | 2.99                   | 0.38                |
| $S_3$    | $3(\pi, \pi^*)$    | 3.36                   | 0.08                |
| $S_4$    | $1(n, \pi^*)$      | 3.50                   | 0.00                |
| $S_5$    | $1(\pi, \sigma^*)$ | 3.89                   | 0.00                |
| $S_6$    | $2(n, \pi^*)$      | 3.90                   | 0.00                |
| $S_7$    | $4(\pi, \pi^*)$    | 4.10                   | 0.06                |
| $S_8$    | $2(\pi, \sigma^*)$ | 4.21                   | 0.00                |
| $S_9$    | $3(\pi, \sigma^*)$ | 4.81                   | 0.01                |
| $S_{10}$ | $1(n, \sigma^*)$   | 4.87                   | 0.00                |

| State    | Character          | Excitation energy [eV] |
|----------|--------------------|------------------------|
| $T_1$    | $1(\pi, \pi^*)$    | 1.51                   |
| $T_2$    | $2(\pi, \pi^*)$    | 2.40                   |
| $T_3$    | $3(\pi, \pi^*)$    | 2.59                   |
| $T_4$    | $4(\pi, \pi^*)$    | 3.33                   |
| $T_5$    | $1(n, \pi^*)$      | 3.48                   |
| $T_6$    | $1(\pi, \sigma^*)$ | 3.67                   |
| $T_7$    | $2(\pi, \sigma^*)$ | 3.80                   |
| $T_8$    | $2(n, \pi^*)$      | 3.87                   |
| $T_9$    | $5(\pi, \pi^*)$    | 4.19                   |
| $T_{10}$ | $1(n, \sigma^*)$   | 4.37                   |

**Table S8b.** Vertical excitation energies [eV] for singlets and triplets of I-BODIPY at sf-X2C-S-TD-DFT/B3LYP-D3/x2c-TZVPPall level at the optimized S<sub>1</sub> geometry

| State           | Character               | Excitation energy [eV] | Oscillator Strength |
|-----------------|-------------------------|------------------------|---------------------|
| S <sub>1</sub>  | 1( $\pi$ , $\pi^*$ )    | 2.23                   | 0.06                |
| S <sub>2</sub>  | 2( $\pi$ , $\pi^*$ )    | 2.77                   | 0.54                |
| S <sub>3</sub>  | 1(n, $\pi^*$ )          | 3.17                   | 0.00                |
| S <sub>4</sub>  | 3( $\pi$ , $\pi^*$ )    | 3.26                   | 0.04                |
| S <sub>5</sub>  | 2(n, $\pi^*$ )          | 3.57                   | 0.00                |
| S <sub>6</sub>  | 4( $\pi$ , $\pi^*$ )    | 3.87                   | 0.09                |
| S <sub>7</sub>  | 1( $\pi$ , $\sigma^*$ ) | 4.31                   | 0.00                |
| S <sub>8</sub>  | 2( $\pi$ , $\sigma^*$ ) | 4.39                   | 0.00                |
| S <sub>9</sub>  | 5( $\pi$ , $\pi^*$ )    | 4.78                   | 0.02                |
| S <sub>10</sub> | 1( $\pi$ , $\sigma^*$ ) | 4.95                   | 0.00                |

| State           | Character               | Excitation energy [eV] |
|-----------------|-------------------------|------------------------|
| T <sub>1</sub>  | 1( $\pi$ , $\pi^*$ )    | 1.44                   |
| T <sub>2</sub>  | 2( $\pi$ , $\pi^*$ )    | 1.87                   |
| T <sub>3</sub>  | 3( $\pi$ , $\pi^*$ )    | 2.41                   |
| T <sub>4</sub>  | 4( $\pi$ , $\pi^*$ )    | 3.03                   |
| T <sub>5</sub>  | 1(n, $\pi^*$ )          | 3.15                   |
| T <sub>6</sub>  | 2(n, $\pi^*$ )          | 3.52                   |
| T <sub>7</sub>  | 1( $\pi$ , $\sigma^*$ ) | 3.73                   |
| T <sub>8</sub>  | 2( $\pi$ , $\sigma^*$ ) | 3.96                   |
| T <sub>9</sub>  | 5( $\pi$ , $\pi^*$ )    | 3.98                   |
| T <sub>10</sub> | 6( $\pi$ , $\pi^*$ )    | 4.17                   |

**Table S8c.** Vertical excitation energies [eV] for singlets and triplets of I-BODIPY at sf-X2C-S-TD-DFT/B3LYP-D3/x2c-TZVPPall level in optimized T<sub>2</sub> geometry

| State           | Character               | Excitation energy [eV] | Oscillator Strength |
|-----------------|-------------------------|------------------------|---------------------|
| S <sub>1</sub>  | 1( $\pi$ , $\pi^*$ )    | 2.71                   | 0.31                |
| S <sub>2</sub>  | 2( $\pi$ , $\pi^*$ )    | 2.97                   | 0.37                |
| S <sub>3</sub>  | 3( $\pi$ , $\pi^*$ )    | 3.32                   | 0.08                |
| S <sub>4</sub>  | 1(n, $\pi^*$ )          | 3.48                   | 0.00                |
| S <sub>5</sub>  | 1( $\pi$ , $\sigma^*$ ) | 3.80                   | 0.00                |
| S <sub>6</sub>  | 2(n, $\pi^*$ )          | 3.86                   | 0.00                |
| S <sub>7</sub>  | 2( $\pi$ , $\sigma^*$ ) | 4.05                   | 0.05                |
| S <sub>8</sub>  | 4( $\pi$ , $\pi^*$ )    | 4.13                   | 0.00                |
| S <sub>9</sub>  | 3( $\pi$ , $\sigma^*$ ) | 4.70                   | 0.00                |
| S <sub>10</sub> | 1(n, $\sigma^*$ )       | 4.80                   | 0.01                |

| State           | Character               | Excitation energy [eV] |
|-----------------|-------------------------|------------------------|
| T <sub>1</sub>  | 1( $\pi$ , $\pi^*$ )    | 1.47                   |
| T <sub>2</sub>  | 2( $\pi$ , $\pi^*$ )    | 2.35                   |
| T <sub>3</sub>  | 3( $\pi$ , $\pi^*$ )    | 2.56                   |
| T <sub>4</sub>  | 4( $\pi$ , $\pi^*$ )    | 3.27                   |
| T <sub>5</sub>  | 1(n, $\pi^*$ )          | 3.46                   |
| T <sub>6</sub>  | 1( $\pi$ , $\sigma^*$ ) | 3.58                   |
| T <sub>7</sub>  | 2( $\pi$ , $\sigma^*$ ) | 3.71                   |
| T <sub>8</sub>  | 2(n, $\pi^*$ )          | 3.83                   |
| T <sub>9</sub>  | 5( $\pi$ , $\pi^*$ )    | 4.13                   |
| T <sub>10</sub> | 1(n, $\sigma^*$ )       | 4.29                   |

**Table S9a.** Vertical excitation energies [eV] for singlets and triplets of I-BODIPY at sf-X2C-TD-DFT(TDA)/BHLYP-D3/x2c-TZVPPall level in optimized  $S_0$  geometry

| State           | Character               | Excitation energy [eV] | Oscillator Strength |
|-----------------|-------------------------|------------------------|---------------------|
| S <sub>1</sub>  | 1( $\pi$ , $\pi^*$ )    | 3.23                   | 0.98                |
| S <sub>2</sub>  | 2( $\pi$ , $\pi^*$ )    | 3.77                   | 0.21                |
| S <sub>3</sub>  | 3( $\pi$ , $\pi^*$ )    | 4.07                   | 0.12                |
| S <sub>4</sub>  | 1( $\pi$ , $\sigma^*$ ) | 4.51                   | 0.00                |
| S <sub>5</sub>  | 2( $\pi$ , $\sigma^*$ ) | 4.64                   | 0.00                |
| S <sub>6</sub>  | 1(n, $\pi^*$ )          | 4.69                   | 0.00                |
| S <sub>7</sub>  | 2(n, $\pi^*$ )          | 5.04                   | 0.00                |
| S <sub>8</sub>  | 4( $\pi$ , $\pi^*$ )    | 5.15                   | 0.05                |
| S <sub>9</sub>  | 1(n, $\sigma^*$ )       | 5.47                   | 0.00                |
| S <sub>10</sub> | 3( $\pi$ , $\sigma^*$ ) | 5.55                   | 0.00                |

| State           | Character               | Excitation energy [eV] |
|-----------------|-------------------------|------------------------|
| T <sub>1</sub>  | 1( $\pi$ , $\pi^*$ )    | 1.61                   |
| T <sub>2</sub>  | 2( $\pi$ , $\pi^*$ )    | 2.88                   |
| T <sub>3</sub>  | 3( $\pi$ , $\pi^*$ )    | 3.09                   |
| T <sub>4</sub>  | 4( $\pi$ , $\pi^*$ )    | 3.70                   |
| T <sub>5</sub>  | 1( $\pi$ , $\sigma^*$ ) | 4.05                   |
| T <sub>6</sub>  | 2( $\pi$ , $\sigma^*$ ) | 4.21                   |
| T <sub>7</sub>  | 1(n, $\pi^*$ )          | 4.62                   |
| T <sub>8</sub>  | 1(n, $\sigma^*$ )       | 4.71                   |
| T <sub>9</sub>  | 2(n, $\sigma^*$ )       | 4.89                   |
| T <sub>10</sub> | 5( $\pi$ , $\pi^*$ )    | 4.93                   |

**Table S9b.** Vertical excitation energies [eV] for singlets and triplets of I-BODIPY at sf-X2C-TD-DFT(TDA)/BHLYP-D3/x2c-TZVPPall level in optimized S<sub>1</sub> geometry

| State           | Character               | Excitation energy [eV] | Oscillator Strength |
|-----------------|-------------------------|------------------------|---------------------|
| S <sub>1</sub>  | 1( $\pi$ , $\pi^*$ )    | 2.95                   | 0.36                |
| S <sub>2</sub>  | 2( $\pi$ , $\pi^*$ )    | 3.33                   | 0.68                |
| S <sub>3</sub>  | 3( $\pi$ , $\pi^*$ )    | 3.93                   | 0.09                |
| S <sub>4</sub>  | 1(n, $\pi^*$ )          | 4.33                   | 0.00                |
| S <sub>5</sub>  | 1( $\pi$ , $\sigma^*$ ) | 4.64                   | 0.00                |
| S <sub>6</sub>  | 2( $\pi$ , $\sigma^*$ ) | 4.68                   | 0.00                |
| S <sub>7</sub>  | 2(n, $\pi^*$ )          | 4.79                   | 0.00                |
| S <sub>8</sub>  | 4( $\pi$ , $\pi^*$ )    | 4.88                   | 0.10                |
| S <sub>9</sub>  | 3( $\pi$ , $\sigma^*$ ) | 5.47                   | 0.02                |
| S <sub>10</sub> | 5( $\pi$ , $\pi^*$ )    | 5.48                   | 0.01                |

| State           | Character               | Excitation energy [eV] |
|-----------------|-------------------------|------------------------|
| T <sub>1</sub>  | 1( $\pi$ , $\pi^*$ )    | 1.61                   |
| T <sub>2</sub>  | 2( $\pi$ , $\pi^*$ )    | 2.49                   |
| T <sub>3</sub>  | 3( $\pi$ , $\pi^*$ )    | 2.77                   |
| T <sub>4</sub>  | 4( $\pi$ , $\pi^*$ )    | 3.46                   |
| T <sub>5</sub>  | 1( $\pi$ , $\sigma^*$ ) | 4.10                   |
| T <sub>6</sub>  | 2( $\pi$ , $\sigma^*$ ) | 4.29                   |
| T <sub>7</sub>  | 1(n, $\pi^*$ )          | 4.31                   |
| T <sub>8</sub>  | 2(n, $\pi^*$ )          | 4.64                   |
| T <sub>9</sub>  | 1(n, $\sigma^*$ )       | 4.80                   |
| T <sub>10</sub> | 5( $\pi$ , $\pi^*$ )    | 4.85                   |



**Table S9c.** Vertical excitation energies [eV] for singlets and triplets of I-BODIPY at TD-DFT(TDA)/BHLYP-D3/x2c-TZVPPall level in optimized T<sub>2</sub> geometry

| State           | Character            | Excitation energy [eV] | Oscillator Strength |
|-----------------|----------------------|------------------------|---------------------|
| S <sub>1</sub>  | 1( $\pi, \pi^*$ )    | 3.20                   | 0.98                |
| S <sub>2</sub>  | 2( $\pi, \pi^*$ )    | 3.74                   | 0.22                |
| S <sub>3</sub>  | 3( $\pi, \pi^*$ )    | 4.04                   | 0.12                |
| S <sub>4</sub>  | 1( $\pi, \sigma^*$ ) | 4.43                   | 0.00                |
| S <sub>5</sub>  | 2( $\pi, \sigma^*$ ) | 4.60                   | 0.00                |
| S <sub>6</sub>  | 1(n, $\pi^*$ )       | 4.62                   | 0.00                |
| S <sub>7</sub>  | 2(n, $\pi^*$ )       | 5.00                   | 0.00                |
| S <sub>8</sub>  | 4( $\pi, \pi^*$ )    | 5.10                   | 0.05                |
| S <sub>9</sub>  | 1(n, $\sigma^*$ )    | 5.38                   | 0.00                |
| S <sub>10</sub> | 3( $\pi, \sigma^*$ ) | 5.44                   | 0.00                |

| State           | Character            | Excitation energy [eV] |
|-----------------|----------------------|------------------------|
| T <sub>1</sub>  | 1( $\pi, \pi^*$ )    | 1.58                   |
| T <sub>2</sub>  | 2( $\pi, \pi^*$ )    | 2.84                   |
| T <sub>3</sub>  | 3( $\pi, \pi^*$ )    | 3.06                   |
| T <sub>4</sub>  | 4( $\pi, \pi^*$ )    | 3.65                   |
| T <sub>5</sub>  | 1( $\pi, \sigma^*$ ) | 3.97                   |
| T <sub>6</sub>  | 2( $\pi, \sigma^*$ ) | 4.12                   |
| T <sub>7</sub>  | 1(n, $\sigma^*$ )    | 4.60                   |
| T <sub>8</sub>  | 1(n, $\pi^*$ )       | 4.62                   |
| T <sub>9</sub>  | 2(n, $\sigma^*$ )    | 4.79                   |
| T <sub>10</sub> | 5( $\pi, \pi^*$ )    | 4.87                   |

**Table S10a.** Vertical excitation energies [eV] for singlets and triplets of I-BODIPY at sf-X2C-S-TD-DFT/M06-2X/x2c-TZVPPall level in optimized  $S_0$  geometry

| State           | Character               | Excitation energy [eV] | Oscillator Strength |
|-----------------|-------------------------|------------------------|---------------------|
| S <sub>1</sub>  | 1( $\pi$ , $\pi^*$ )    | 2.88                   | 0.67                |
| S <sub>2</sub>  | 2( $\pi$ , $\pi^*$ )    | 3.53                   | 0.11                |
| S <sub>3</sub>  | 3( $\pi$ , $\pi^*$ )    | 3.80                   | 0.07                |
| S <sub>4</sub>  | 1( $\pi$ , $\sigma^*$ ) | 4.38                   | 0.00                |
| S <sub>5</sub>  | 1(n, $\pi^*$ )          | 4.49                   | 0.00                |
| S <sub>6</sub>  | 2( $\pi$ , $\sigma^*$ ) | 4.54                   | 0.00                |
| S <sub>7</sub>  | 2(n, $\pi^*$ )          | 4.82                   | 0.00                |
| S <sub>8</sub>  | 4( $\pi$ , $\pi^*$ )    | 4.96                   | 0.02                |
| S <sub>9</sub>  | 1(n, $\sigma^*$ )       | 5.22                   | 0.00                |
| S <sub>10</sub> | 3( $\pi$ , $\sigma^*$ ) | 5.52                   | 0.00                |

| State           | Character               | Excitation energy [eV] |
|-----------------|-------------------------|------------------------|
| T <sub>1</sub>  | 1( $\pi$ , $\pi^*$ )    | 1.49                   |
| T <sub>2</sub>  | 2( $\pi$ , $\pi^*$ )    | 2.85                   |
| T <sub>3</sub>  | 3( $\pi$ , $\pi^*$ )    | 3.05                   |
| T <sub>4</sub>  | 4( $\pi$ , $\pi^*$ )    | 3.78                   |
| T <sub>5</sub>  | 1( $\pi$ , $\sigma^*$ ) | 4.01                   |
| T <sub>6</sub>  | 2( $\pi$ , $\sigma^*$ ) | 4.19                   |
| T <sub>7</sub>  | 1(n, $\pi^*$ )          | 4.47                   |
| T <sub>8</sub>  | 1(n, $\sigma^*$ )       | 4.79                   |
| T <sub>9</sub>  | 2(n, $\sigma^*$ )       | 4.80                   |
| T <sub>10</sub> | 2(n, $\pi^*$ )          | 5.02                   |

**Table S10b.** Vertical excitation energies [eV] for singlets and triplets of I-BODIPY at sf-X2C-S-TD-DFT/M06-2X/x2c-TZVPPall level in optimized S<sub>1</sub> geometry

| State           | Character               | Excitation energy [eV] | Oscillator Strength |
|-----------------|-------------------------|------------------------|---------------------|
| S <sub>1</sub>  | 1( $\pi$ , $\pi^*$ )    | 2.68                   | 0.34                |
| S <sub>2</sub>  | 2( $\pi$ , $\pi^*$ )    | 3.05                   | 0.35                |
| S <sub>3</sub>  | 3( $\pi$ , $\pi^*$ )    | 3.63                   | 0.06                |
| S <sub>4</sub>  | 1(n, $\pi^*$ )          | 4.20                   | 0.00                |
| S <sub>5</sub>  | 1( $\pi$ , $\sigma^*$ ) | 4.46                   | 0.00                |
| S <sub>6</sub>  | 2(n, $\pi^*$ )          | 4.47                   | 0.00                |
| S <sub>7</sub>  | 1( $\pi$ , $\sigma^*$ ) | 4.67                   | 0.00                |
| S <sub>8</sub>  | 4( $\pi$ , $\pi^*$ )    | 4.69                   | 0.05                |
| S <sub>9</sub>  | 2( $\pi$ , $\sigma^*$ ) | 5.31                   | 0.01                |
| S <sub>10</sub> | 5( $\pi$ , $\pi^*$ )    | 5.38                   | 0.00                |

| State           | Character               | Excitation energy [eV] |
|-----------------|-------------------------|------------------------|
| T <sub>1</sub>  | 1( $\pi$ , $\pi^*$ )    | 1.49                   |
| T <sub>2</sub>  | 2( $\pi$ , $\pi^*$ )    | 2.42                   |
| T <sub>3</sub>  | 3( $\pi$ , $\pi^*$ )    | 2.74                   |
| T <sub>4</sub>  | 4( $\pi$ , $\pi^*$ )    | 3.52                   |
| T <sub>5</sub>  | 1( $\pi$ , $\sigma^*$ ) | 4.07                   |
| T <sub>6</sub>  | 1(n, $\pi^*$ )          | 4.18                   |
| T <sub>7</sub>  | 2( $\pi$ , $\sigma^*$ ) | 4.28                   |
| T <sub>8</sub>  | 2(n, $\pi^*$ )          | 4.44                   |
| T <sub>9</sub>  | 1(n, $\sigma^*$ )       | 4.76                   |
| T <sub>10</sub> | 5( $\pi$ , $\pi^*$ )    | 4.85                   |

**Table S10c.** Vertical excitation energies [eV] for singlets and triplets of I-BODIPY at sf-X2C-S-TD-DFT/M06-2X/x2c-TZVPPall level in optimized T<sub>2</sub> geometry

| State           | Character               | Excitation energy [eV] | Oscillator Strength |
|-----------------|-------------------------|------------------------|---------------------|
| S <sub>1</sub>  | 1( $\pi$ , $\pi^*$ )    | 2.84                   | 0.66                |
| S <sub>2</sub>  | 2( $\pi$ , $\pi^*$ )    | 3.51                   | 0.12                |
| S <sub>3</sub>  | 3( $\pi$ , $\pi^*$ )    | 3.76                   | 0.07                |
| S <sub>4</sub>  | 1( $\pi$ , $\sigma^*$ ) | 4.29                   | 0.00                |
| S <sub>5</sub>  | 2( $\pi$ , $\sigma^*$ ) | 4.45                   | 0.00                |
| S <sub>6</sub>  | 1(n, $\pi^*$ )          | 4.47                   | 0.00                |
| S <sub>7</sub>  | 2(n, $\pi^*$ )          | 4.80                   | 0.00                |
| S <sub>8</sub>  | 4( $\pi$ , $\pi^*$ )    | 4.91                   | 0.02                |
| S <sub>9</sub>  | 1(n, $\sigma^*$ )       | 5.14                   | 0.00                |
| S <sub>10</sub> | 3( $\pi$ , $\sigma^*$ ) | 5.30                   | 0.00                |

| State           | Character               | Excitation energy [eV] |
|-----------------|-------------------------|------------------------|
| T <sub>1</sub>  | 1( $\pi$ , $\pi^*$ )    | 1.46                   |
| T <sub>2</sub>  | 2( $\pi$ , $\pi^*$ )    | 2.81                   |
| T <sub>3</sub>  | 3( $\pi$ , $\pi^*$ )    | 3.02                   |
| T <sub>4</sub>  | 4( $\pi$ , $\pi^*$ )    | 3.73                   |
| T <sub>5</sub>  | 1( $\pi$ , $\sigma^*$ ) | 3.93                   |
| T <sub>6</sub>  | 2( $\pi$ , $\sigma^*$ ) | 4.09                   |
| T <sub>7</sub>  | 1(n, $\pi^*$ )          | 4.45                   |
| T <sub>8</sub>  | 1(n, $\sigma^*$ )       | 4.51                   |
| T <sub>9</sub>  | 2(n, $\sigma^*$ )       | 4.70                   |
| T <sub>10</sub> | 2(n, $\pi^*$ )          | 4.77                   |

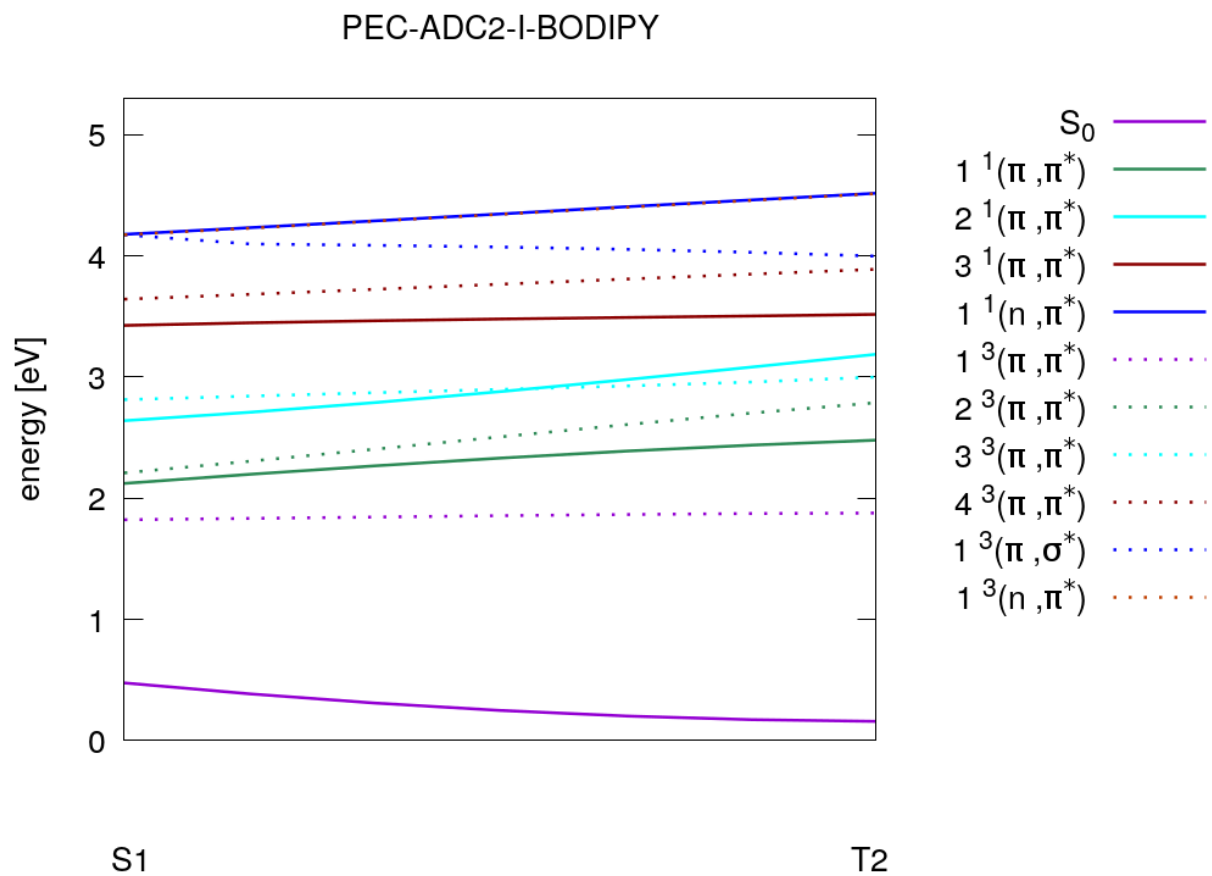

**Figure S1.** Relative electronic energies for I-BODPY at the ADC(2)/dhf-TZVP level along the PEC with respect to the  $S_0$  energy at  $S_0$  optimized geometry.



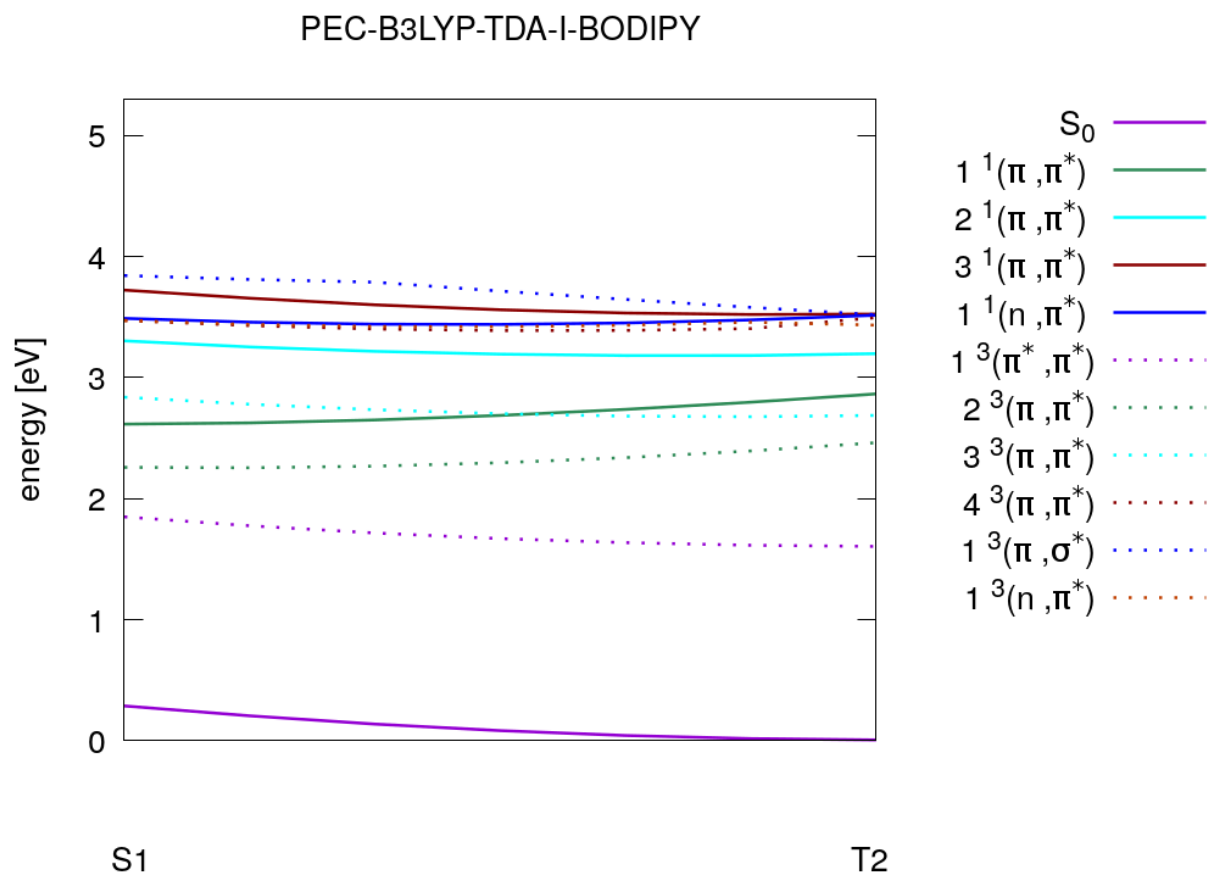

**Figure S3.** Relative electronic energies for I-BODPY at the TD-DFT(TDA)/B3LYP/dhf-TZVP level along the PEC with respect to the  $S_0$  energy at  $S_0$  optimized geometry.

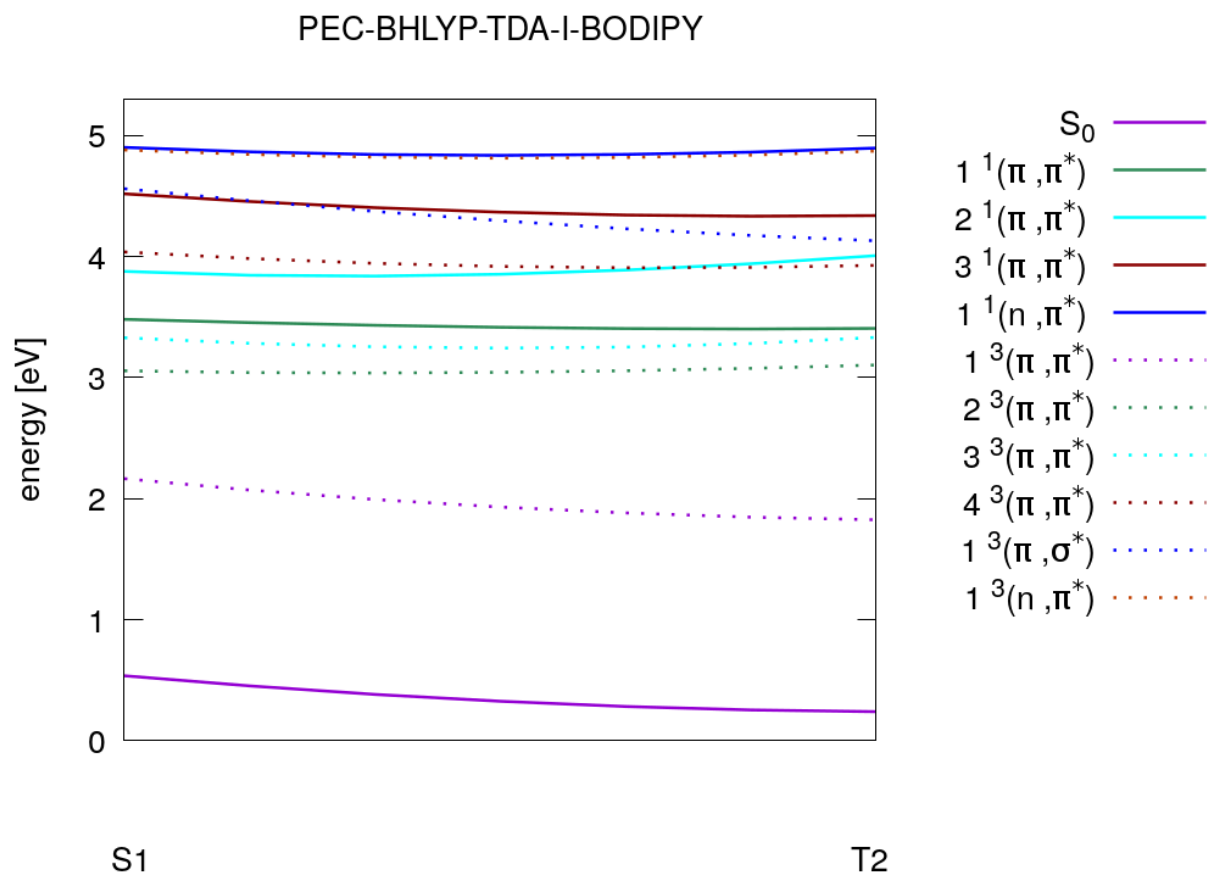

**Figure S4.** Relative electronic energies for I-BODPY at the TD-DFT(TDA)/BHLYP/dhf-TZVP level along the PEC with respect to the  $S_0$  energy at  $S_0$  optimized geometry.



**Table S11.** Non-parallelities [eV] between ADC(2) —TD-DFT/B3LYP and ADC(2)—TD-DFT(TDA)/BHLYP for I-BODIPY along the PEC.

| State                | ADC(2) and TD-DFT/B3LYP | ADC(2) and TD-DFT(TDA)/BHLYP |
|----------------------|-------------------------|------------------------------|
| $S_0$                | 0.04                    | 0.02                         |
| $1^1(\pi, \pi^*)$    | 0.19                    | 0.43                         |
| $2^1(\pi, \pi^*)$    | 0.36                    | 0.42                         |
| $3^1(\pi, \pi^*)$    | 0.16                    | 0.27                         |
| $1^1(n, \pi^*)$      | 0.31                    | 0.35                         |
| $1^3(\pi, \pi^*)$    | 0.32                    | 0.33                         |
| $2^3(\pi, \pi^*)$    | 0.38                    | 0.53                         |
| $3^3(\pi, \pi^*)$    | 0.32                    | 0.19                         |
| $4^3(\pi, \pi^*)$    | 0.28                    | 0.36                         |
| $1^3(n, \pi^*)$      | 0.26                    | 0.25                         |
| $1^3(\pi, \sigma^*)$ | 0.27                    | 0.35                         |

**Table S12.** Shapes and energies [eV] of frontier molecular orbitals of I-BODIPY at DFT/B3LYP/dhf-TZVP level of theory

|                                                                                     |                                                                                      |
|-------------------------------------------------------------------------------------|--------------------------------------------------------------------------------------|
| 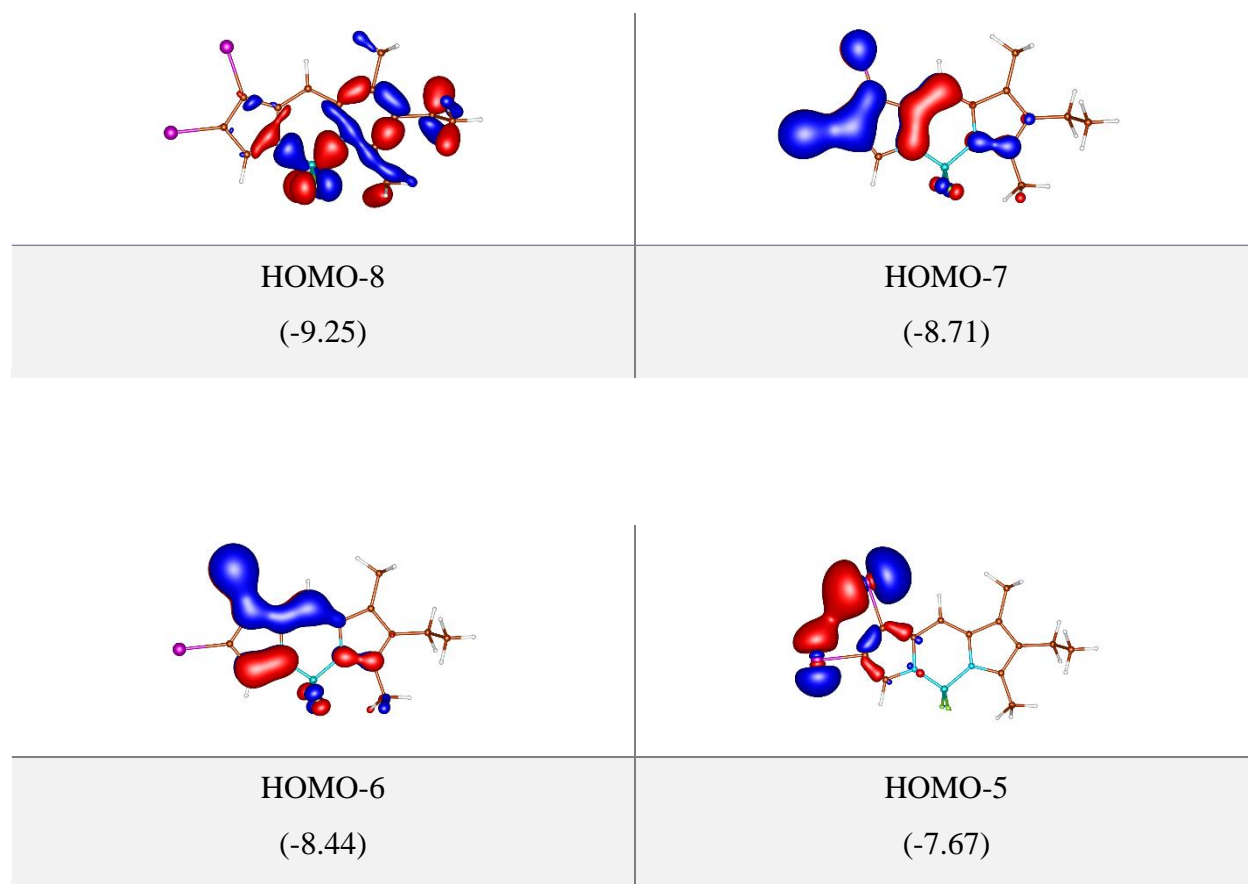   | 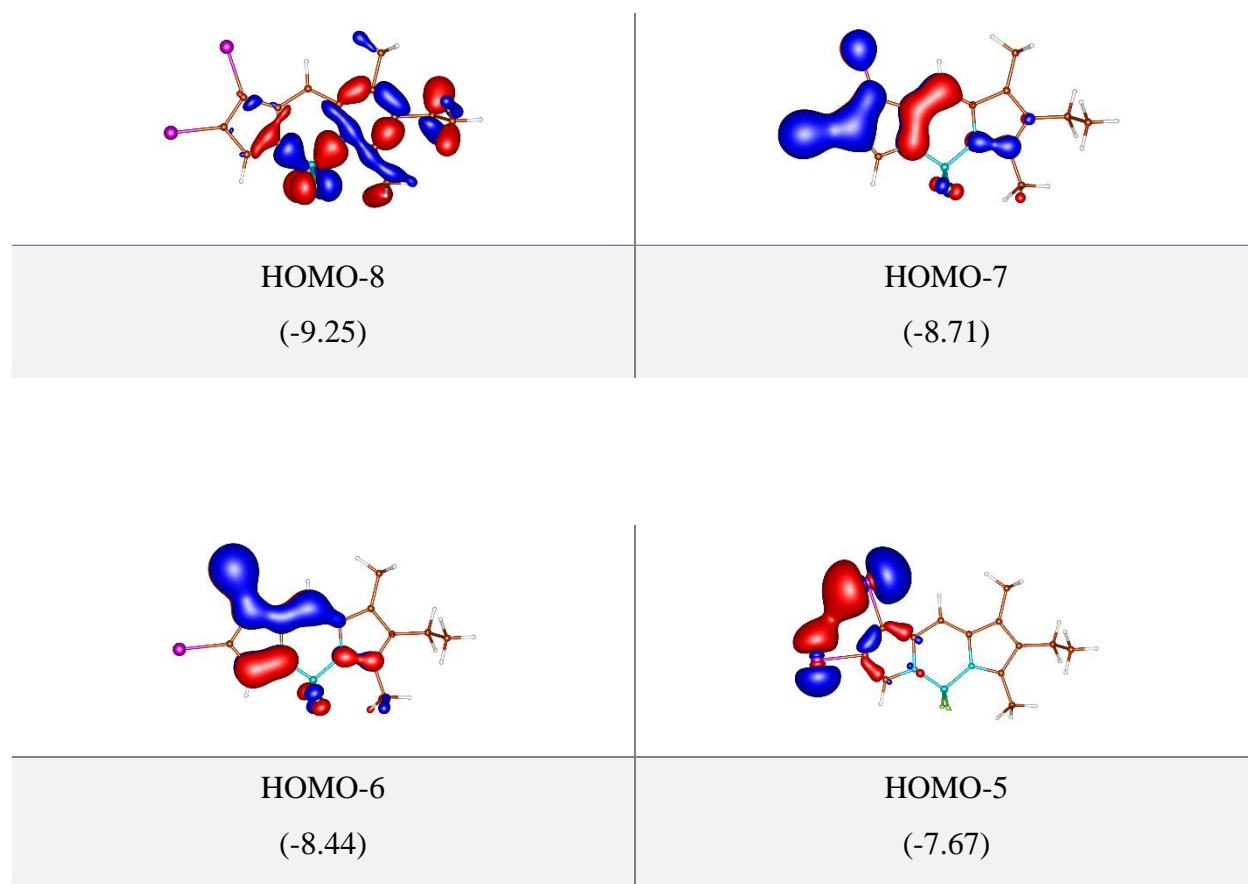   |
| <p>HOMO-8<br/>(-9.25)</p>                                                           | <p>HOMO-7<br/>(-8.71)</p>                                                            |
| 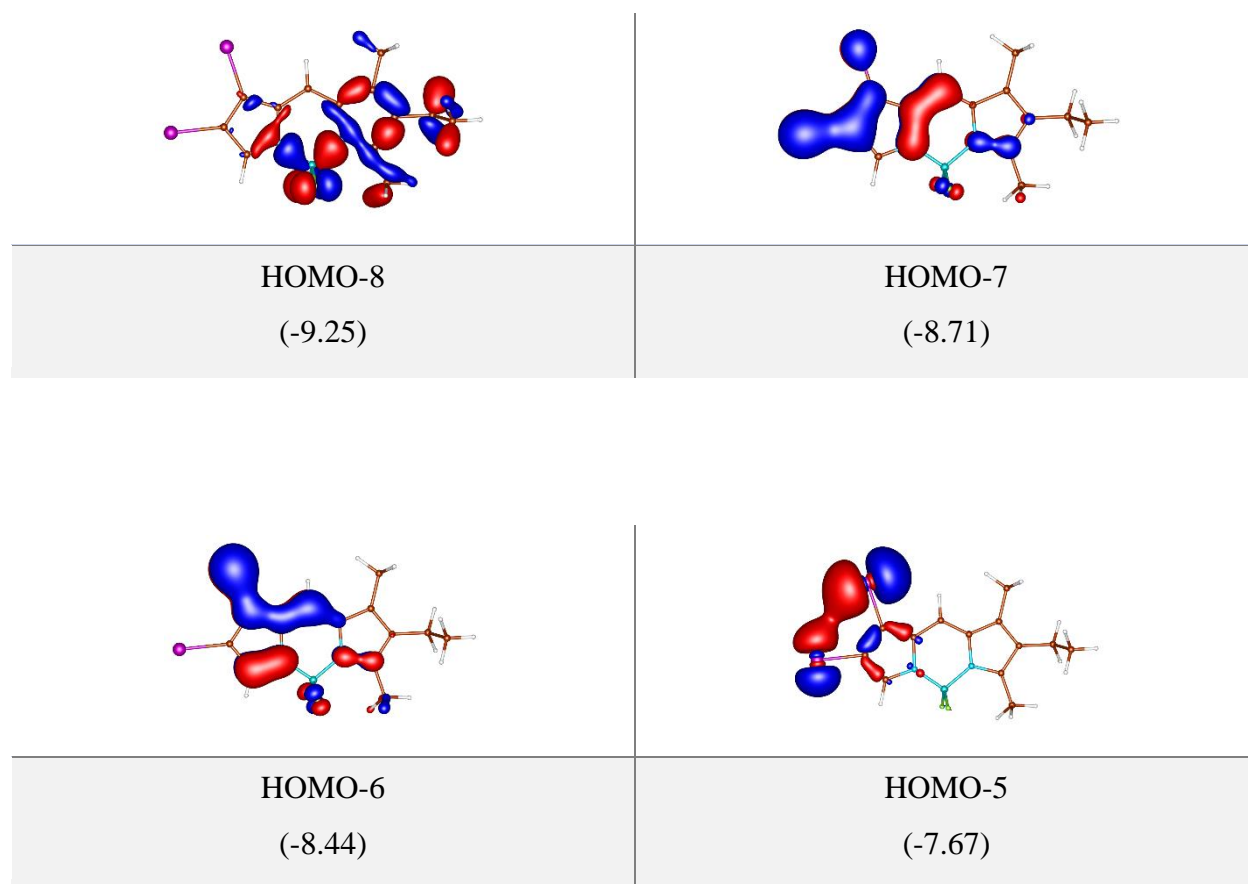 | 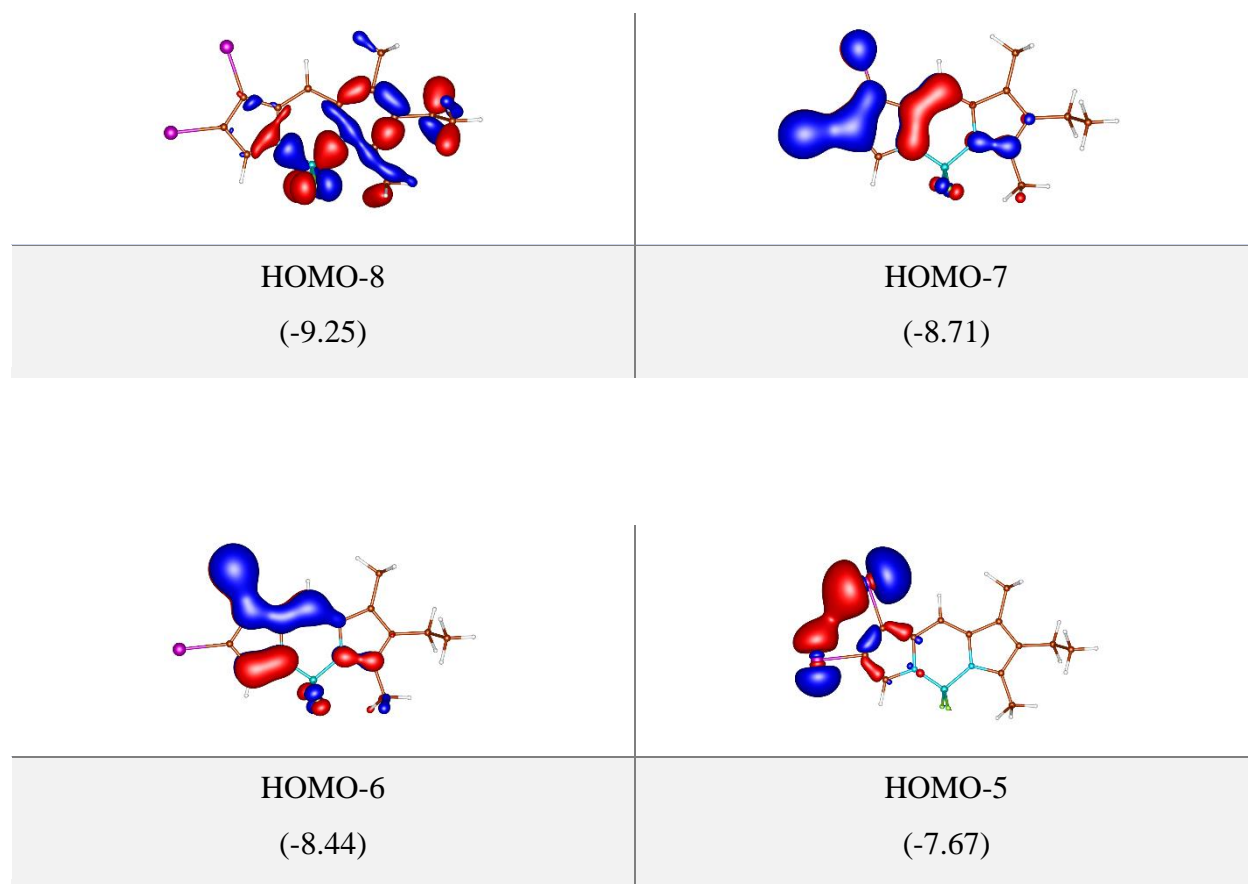 |
| <p>HOMO-6<br/>(-8.44)</p>                                                           | <p>HOMO-5<br/>(-7.67)</p>                                                            |

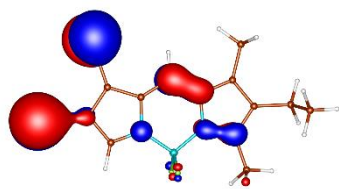

HOMO-4  
(-7.65)

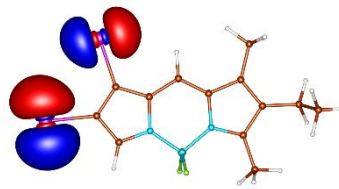

HOMO-3  
(-7.20)

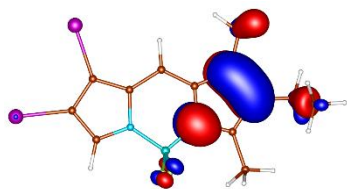

HOMO-2  
(-7.07)

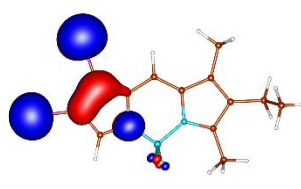

HOMO-1  
(-6.53)

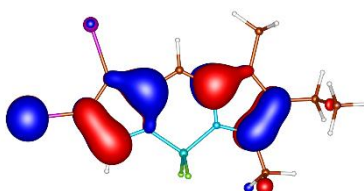

HOMO  
(-5.98)

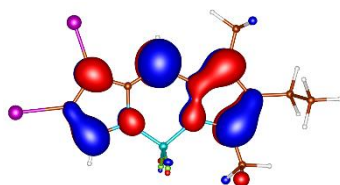

LUMO  
(-3.07)

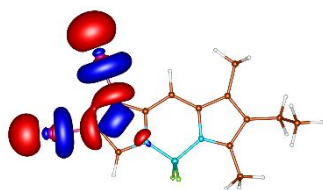

LUMO+1  
(-1.38)

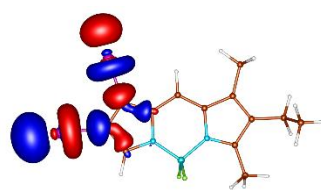

LUMO+2  
(-0.55)

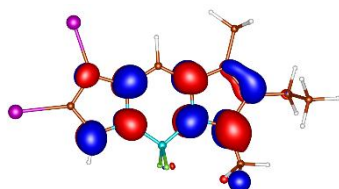

LUMO+3  
(0.23)

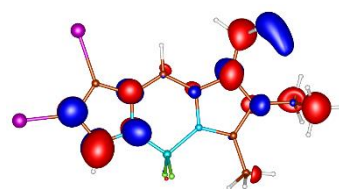

LUMO+4  
(0.33)

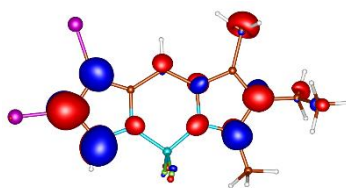

LUMO+5  
(0.54)

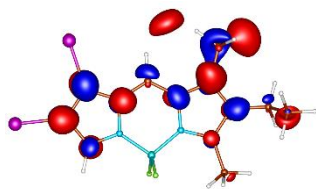

LUMO+6  
(0.82)

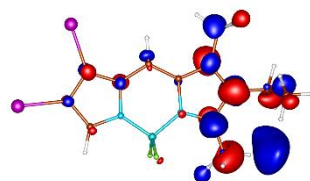

LUMO+7  
(1.09)

**Table S13a.** Spin-Orbit Couplings [ $\text{cm}^{-1}$ ] in monoiodinated BODIPY in the position 2 at  $S_0$  optimized geometry at CAS(18,15)SCF/ANO-RCC(TZP) level employing full two-electron Breit--Pauli spin--orbit Hamiltonian

| STATE           | T <sub>1</sub> | T <sub>2</sub> | T <sub>3</sub> | T <sub>4</sub> | T <sub>5</sub> | T <sub>6</sub> | T <sub>7</sub> | T <sub>8</sub> | T <sub>9</sub> | T <sub>10</sub> |
|-----------------|----------------|----------------|----------------|----------------|----------------|----------------|----------------|----------------|----------------|-----------------|
| S <sub>0</sub>  | 0.29           | 5.05           | 4.72           | 4.80           | 1893           | 2781           | 329            | 28.4           | 37.2           | 1121            |
| S <sub>1</sub>  | 1.00           | 1.37           | 0.82           | 0.17           | 69.1           | 329            | 708            | 1.15           | 2.09           | 249             |
| S <sub>2</sub>  | 1.11           | 0.58           | 0.96           | 0.09           | 30.8           | 87.3           | 215            | 0.71           | 0.31           | 106             |
| S <sub>3</sub>  | 2.65           | 0.03           | 0.35           | 0.93           | 32.7           | 65.5           | 703            | 0.37           | 2.07           | 62.6            |
| S <sub>4</sub>  | 1.13           | 0.74           | 1.06           | 0.30           | 29.1           | 154            | 378            | 1.00           | 4.08           | 44.6            |
| S <sub>5</sub>  | 175            | 96.9           | 66.5           | 36.4           | 2.03           | 1300           | 78.4           | 157            | 268            | 4.60            |
| S <sub>6</sub>  | 382            | 692            | 645            | 458            | 67.7           | 181            | 2.87           | 23.1           | 20.5           | 22.4            |
| S <sub>7</sub>  | 3.62           | 0.86           | 0.93           | 1.76           | 67.8           | 87.7           | 1717           | 0.78           | 0.64           | 41.8            |
| S <sub>8</sub>  | 356            | 162            | 160            | 93.3           | 2.30           | 1402           | 55.3           | 36.4           | 34.2           | 3.95            |
| S <sub>9</sub>  | 3.89           | 1.44           | 0.22           | 0.69           | 6.18           | 85.0           | 681            | 0.35           | 0.10           | 115             |
| S <sub>10</sub> | 2.49           | 2.74           | 2.92           | 0.27           | 16.8           | 29.8           | 266            | 1.06           | 0.43           | 84.6            |

**Table S13b.** Spin-Orbit Couplings [ $\text{cm}^{-1}$ ] in monoiodinated BODIPY in the position 2 at  $S_0$  optimized geometry at CAS(18,15)SCF/ANO-RCC(TZP) level employing full two-electron DKH1 spin--orbit Hamiltonian

| STATE           | T <sub>1</sub> | T <sub>2</sub> | T <sub>3</sub> | T <sub>4</sub> | T <sub>5</sub> | T <sub>6</sub> | T <sub>7</sub> | T <sub>8</sub> | T <sub>9</sub> | T <sub>10</sub> |
|-----------------|----------------|----------------|----------------|----------------|----------------|----------------|----------------|----------------|----------------|-----------------|
| S <sub>0</sub>  | 0.20           | 4.27           | 3.93           | 3.98           | 1564           | 2296           | 271            | 23.5           | 30.7           | 925             |
| S <sub>1</sub>  | 0.85           | 1.16           | 0.62           | 0.13           | 57.7           | 272            | 584            | 0.97           | 1.80           | 206             |
| S <sub>2</sub>  | 0.92           | 0.50           | 0.85           | 0.04           | 25.4           | 72.1           | 177            | 0.62           | 0.30           | 87.4            |
| S <sub>3</sub>  | 2.28           | 0.09           | 0.31           | 0.78           | 27.1           | 54.1           | 581            | 0.32           | 1.75           | 51.9            |
| S <sub>4</sub>  | 0.91           | 0.6            | 0.89           | 0.25           | 24.2           | 127            | 312            | 0.84           | 3.41           | 36.9            |
| S <sub>5</sub>  | 145            | 80.2           | 55.04          | 30.1           | 1.67           | 1074           | 64.7           | 130            | 222            | 3.80            |
| S <sub>6</sub>  | 315            | 571            | 532            | 378            | 55.9           | 151            | 2.37           | 19.1           | 16.9           | 18.5            |
| S <sub>7</sub>  | 2.99           | 0.71           | 0.81           | 1.49           | 56.3           | 72.4           | 1418           | 0.65           | 0.54           | 34.6            |
| S <sub>8</sub>  | 294            | 133            | 133            | 77.30          | 1.90           | 1157           | 45.7           | 30.0           | 28.1           | 3.27            |
| S <sub>9</sub>  | 3.25           | 1.22           | 0.25           | 0.56           | 5.02           | 70.2           | 562            | 0.28           | 0.08           | 95.7            |
| S <sub>10</sub> | 2.08           | 2.36           | 2.47           | 0.22           | 13.9           | 24.6           | 220            | 0.90           | 0.37           | 70.0            |

**Table S13c.** Spin-Orbit Couplings [ $\text{cm}^{-1}$ ] in monoiodinated BODIPY in the position 2 at  $S_0$  optimized geometry at CAS(18,15)SCF/ANO-RCC(TZP) level employing one-electron mean-field DKH1 spin--orbit Hamiltonian

| STATE           | T <sub>1</sub> | T <sub>2</sub> | T <sub>3</sub> | T <sub>4</sub> | T <sub>5</sub> | T <sub>6</sub> | T <sub>7</sub> | T <sub>8</sub> | T <sub>9</sub> | T <sub>10</sub> |
|-----------------|----------------|----------------|----------------|----------------|----------------|----------------|----------------|----------------|----------------|-----------------|
| S <sub>0</sub>  | 0.20           | 4.29           | 3.92           | 3.97           | 1564           | 2296           | 271            | 23.5           | 30.7           | 924             |
| S <sub>1</sub>  | 0.85           | 1.15           | 0.61           | 0.12           | 57.7           | 272            | 584            | 0.95           | 1.80           | 206             |
| S <sub>2</sub>  | 0.91           | 0.50           | 0.84           | 0.05           | 25.4           | 72.1           | 177            | 0.61           | 0.30           | 87.4            |
| S <sub>3</sub>  | 2.31           | 0.09           | 0.30           | 0.78           | 27.1           | 54.1           | 581            | 0.32           | 1.76           | 51.7            |
| S <sub>4</sub>  | 0.89           | 0.62           | 0.89           | 0.25           | 24.2           | 127            | 312            | 0.84           | 3.40           | 36.9            |
| S <sub>5</sub>  | 145            | 80.3           | 55.0           | 30.2           | 1.67           | 1074           | 64.7           | 130            | 222            | 3.81            |
| S <sub>6</sub>  | 315            | 571            | 532            | 378            | 55.9           | 150            | 2.37           | 19.1           | 17.0           | 18.5            |
| S <sub>7</sub>  | 2.98           | 0.70           | 0.83           | 1.50           | 56.3           | 72.4           | 1418           | 0.65           | 0.53           | 34.6            |
| S <sub>8</sub>  | 294            | 134            | 133            | 77.3           | 1.90           | 1157           | 45.7           | 30.0           | 28.1           | 3.27            |
| S <sub>9</sub>  | 3.26           | 1.24           | 0.26           | 0.57           | 5.03           | 70.2           | 562            | 0.27           | 0.08           | 95.7            |
| S <sub>10</sub> | 2.08           | 2.38           | 2.47           | 0.22           | 14.00          | 24.6           | 220            | 0.90           | 0.39           | 70.1            |



**Table S13d.** Spin-Orbit Couplings [ $\text{cm}^{-1}$ ] in monoiodinated BODIPY in the position 2 at  $S_0$  optimized geometry at CAS(18,15)SCF/ANO-RCC(TZP) level employing one-electron one-center flexible nuclear screening DKH1 spin--orbit Hamiltonian

| STATE           | T <sub>1</sub> | T <sub>2</sub> | T <sub>3</sub> | T <sub>4</sub> | T <sub>5</sub> | T <sub>6</sub> | T <sub>7</sub> | T <sub>8</sub> | T <sub>9</sub> | T <sub>10</sub> |
|-----------------|----------------|----------------|----------------|----------------|----------------|----------------|----------------|----------------|----------------|-----------------|
| S <sub>0</sub>  | 0.19           | 4.37           | 3.92           | 3.96           | 1564           | 2296           | 271            | 23.5           | 30.7           | 925             |
| S <sub>1</sub>  | 0.85           | 1.16           | 0.60           | 0.11           | 57.6           | 272            | 585            | 0.99           | 1.81           | 206             |
| S <sub>2</sub>  | 0.90           | 0.50           | 0.87           | 0.06           | 25.4           | 72.2           | 177            | 0.63           | 0.31           | 87.4            |
| S <sub>3</sub>  | 2.38           | 0.09           | 0.31           | 0.79           | 27.1           | 54.1           | 581            | 0.32           | 1.76           | 52.0            |
| S <sub>4</sub>  | 0.88           | 0.62           | 0.90           | 0.25           | 24.1           | 127            | 312            | 0.83           | 3.41           | 36.8            |
| S <sub>5</sub>  | 145            | 80.2           | 55.0           | 30.1           | 1.66           | 1074           | 64.8           | 130            | 222            | 3.83            |
| S <sub>6</sub>  | 315            | 571            | 533            | 379            | 55.9           | 150            | 2.38           | 19.1           | 17.0           | 18.5            |
| S <sub>7</sub>  | 2.96           | 0.69           | 0.83           | 1.49           | 56.2           | 72.5           | 1419           | 0.63           | 0.53           | 34.7            |
| S <sub>8</sub>  | 294            | 134            | 133            | 77.2           | 1.92           | 1158           | 45.8           | 30.0           | 28.2           | 3.29            |
| S <sub>9</sub>  | 3.27           | 1.26           | 0.28           | 0.58           | 5.02           | 70.2           | 562            | 0.29           | 0.06           | 95.5            |
| S <sub>10</sub> | 2.08           | 2.43           | 2.47           | 0.22           | 13.9           | 24.7           | 220            | 0.90           | 0.41           | 70.0            |

**Table S14.** Spin-Orbit Couplings [ $\text{cm}^{-1}$ ] in monoiodinated BODIPY in the position 2 at  $S_0$  optimized geometry at ADC(2)/dhf-TZVP level

| STATE           | T <sub>1</sub> | T <sub>2</sub> | T <sub>3</sub> | T <sub>4</sub> | T <sub>5</sub> | T <sub>6</sub> | T <sub>7</sub> | T <sub>8</sub> | T <sub>9</sub> | T <sub>10</sub> |
|-----------------|----------------|----------------|----------------|----------------|----------------|----------------|----------------|----------------|----------------|-----------------|
| S <sub>0</sub>  | 1.69           | 8.29           | 3.55           | 11.1           | 1604           | 1892           | 22.7           | 36.0           | 5.98           | 4.54            |
| S <sub>1</sub>  | 0.13           | 0.42           | 0.52           | 0.45           | 17.8           | 55.2           | 0.55           | 1.56           | 0.73           | 0.21            |
| S <sub>2</sub>  | 0.87           | 1.51           | 3.01           | 0.21           | 74.5           | 38.0           | 0.19           | 0.68           | 0.36           | 0.45            |
| S <sub>3</sub>  | 0.40           | 3.10           | 2.23           | 1.70           | 12.11          | 23.6           | 3.16           | 1.28           | 0.11           | 1.36            |
| S <sub>4</sub>  | 413            | 766            | 430            | 596            | 2.84           | 172            | 1717           | 612            | 106            | 183             |
| S <sub>5</sub>  | 53.9           | 76.7           | 39.8           | 32.5           | 1.36           | 1781           | 143            | 119            | 141            | 111             |
| S <sub>6</sub>  | 0.69           | 2.78           | 2.26           | 0.12           | 103            | 30.2           | 2.16           | 2.65           | 1.68           | 0.87            |
| S <sub>7</sub>  | 4.02           | 10.9           | 5.41           | 2.53           | 1745           | 23.2           | 19.2           | 63.4           | 59.4           | 71.9            |
| S <sub>8</sub>  | 2.14           | 5.91           | 4.52           | 2.51           | 846            | 52.5           | 9.82           | 31.6           | 30.6           | 36.7            |
| S <sub>9</sub>  | 42.8           | 40.4           | 24.5           | 5.86           | 0.31           | 892            | 25.5           | 19.8           | 4.75           | 75.4            |
| S <sub>10</sub> | 0.36           | 0.34           | 0.28           | 0.25           | 35.1           | 41.4           | 1.32           | 0.07           | 2.16           | 1.47            |

**Table S15.** Spin-Orbit Couplings [ $\text{cm}^{-1}$ ] in monoiodinated BODIPY in the position 2 at  $S_0$  optimized geometry at TD-DFT(TDA)/BHLYP/dhf-TZVP level

| STATE           | T <sub>1</sub> | T <sub>2</sub> | T <sub>3</sub> | T <sub>4</sub> | T <sub>5</sub> | T <sub>6</sub> | T <sub>7</sub> | T <sub>8</sub> | T <sub>9</sub> | T <sub>10</sub> |
|-----------------|----------------|----------------|----------------|----------------|----------------|----------------|----------------|----------------|----------------|-----------------|
| S <sub>0</sub>  | 1.27           | 8.79           | 3.39           | 6.18           | 1527           | 234            | 1886           | 26.3           | 33.6           | 4.3             |
| S <sub>1</sub>  | 0.11           | 0.55           | 0.37           | 0.42           | 18.2           | 928            | 88.4           | 1.62           | 1.95           | 0.91            |
| S <sub>2</sub>  | 0.66           | 0.38           | 2.26           | 0.28           | 116            | 1104           | 74.7           | 1.15           | 2.00           | 0.74            |
| S <sub>3</sub>  | 0.49           | 2.43           | 1.20           | 1.29           | 14.2           | 399            | 21.1           | 0.37           | 2.16           | 0.53            |
| S <sub>4</sub>  | 320            | 781            | 392            | 374            | 3.16           | 18.1           | 987            | 377            | 1474           | 483             |
| S <sub>5</sub>  | 214            | 515            | 257            | 241            | 3.16           | 30.9           | 1405           | 241            | 1014           | 342             |
| S <sub>6</sub>  | 0.43           | 2.99           | 1.61           | 0.21           | 227            | 1545           | 70.7           | 3.97           | 7.44           | 5.14            |
| S <sub>7</sub>  | 3.98           | 12.3           | 6.07           | 2.42           | 1891           | 200            | 8.38           | 33.5           | 59.0           | 56.4            |
| S <sub>8</sub>  | 56.4           | 50.3           | 27.4           | 3.92           | 0.59           | 0.85           | 1072           | 13.2           | 50.8           | 5.12            |
| S <sub>9</sub>  | 0.00           | 0.69           | 0.52           | 0.82           | 79.1           | 803            | 94.0           | 0.48           | 0.71           | 1.89            |
| S <sub>10</sub> | 61.4           | 158            | 72.7           | 74.6           | 5.03           | 178            | 40.3           | 76.5           | 296            | 101             |

**Table S16.** Spin-Orbit Couplings [ $\text{cm}^{-1}$ ] in monoiodinated BODIPY in the position 2 at  $S_0$  optimized geometry at TD-DFT/B3LYP/dhf-TZVP level

| STATE           | T <sub>1</sub> | T <sub>2</sub> | T <sub>3</sub> | T <sub>4</sub> | T <sub>5</sub> | T <sub>6</sub> | T <sub>7</sub> | T <sub>8</sub> | T <sub>9</sub> | T <sub>10</sub> |
|-----------------|----------------|----------------|----------------|----------------|----------------|----------------|----------------|----------------|----------------|-----------------|
| S <sub>0</sub>  | 1.93           | 8.08           | 0.81           | 5.12           | 261            | 1361           | 23             | 1843           | 66.9           | 833             |
| S <sub>1</sub>  | 0.36           | 0.41           | 1.61           | 0.65           | 1476           | 83.2           | 0.33           | 23.3           | 0.94           | 15.9            |
| S <sub>2</sub>  | 0.83           | 1.07           | 2.67           | 0.15           | 962            | 55.2           | 1.35           | 63.8           | 2.61           | 146             |
| S <sub>3</sub>  | 583            | 1248           | 411            | 696            | 1.97           | 15.5           | 1723           | 109            | 51.9           | 59.7            |
| S <sub>4</sub>  | 0.34           | 3.79           | 2.15           | 3.75           | 221            | 5.54           | 3.28           | 20.5           | 0.63           | 25.1            |
| S <sub>5</sub>  | 88.8           | 76.8           | 14.3           | 0.97           | 18.7           | 0.23           | 10.9           | 1425           | 113            | 0.61            |
| S <sub>6</sub>  | 1.35           | 2.84           | 5.13           | 0.69           | 1454           | 41.7           | 1.07           | 55.1           | 2.72           | 86.2            |
| S <sub>7</sub>  | 45.8           | 103            | 30.9           | 10.6           | 14.6           | 0.64           | 20.9           | 1188           | 45.3           | 1.06            |
| S <sub>8</sub>  | 3.47           | 12.4           | 3.12           | 7.36           | 189            | 1652           | 25.7           | 9.05           | 45.9           | 1028            |
| S <sub>9</sub>  | 0.38           | 6.09           | 0.57           | 4.17           | 499            | 495            | 10.5           | 45.9           | 11.7           | 306             |
| S <sub>10</sub> | 85.7           | 188            | 56.0           | 106            | 262            | 4.72           | 256            | 33.8           | 6.32           | 7.36            |

**Table S17.** Spin-Orbit Couplings [ $\text{cm}^{-1}$ ] in monoiodinated BODIPY in the position 2 at  $S_0$  optimized geometry at TD-DFT/M06-2X/dhf-TZVP level

| STATE           | T <sub>1</sub> | T <sub>2</sub> | T <sub>3</sub> | T <sub>4</sub> | T <sub>5</sub> | T <sub>6</sub> | T <sub>7</sub> | T <sub>8</sub> | T <sub>9</sub> | T <sub>10</sub> |
|-----------------|----------------|----------------|----------------|----------------|----------------|----------------|----------------|----------------|----------------|-----------------|
| S <sub>0</sub>  | 2.04           | 10.7           | 4.46           | 6.95           | 1541           | 227            | 1881           | 4.72           | 24.5           | 8.48            |
| S <sub>1</sub>  | 0.07           | 0.45           | 0.25           | 0.32           | 18.7           | 794            | 62.9           | 0.17           | 1.00           | 0.72            |
| S <sub>2</sub>  | 0.66           | 0.23           | 2.71           | 0.55           | 94.6           | 1129           | 50.4           | 0.14           | 1.86           | 1.79            |
| S <sub>3</sub>  | 0.52           | 2.66           | 0.98           | 1.48           | 18.1           | 433            | 8.47           | 1.94           | 0.58           | 0.77            |
| S <sub>4</sub>  | 393            | 958            | 483            | 494            | 6.61           | 1.57           | 198            | 1694           | 878            | 204             |
| S <sub>5</sub>  | 66.6           | 113            | 54.9           | 38.9           | 0.93           | 21.5           | 1801           | 168            | 171            | 242             |
| S <sub>6</sub>  | 0.20           | 3.23           | 1.57           | 0.46           | 165            | 1559           | 60.7           | 0.09           | 9.33           | 11.2            |
| S <sub>7</sub>  | 8.20           | 19.9           | 11.7           | 0.14           | 1926           | 155            | 9.97           | 5.92           | 128            | 172             |
| S <sub>8</sub>  | 61.2           | 54.0           | 28.2           | 4.69           | 0.16           | 4.90           | 926            | 39.2           | 19.5           | 25.9            |
| S <sub>9</sub>  | 0.04           | 0.61           | 0.71           | 0.81           | 71.9           | 938            | 74.7           | 0.74           | 1.29           | 2.55            |
| S <sub>10</sub> | 71.8           | 184            | 86.7           | 92.5           | 2.87           | 104            | 27.1           | 319            | 160            | 45.5            |

**Table S18.** Spin-Orbit Couplings [ $\text{cm}^{-1}$ ] in I-BODIPY at  $S_0$  optimized geometry at ADC(2)/dhf-TZVP level

| STATE           | T <sub>1</sub> | T <sub>2</sub> | T <sub>3</sub> | T <sub>4</sub> | T <sub>5</sub> | T <sub>6</sub> | T <sub>7</sub> | T <sub>8</sub> | T <sub>9</sub> | T <sub>10</sub> |
|-----------------|----------------|----------------|----------------|----------------|----------------|----------------|----------------|----------------|----------------|-----------------|
| S <sub>0</sub>  | 1.64           | 4.93           | 2.54           | 13.5           | 1556           | 1431           | 250            | 2681           | 203            | 500             |
| S <sub>1</sub>  | 0.19           | 0.48           | 0.53           | 1.78           | 41.6           | 19.6           | 504            | 66.7           | 465            | 6.20            |
| S <sub>2</sub>  | 0.89           | 1.36           | 2.24           | 2.07           | 37.0           | 29.1           | 1002           | 46.5           | 716            | 8.26            |
| S <sub>3</sub>  | 0.53           | 2.46           | 1.66           | 1.27           | 14.5           | 9.56           | 265            | 23.3           | 217            | 2.33            |
| S <sub>4</sub>  | 60.2           | 15.8           | 17.6           | 22.4           | 15.7           | 2.82           | 15.6           | 1018           | 13.5           | 42.9            |
| S <sub>5</sub>  | 354            | 705            | 624            | 579            | 1.81           | 5.32           | 1.63           | 115            | 98.5           | 35.5            |
| S <sub>6</sub>  | 63.6           | 91.8           | 77.03          | 41.6           | 1.42           | 5.78           | 28.7           | 1224           | 50.8           | 31.5            |
| S <sub>7</sub>  | 340            | 477            | 422            | 545            | 18.9           | 26.9           | 333            | 48.3           | 317            | 14.8            |
| S <sub>8</sub>  | 110            | 157            | 138            | 180            | 52.7           | 79.2           | 1005           | 58.4           | 986            | 8.93            |
| S <sub>9</sub>  | 49.0           | 72.5           | 55.8           | 21.3           | 71.8           | 20.3           | 31.5           | 847            | 6.38           | 42.5            |
| S <sub>10</sub> | 3.61           | 15.5           | 14.3           | 2.70           | 45.0           | 42.6           | 36.3           | 53.8           | 18.3           | 2.43            |

**Table S19.** Spin-Orbit Couplings [ $\text{cm}^{-1}$ ] in I-BODIPY at  $S_0$  optimized geometry at TD-DFT(TDA)/BHLYP/dhf-TZVP level

| STATE           | T <sub>1</sub> | T <sub>2</sub> | T <sub>3</sub> | T <sub>4</sub> | T <sub>5</sub> | T <sub>6</sub> | T <sub>7</sub> | T <sub>8</sub> | T <sub>9</sub> | T <sub>10</sub> |
|-----------------|----------------|----------------|----------------|----------------|----------------|----------------|----------------|----------------|----------------|-----------------|
| S <sub>0</sub>  | 1.74           | 2.49           | 3.81           | 11.7           | 1544           | 1326           | 339            | 2635           | 445            | 25.5            |
| S <sub>1</sub>  | 0.12           | 0.64           | 0.70           | 1.55           | 46.1           | 24.6           | 491            | 118            | 25.9           | 1.99            |
| S <sub>2</sub>  | 0.73           | 1.31           | 1.36           | 1.26           | 47.9           | 34.4           | 1243           | 70.7           | 59.0           | 1.09            |
| S <sub>3</sub>  | 0.63           | 1.46           | 1.66           | 0.88           | 17.4           | 21.5           | 423            | 28.6           | 1.03           | 0.50            |
| S <sub>4</sub>  | 76.0           | 18.6           | 33.8           | 22.6           | 13.7           | 3.95           | 39.1           | 1057           | 780            | 108             |
| S <sub>5</sub>  | 71.0           | 86.2           | 158            | 23.3           | 1.8            | 9.19           | 47.8           | 1188           | 1162           | 8.47            |
| S <sub>6</sub>  | 332            | 466            | 898            | 491            | 2.28           | 8.48           | 6.20           | 66.9           | 119            | 828             |
| S <sub>7</sub>  | 359            | 339            | 670            | 596            | 8.02           | 7.09           | 143            | 63.9           | 83.2           | 801.8           |
| S <sub>8</sub>  | 4.29           | 6.43           | 10.3           | 9.18           | 97.7           | 152            | 1320           | 135            | 40.7           | 15.6            |
| S <sub>9</sub>  | 7.28           | 2.77           | 5.10           | 1.69           | 1496           | 1032           | 116            | 15.1           | 12.9           | 9.41            |
| S <sub>10</sub> | 54.8           | 56.0           | 97.7           | 22.8           | 86.1           | 18.0           | 40.7           | 795            | 1015           | 41.4            |

**Table S20.** Spin-Orbit Couplings [ $\text{cm}^{-1}$ ] in I-BODIPY at  $S_0$  optimized geometry at TD-DFT B3LYP/dhf-TZVP level

| STATE           | T <sub>1</sub> | T <sub>2</sub> | T <sub>3</sub> | T <sub>4</sub> | T <sub>5</sub> | T <sub>6</sub> | T <sub>7</sub> | T <sub>8</sub> | T <sub>9</sub> | T <sub>10</sub> |
|-----------------|----------------|----------------|----------------|----------------|----------------|----------------|----------------|----------------|----------------|-----------------|
| S <sub>0</sub>  | 1.89           | 3.25           | 1.41           | 8.29           | 290            | 1090           | 1314           | 348            | 16.2           | 2470            |
| S <sub>1</sub>  | 0.43           | 1.15           | 1.61           | 2.65           | 1071           | 86.4           | 38.7           | 753            | 3.14           | 37.3            |
| S <sub>2</sub>  | 0.88           | 2.07           | 1.99           | 3.87           | 1121           | 16.1           | 104            | 1079           | 5.05           | 43.5            |
| S <sub>3</sub>  | 0.81           | 2.82           | 1.32           | 2.16           | 392            | 19.0           | 12.6           | 316            | 2.69           | 14.9            |
| S <sub>4</sub>  | 432            | 1077           | 616            | 892            | 3.02           | 11.1           | 18.8           | 124            | 1241           | 93.5            |
| S <sub>5</sub>  | 112            | 42.6           | 15.1           | 23.1           | 0.24           | 20.0           | 15.2           | 1.15           | 12.5           | 769             |
| S <sub>6</sub>  | 470            | 811            | 452            | 907            | 125            | 4.39           | 28.3           | 14.8           | 1479           | 50.9            |
| S <sub>7</sub>  | 1.48           | 8.31           | 3.24           | 9.37           | 1408           | 58.4           | 6.92           | 1463           | 16.8           | 98.6            |
| S <sub>8</sub>  | 48.9           | 139            | 68.6           | 22.4           | 23.9           | 5.62           | 8.33           | 42.9           | 33.2           | 1274            |
| S <sub>9</sub>  | 93.5           | 56.7           | 20.6           | 14.9           | 8.68           | 96.6           | 27.7           | 9.59           | 22.9           | 294             |
| S <sub>10</sub> | 4.95           | 2.87           | 0.77           | 5.05           | 254            | 1136           | 1009           | 311            | 11.7           | 42.3            |



**Table S21.** Spin-Orbit Couplings [ $\text{cm}^{-1}$ ] in I-BODIPY at  $S_0$  optimized geometry at TD-DFT(TDA)/M06-2X/dhf-TZVP level

| STATE           | T <sub>1</sub> | T <sub>2</sub> | T <sub>3</sub> | T <sub>4</sub> | T <sub>5</sub> | T <sub>6</sub> | T <sub>7</sub> | T <sub>8</sub> | T <sub>9</sub> | T <sub>10</sub> |
|-----------------|----------------|----------------|----------------|----------------|----------------|----------------|----------------|----------------|----------------|-----------------|
| S <sub>0</sub>  | 2.05           | 4.17           | 6.87           | 12.1           | 1527           | 1328           | 321            | 2605           | 450            | 270             |
| S <sub>1</sub>  | 0.13           | 0.56           | 0.48           | 1.98           | 43.9           | 31.2           | 440            | 82.5           | 52.4           | 572             |
| S <sub>2</sub>  | 0.70           | 1.11           | 1.82           | 1.74           | 53.6           | 51.0           | 1253           | 34.4           | 71.9           | 794             |
| S <sub>3</sub>  | 0.66           | 1.72           | 1.49           | 1.19           | 25.9           | 22.1           | 484            | 17.8           | 34.0           | 418             |
| S <sub>4</sub>  | 69.3           | 23.2           | 33.0           | 18.8           | 10.3           | 2.56           | 8.60           | 1182           | 802            | 71.3            |
| S <sub>5</sub>  | 338            | 573            | 934            | 536            | 8.06           | 13.4           | 2.41           | 293            | 177            | 146             |
| S <sub>6</sub>  | 121            | 55.8           | 85.9           | 128            | 1.15           | 6.25           | 22.4           | 1119           | 1200           | 111             |
| S <sub>7</sub>  | 384            | 408            | 686            | 700            | 13.3           | 4.01           | 155            | 60.2           | 70.1           | 40.7            |
| S <sub>8</sub>  | 6.93           | 9.82           | 14.5           | 16.0           | 82.5           | 115            | 1315           | 102            | 130            | 1550            |
| S <sub>9</sub>  | 14.0           | 6.42           | 10.1           | 4.87           | 1537           | 1014           | 105            | 7.58           | 25.6           | 45.2            |
| S <sub>10</sub> | 48.5           | 61.8           | 90.9           | 21.5           | 86.8           | 8.55           | 30.6           | 840            | 1050           | 86.6            |

**Graphs showing variation in magnitudes of SOC in I-BODIPY between selected singlets and triplets along the PEC.**

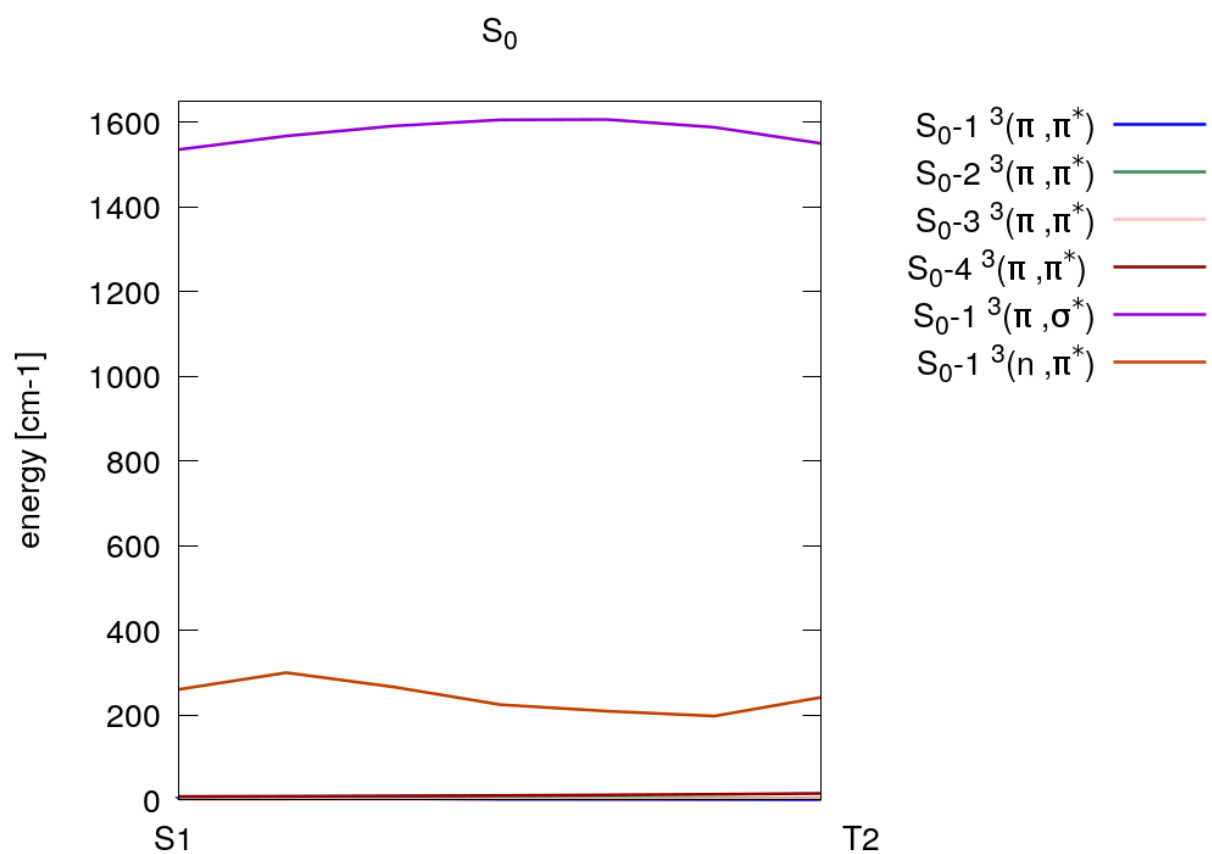

**Figure S5.** SOC between ground state S<sub>0</sub> and 6 triplets at ADC(2)/dhf-TZVP level along the PEC.

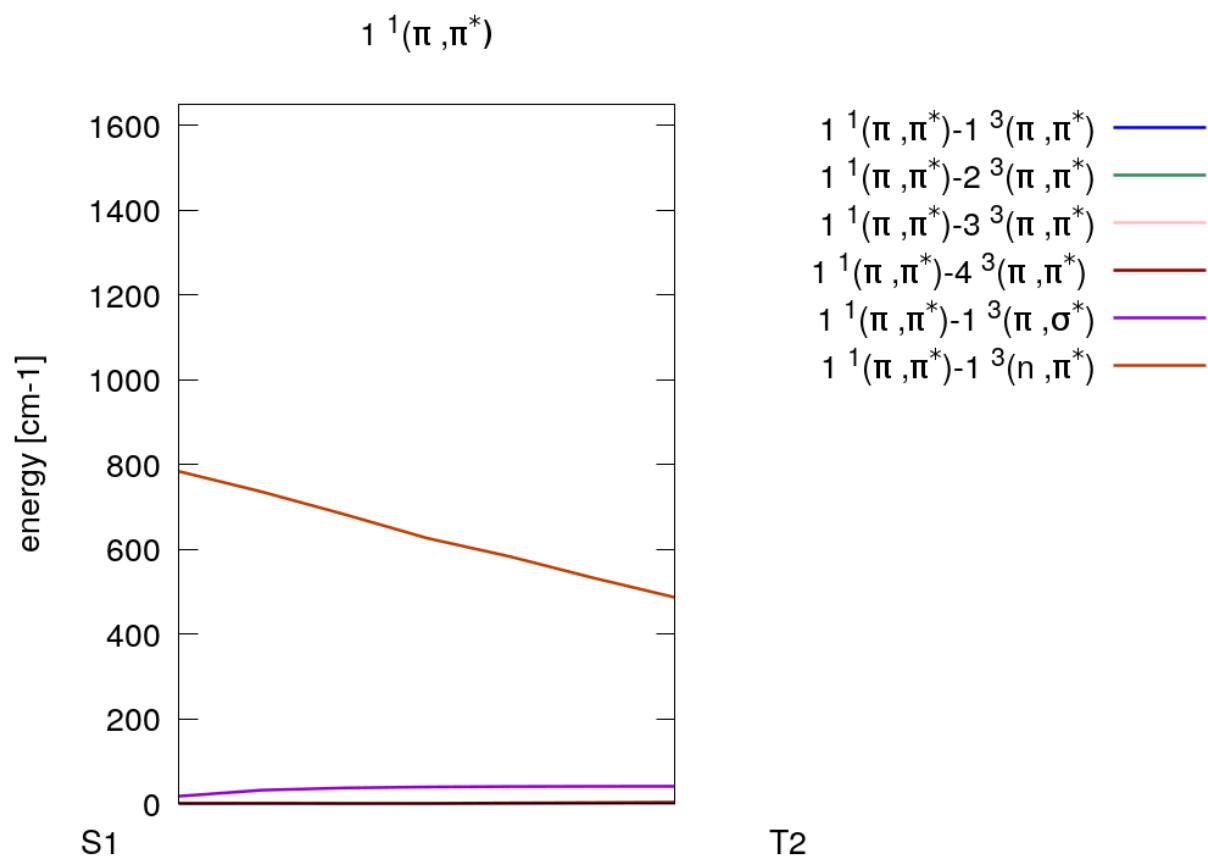

**Figure S6.** SOCs between excited state  $1^1(\pi, \pi^*)$  and 6 triplets at ADC(2)/dhf-TZVP level along the PEC.

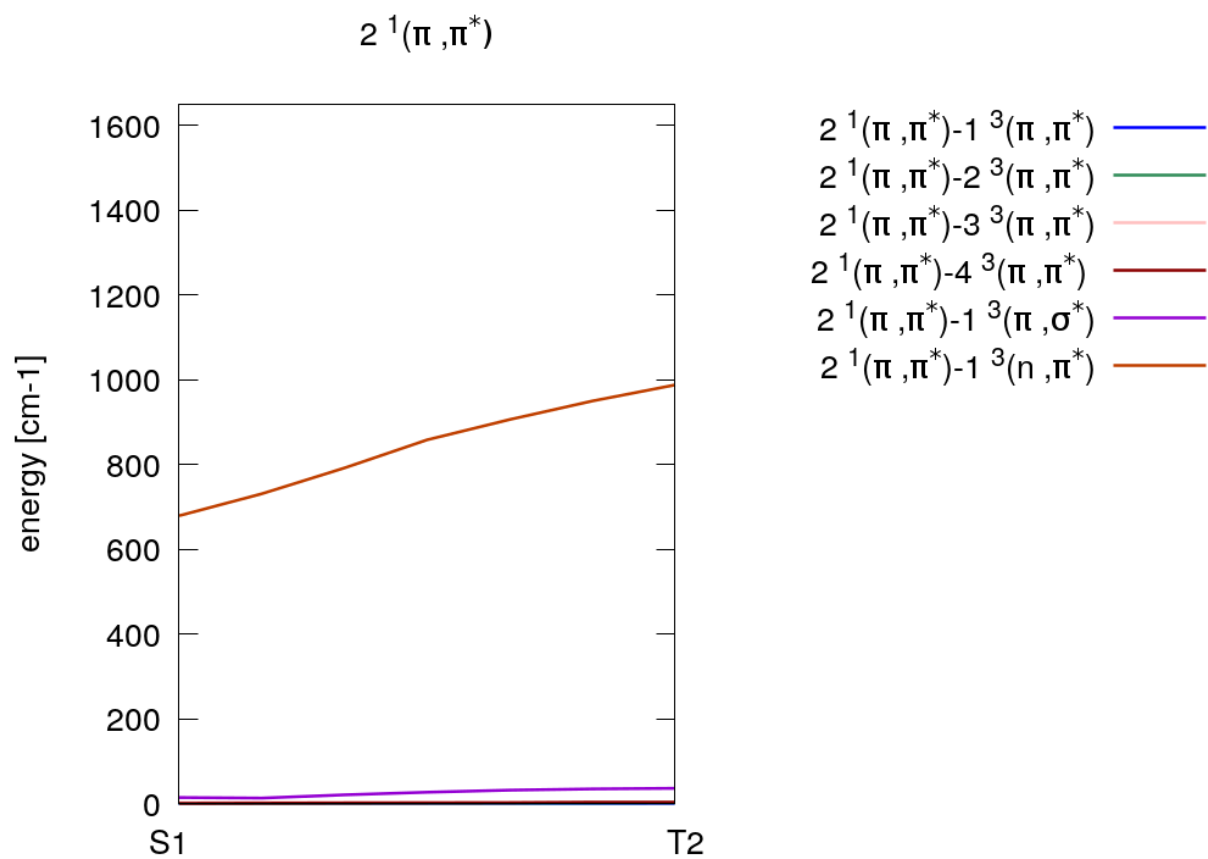

**Figure S7.** SOCs between excited state  $2^1(\pi, \pi^*)$  and 6 triplets at ADC(2)/dhf-TZVP level along the PEC.

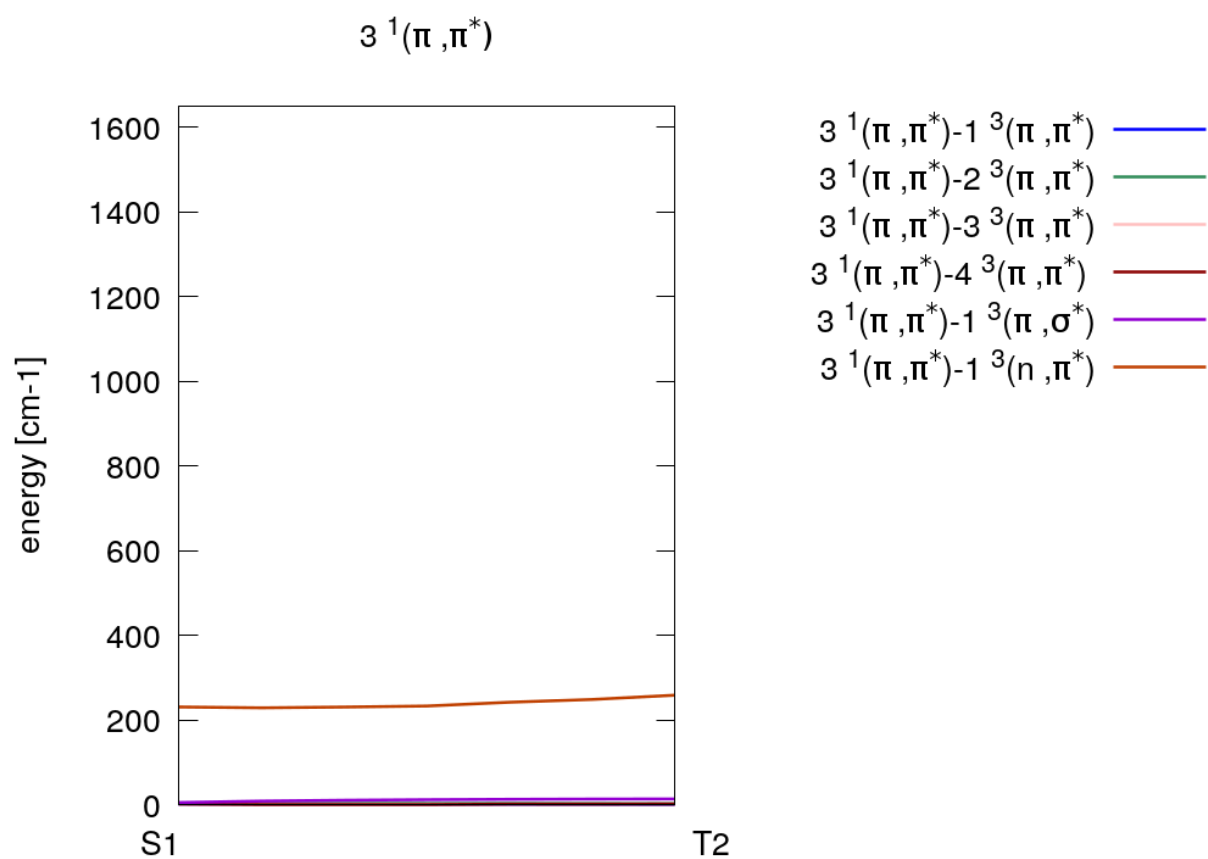

**Figure S8.** SOC between excited state  $3^1(\pi, \pi^*)$  and 6 triplets at ADC(2)/dhf-TZVP level along the PEC.

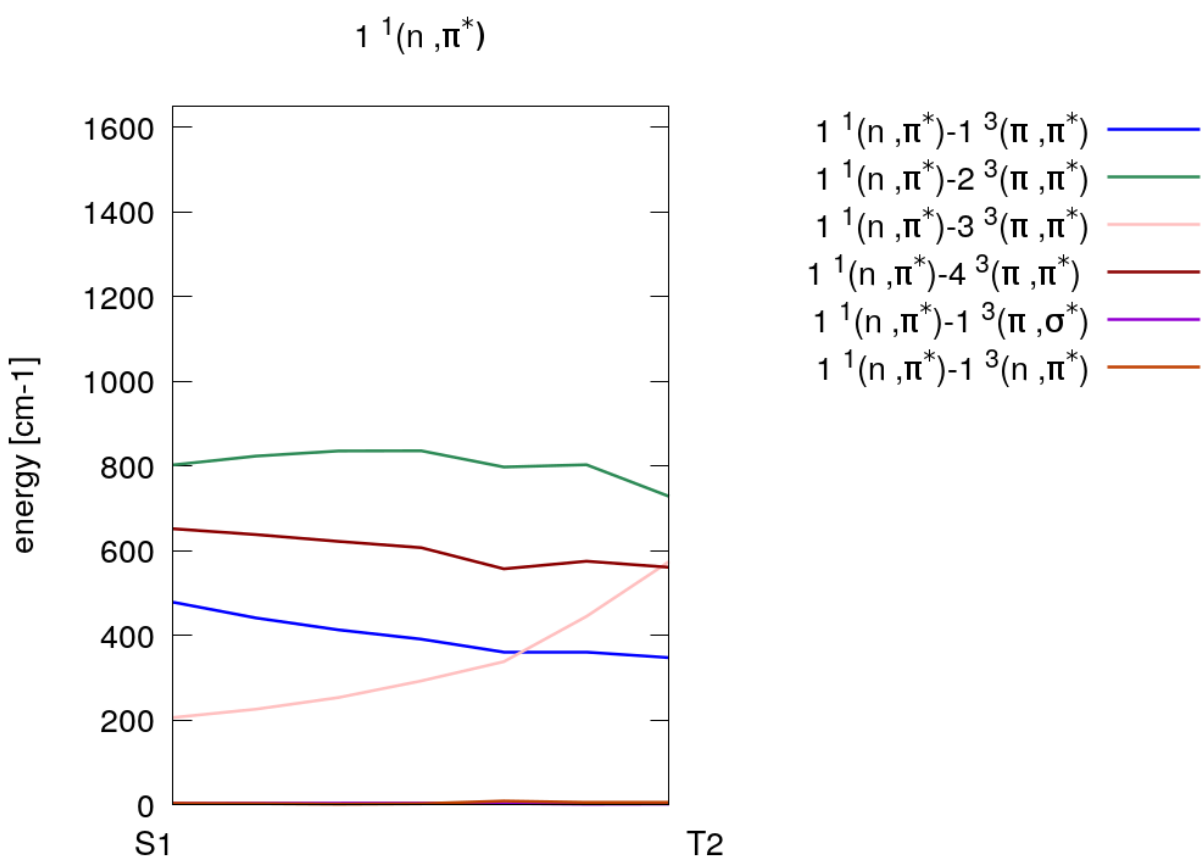

**Figure S9.** SOCs between excited state  $1^1(n, \pi^*)$  and 6 triplets at ADC(2)/dhf-TZVP level along the PEC.





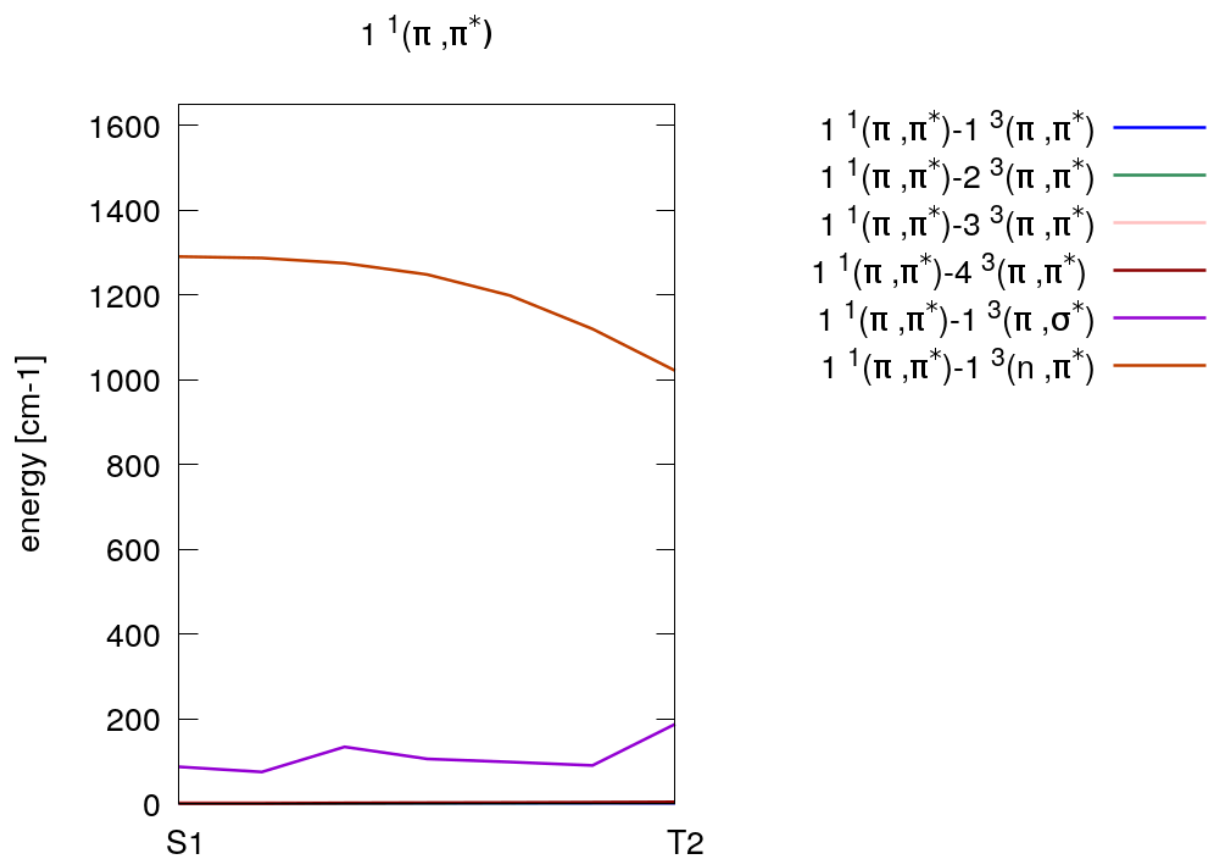

**Figure S11.** SOC between excited state  $1^1(\pi, \pi^*)$  and 6 triplets at TD-DFT/B3LYP/dhf-TZVP level along the PEC.

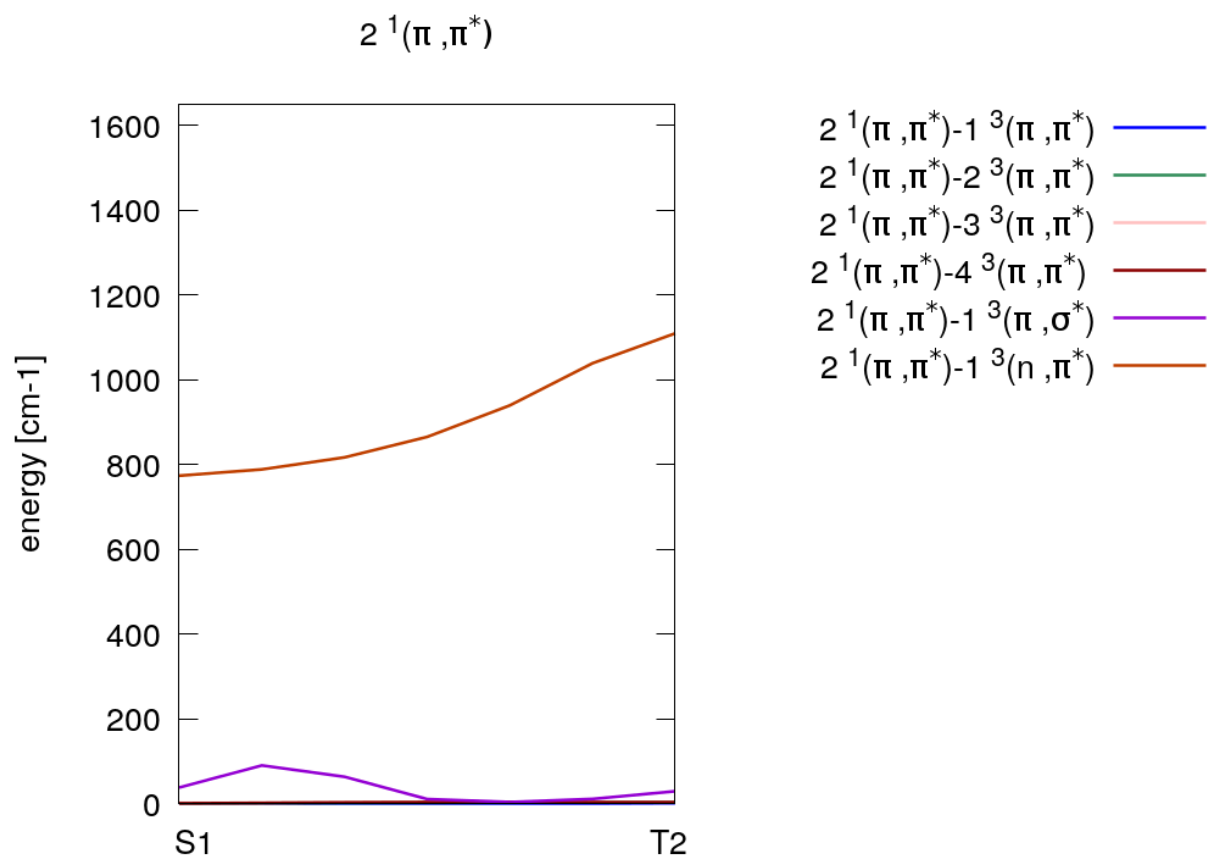

**Figure S12.** SOCs between excited state  $2^1(\pi, \pi^*)$  and 6 triplets at TD-DFT/B3LYP/dhf-TZVP level along the PEC.

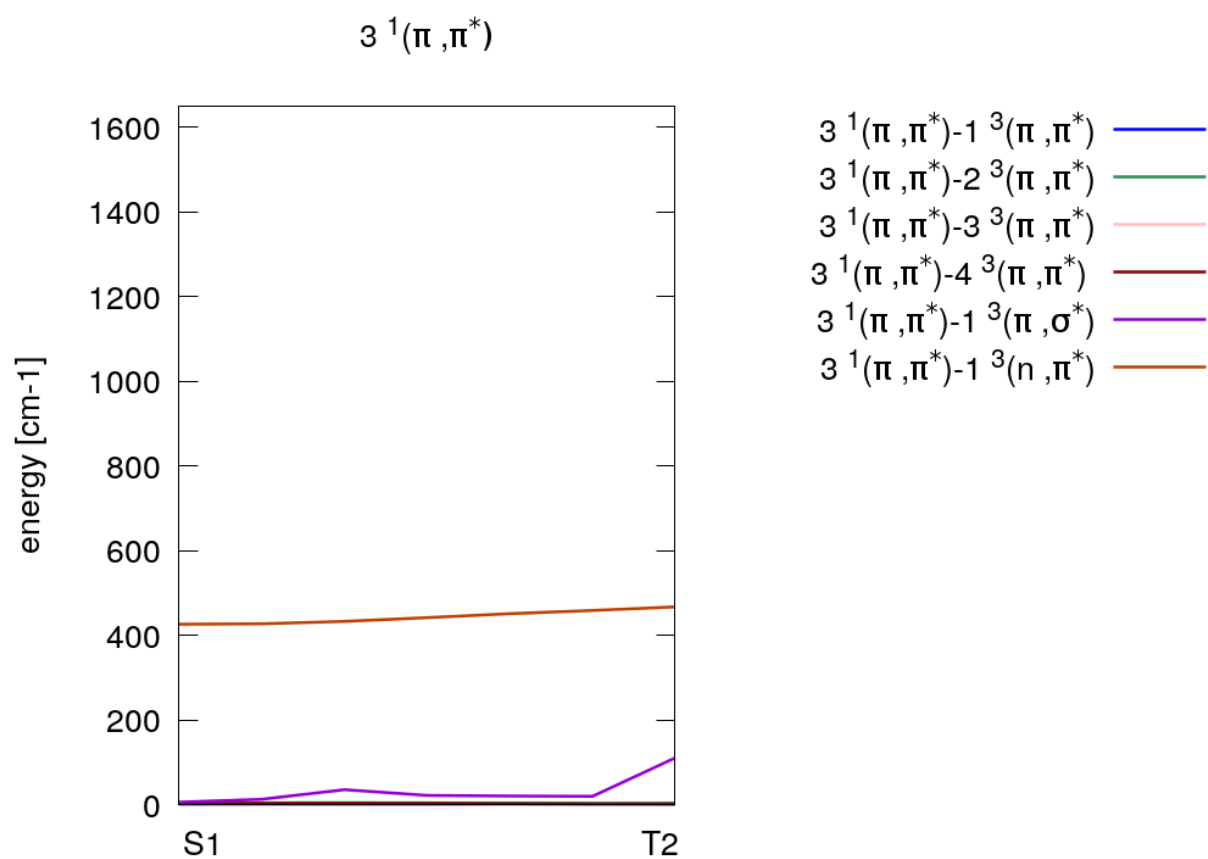

**Figure S13.** SOCs between excited state  $3^1(\pi, \pi^*)$  and 6 triplets at TD-DFT/B3LYP/dhf-TZVP level along the PEC.

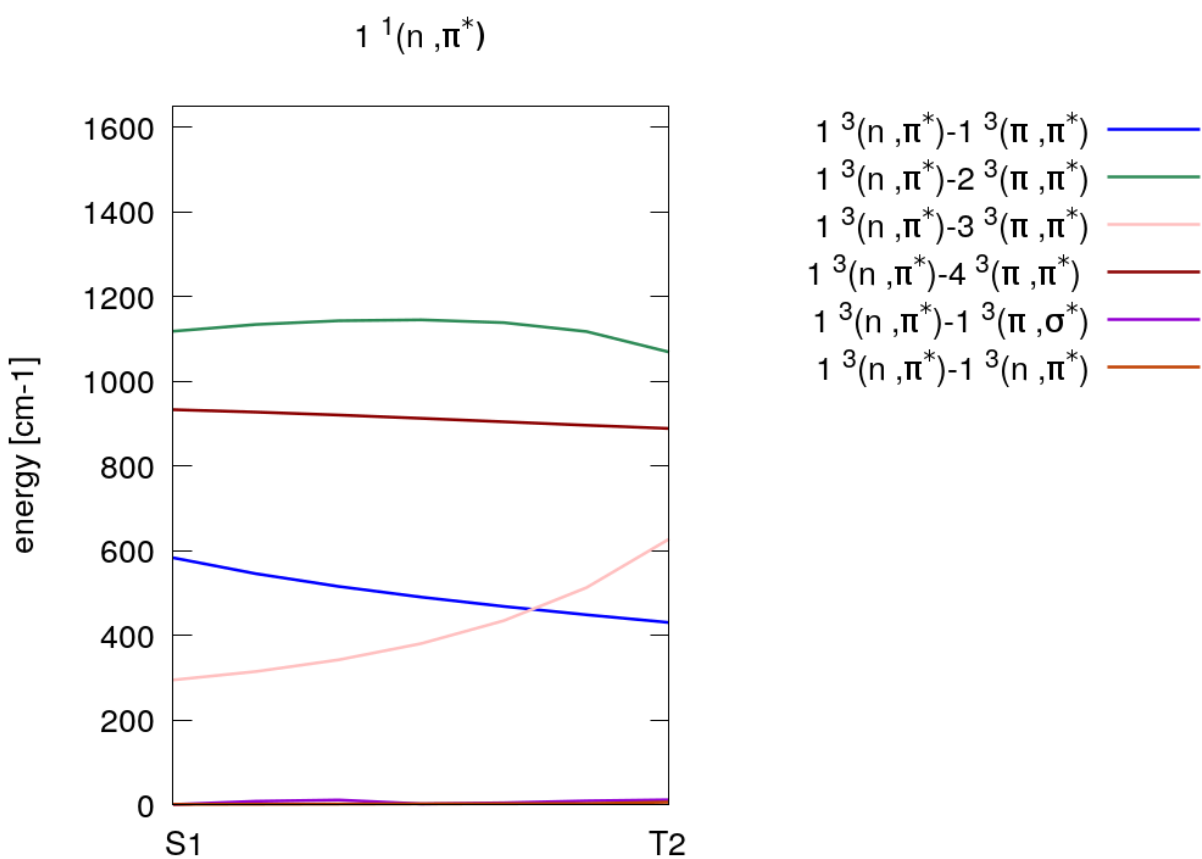

**Figure S14.** SOCs between excited state  $1^1(n, \pi^*)$  and 6 triplets at TD-DFT/B3LYP/dhf-TZVP level along the PEC.



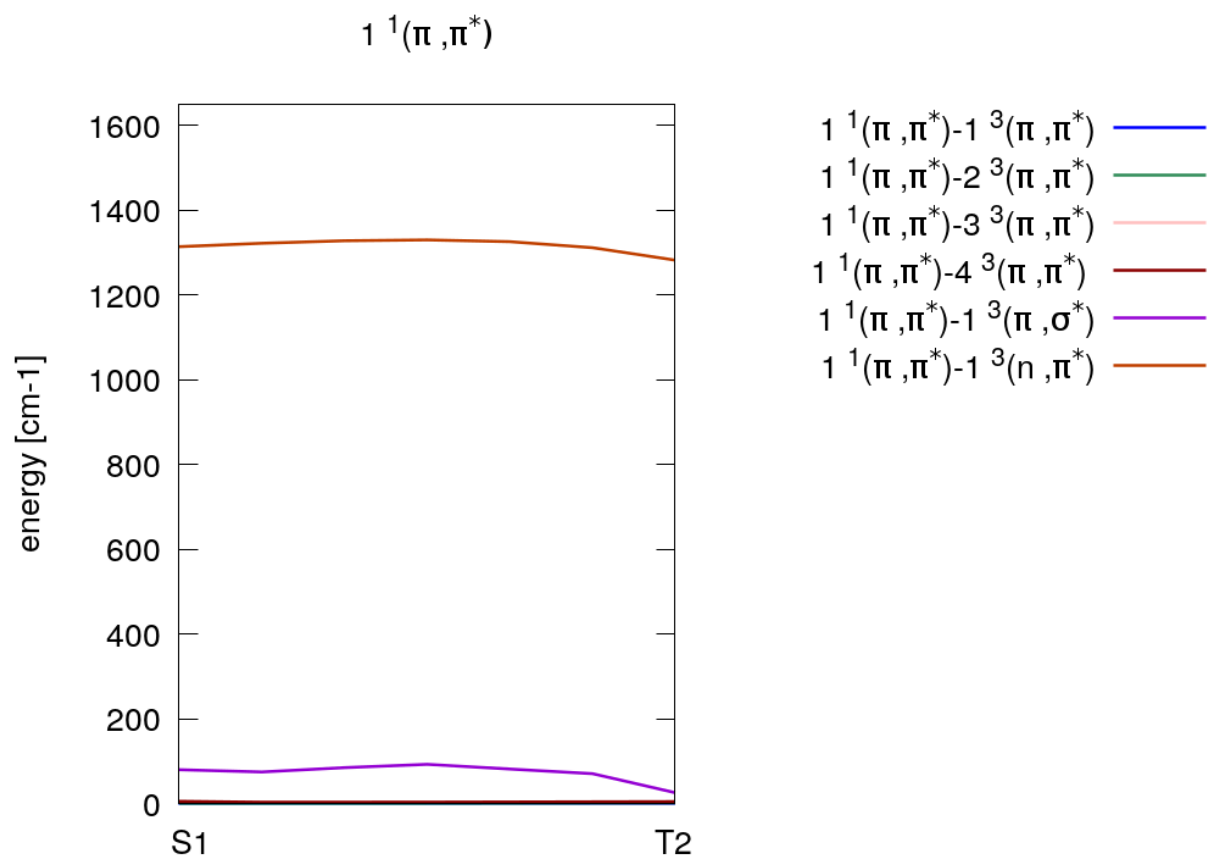

**Figure S16.** SOC between excited state  $1^1(\pi, \pi^*)$  and 6 triplets at TD-DFT(TDA)/B3LYP/dhf-TZVP level along the PEC.

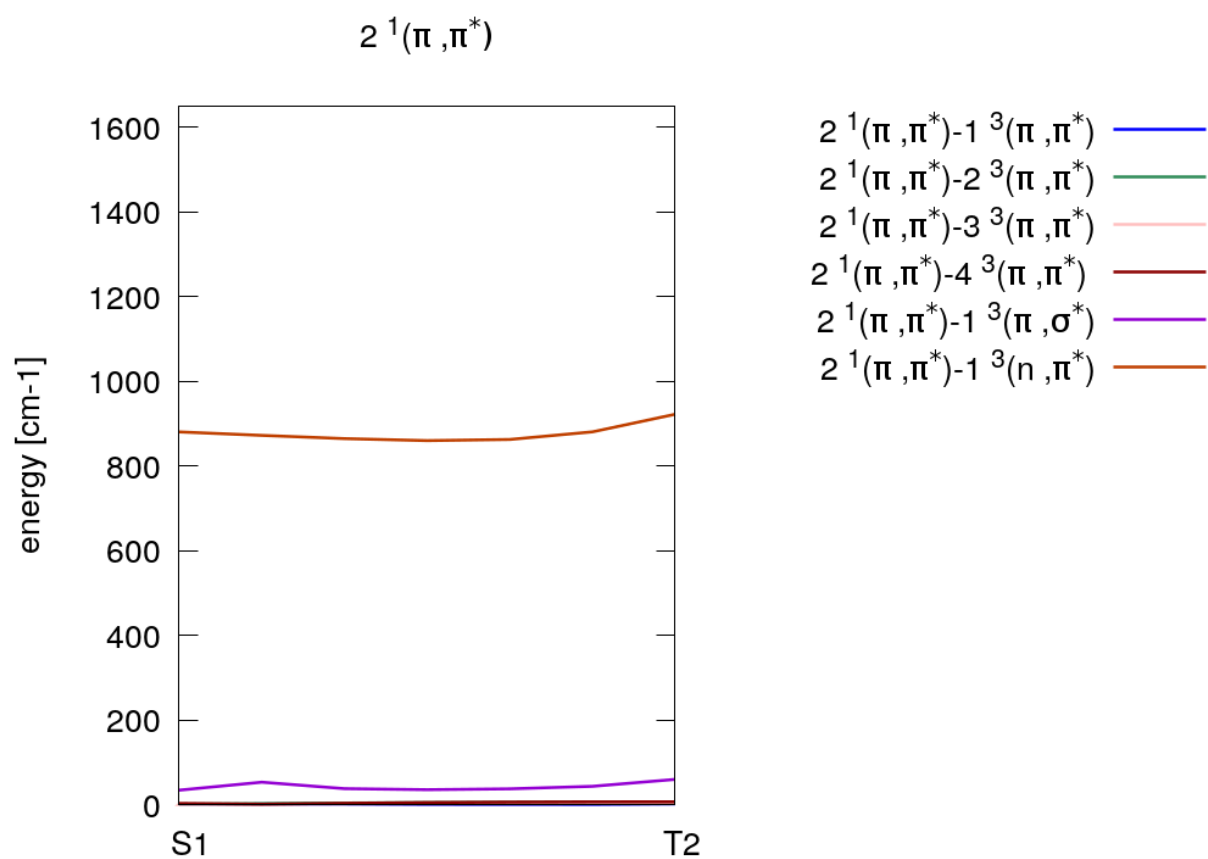

**Figure S17.** SOCs between excited state  $2^1(\pi, \pi^*)$  and 6 triplets at TD-DFT(TDA)/B3LYP/dhf-TZVP level along the PEC.

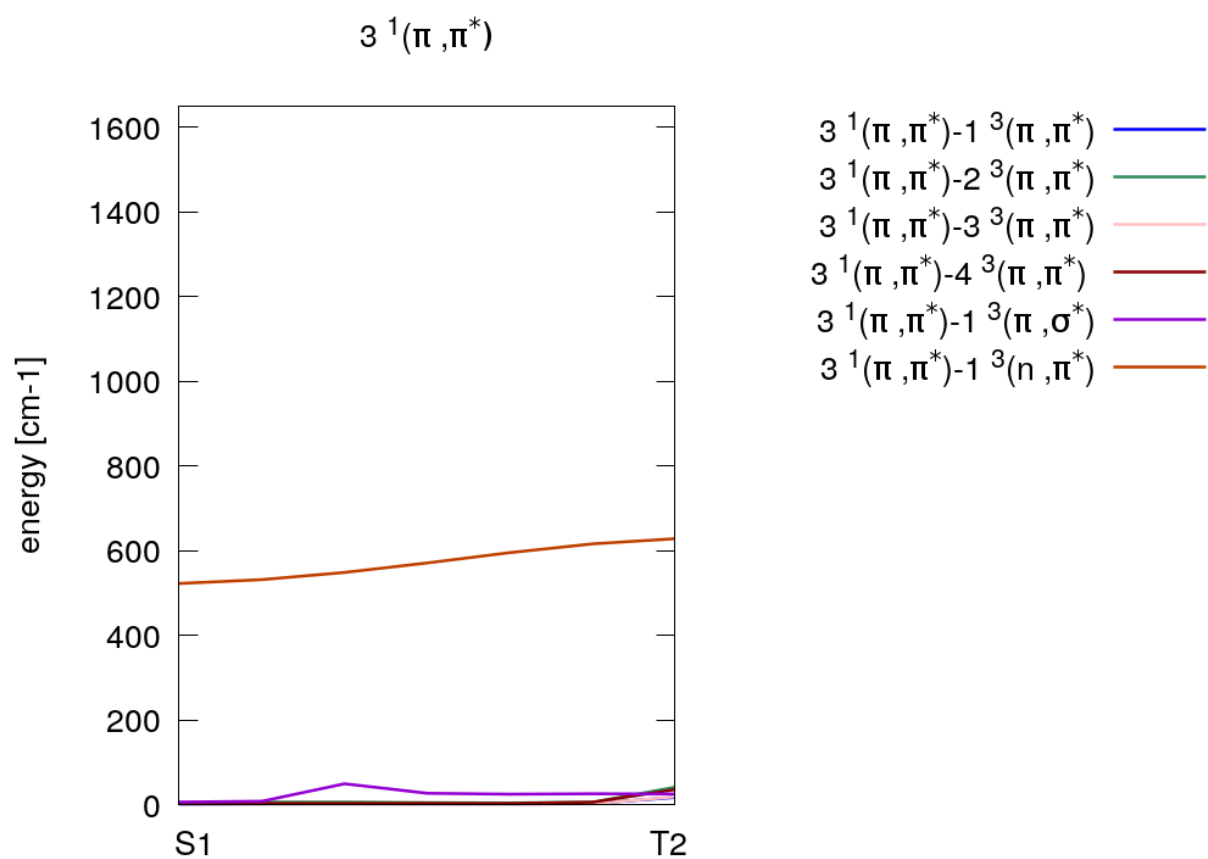

**Figure S18.** SOCs between excited state  $3^1(\pi, \pi^*)$  and 6 triplets at TD-DFT(TDA)/B3LYP/dhf-TZVP level along the PEC.



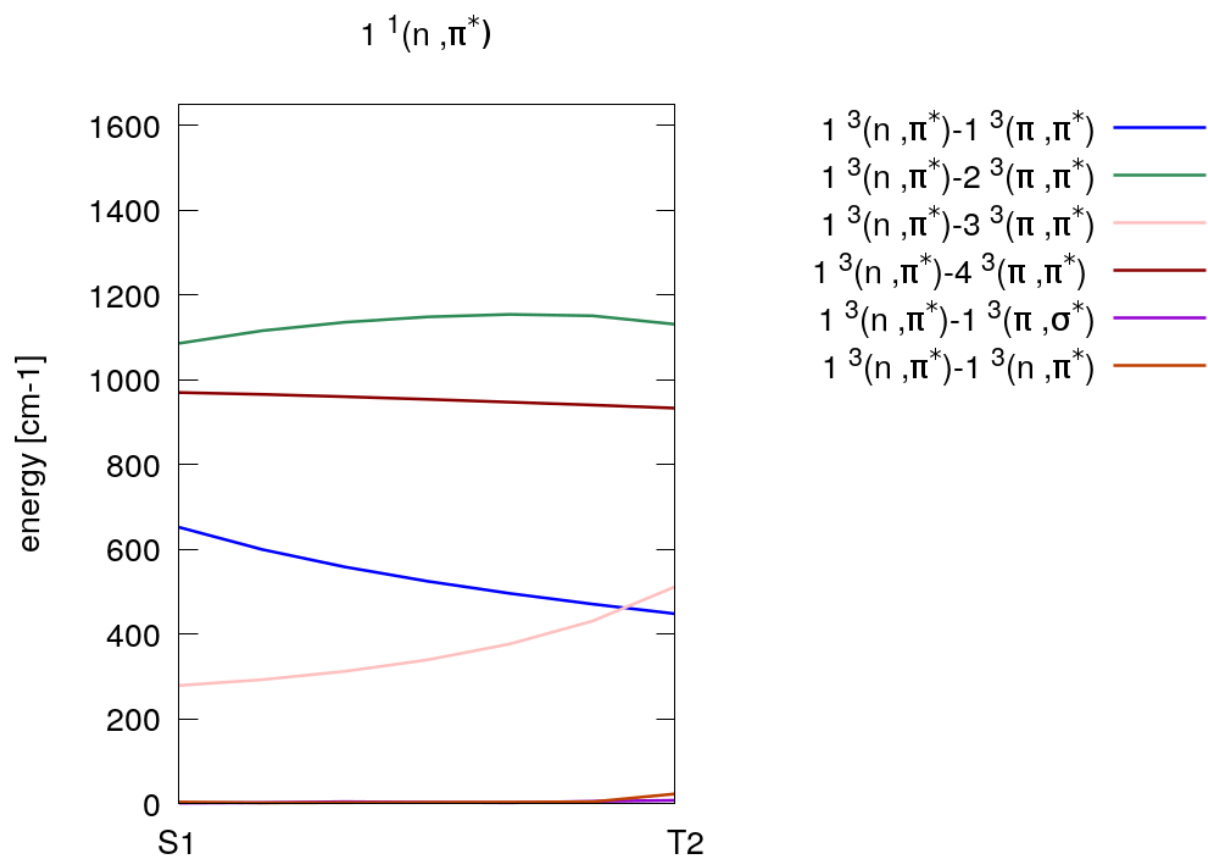

**Figure S19.** SOCs between excited state  $1^1(n, \pi^*)$  and 6 triplets at TD-DFT(TDA)/B3LYP/dhf-TZVP level along the PEC.



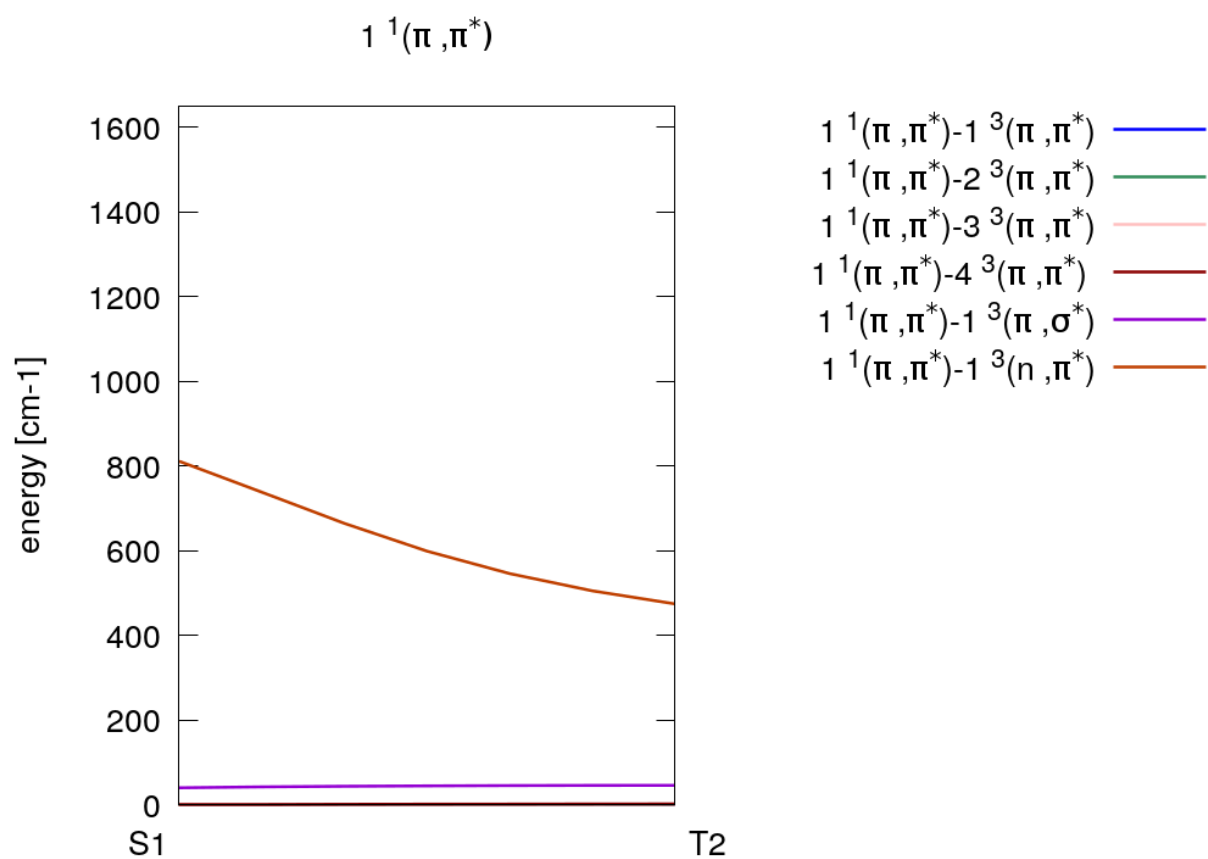

**Figure S21.** SOCs between excited state  $1^1(\pi, \pi^*)$  and 6 triplets at TD-DFT/BHLYP/dhf-TZVP level along the PEC.

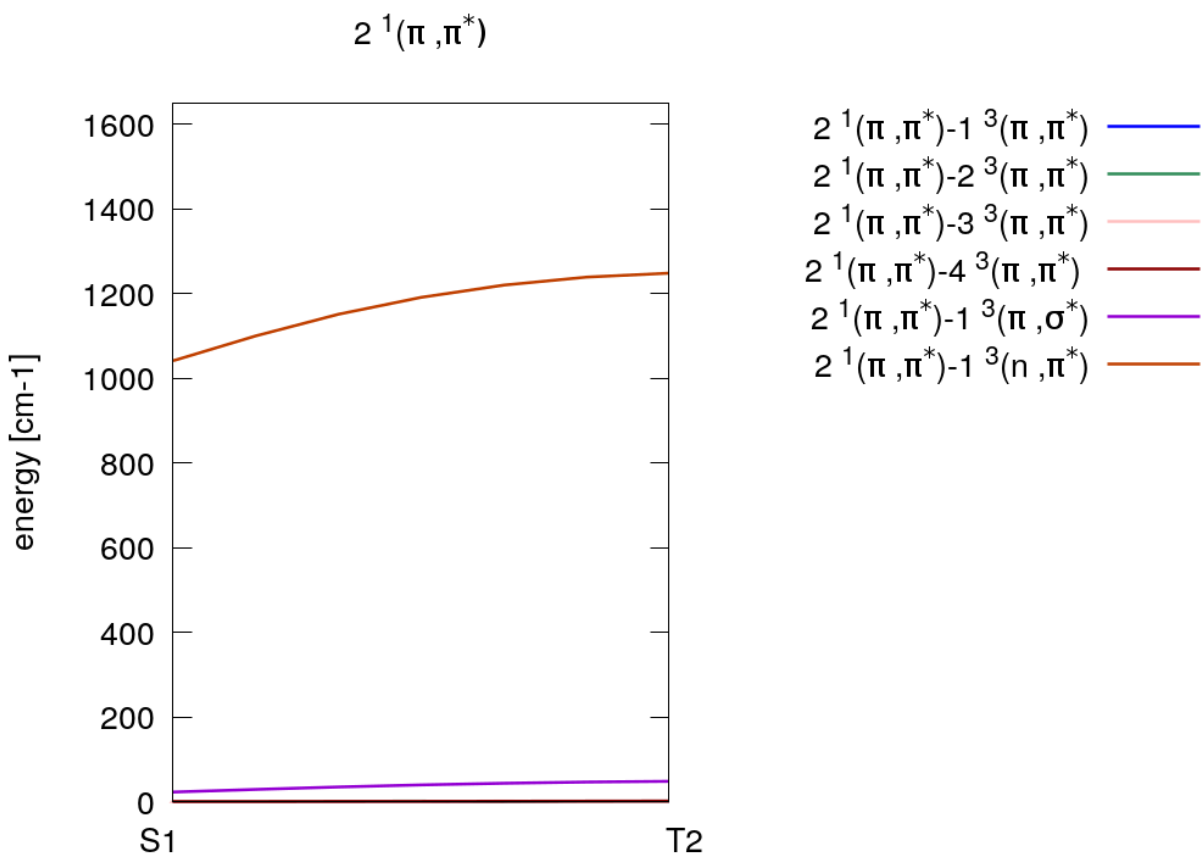

**Figure S22.** SOCs between excited state  $2^1(\pi, \pi^*)$  and 6 triplets at TD-DFT(TDA)/BHLYP/dhf-TZVP level along the PEC.

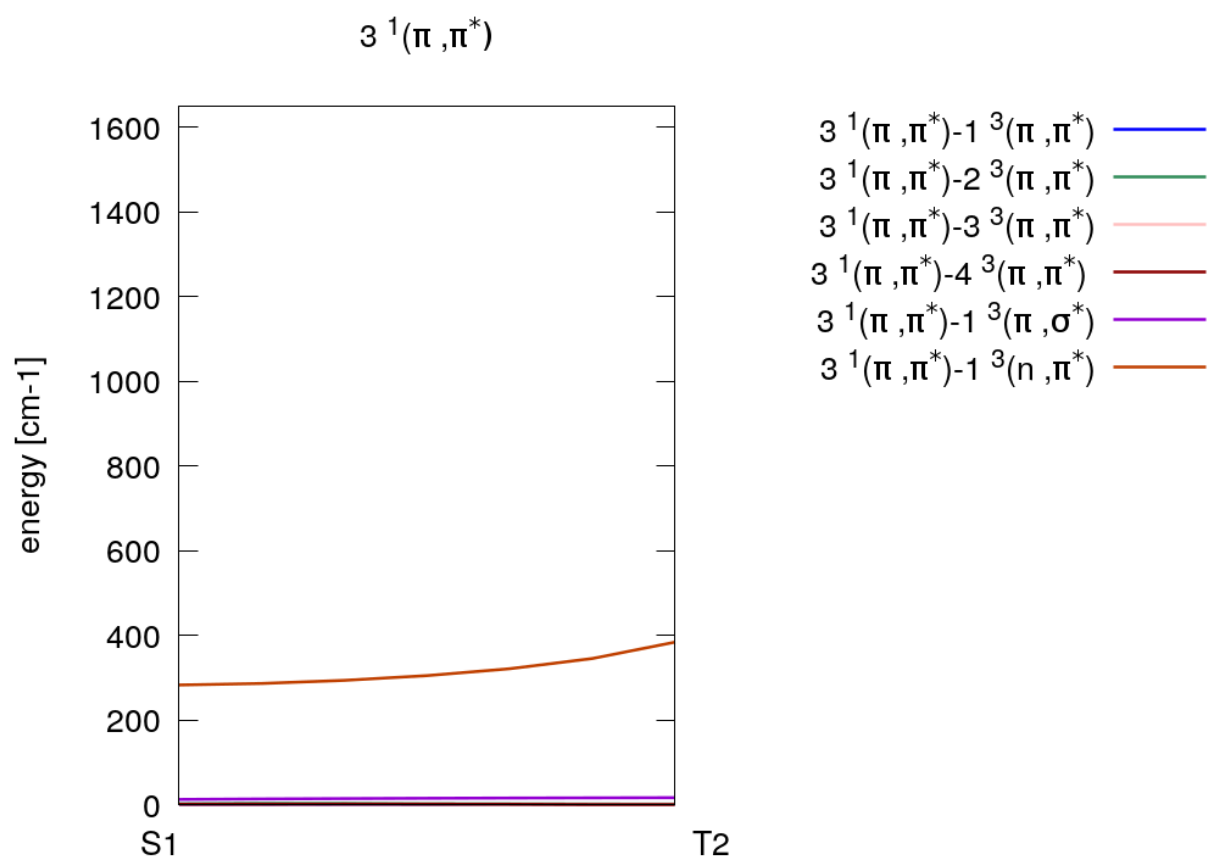

**Figure S23.** SOCs between excited state  $3^1(\pi, \pi^*)$  and 6 triplets at TD-DFT(TDA)/BHLYP/dhf-TZVP level along the PEC.

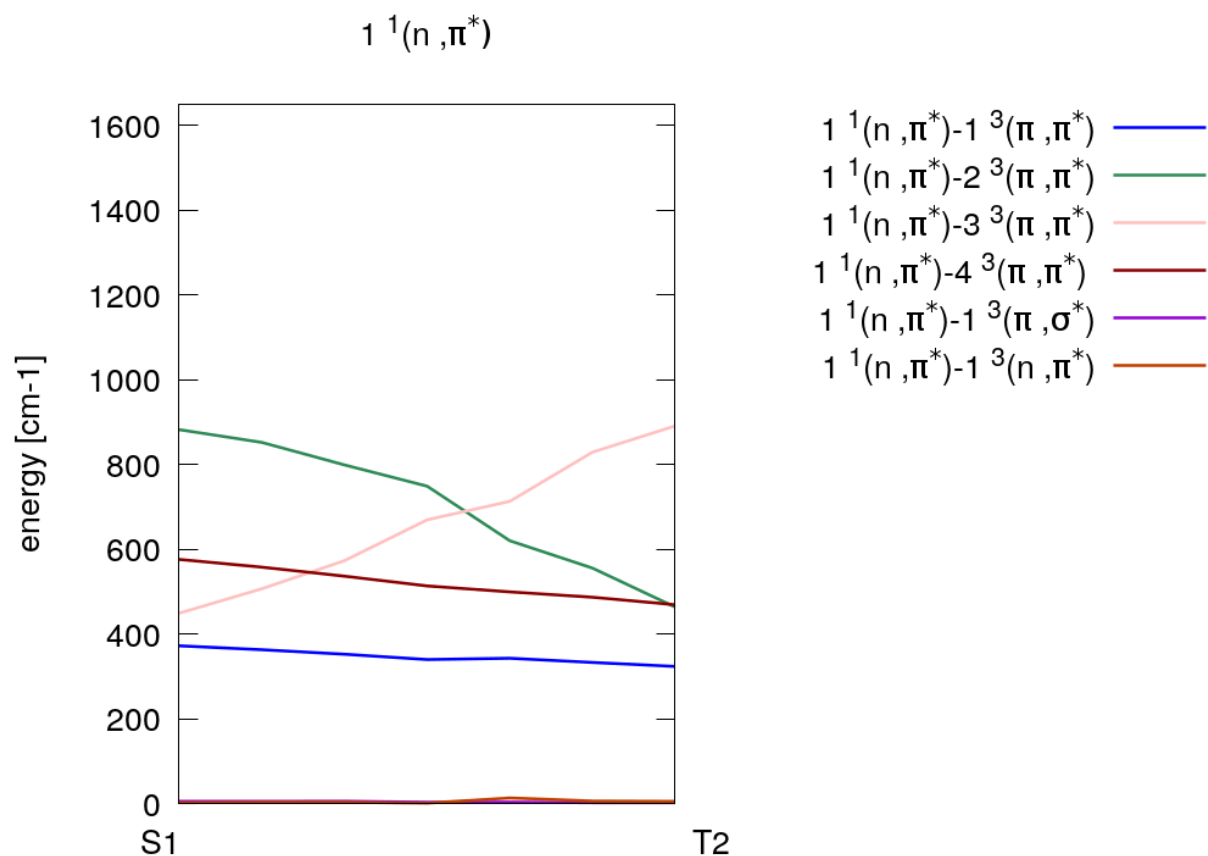

**Figure S24.** SOC between excited state  $1^1(n, \pi^*)$  and 6 triplets at TD-DFT(TDA)/BHLYP/dhf-TZVP level along the PEC.

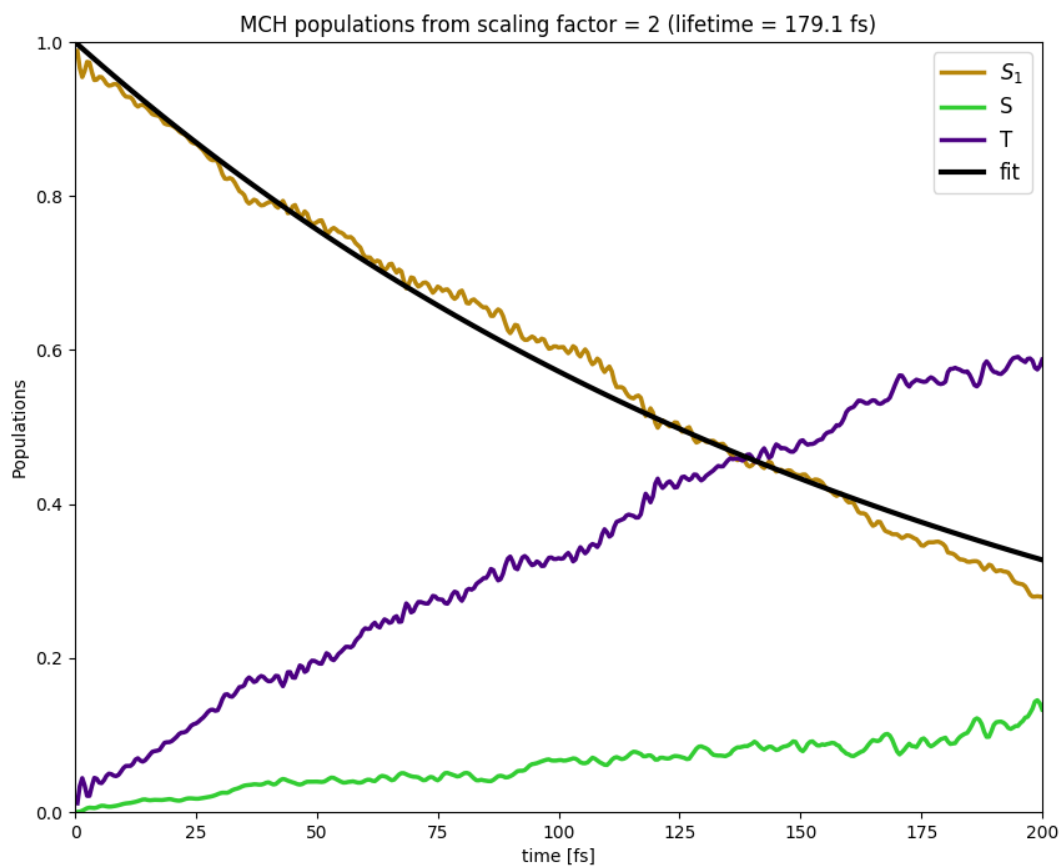

**Figure S25.** Time evolution of populations of singlets and triplets in I-BODIPY for excited state dynamics started in excited state  $S_1$  using scaling factor 2

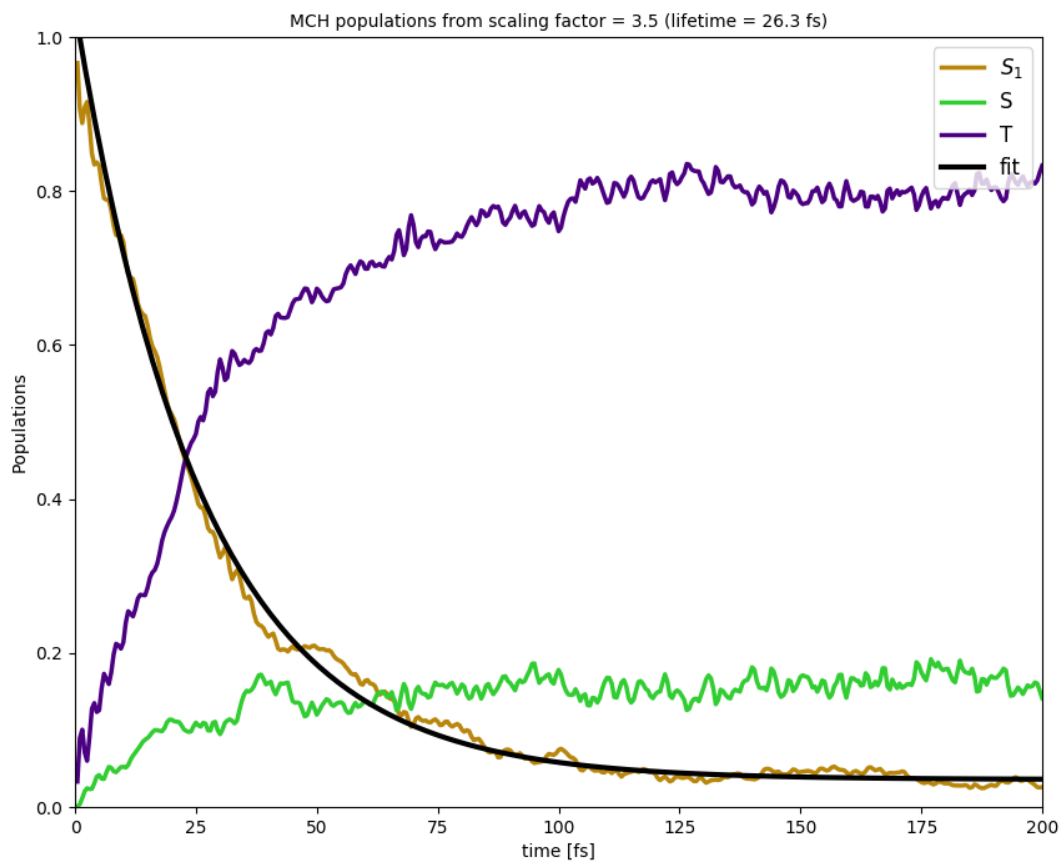

**Figure S26.** Time evolution of populations of singlets and triplets in I-BODIPY for excited state dynamics started in excited state  $S_1$  using scaling factor 3.5



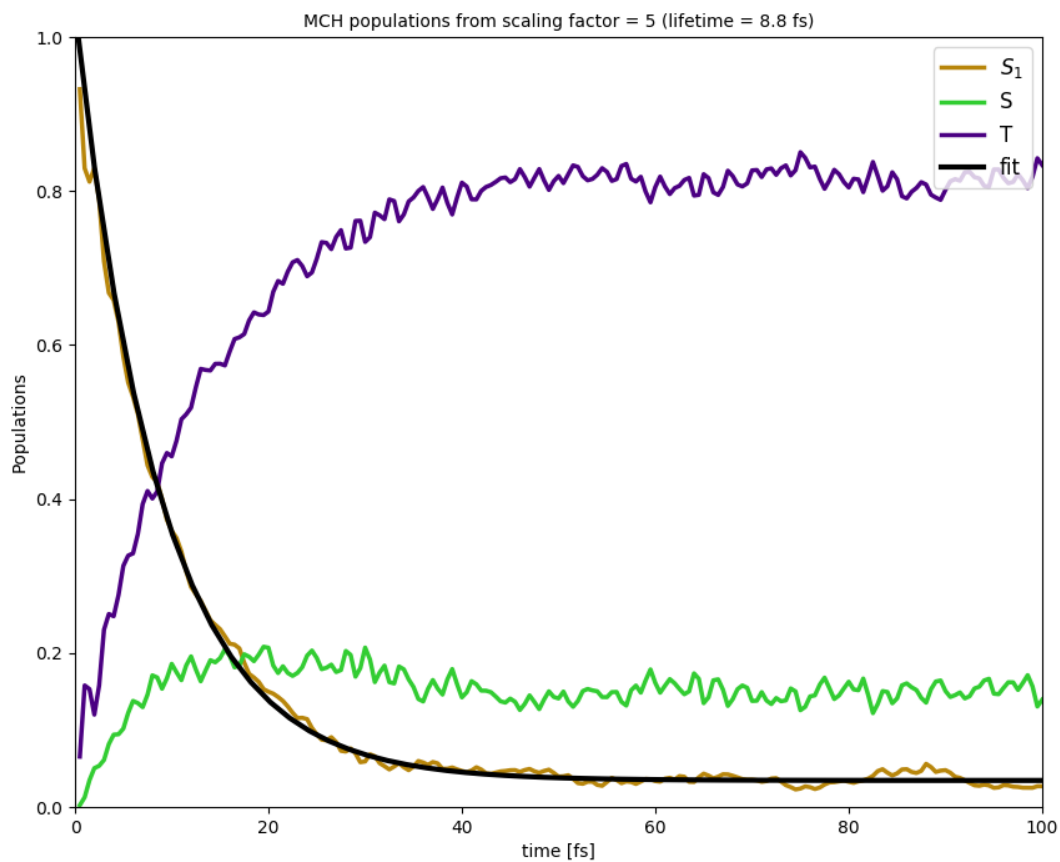

**Figure S27.** Time evolution of populations of singlets and triplets in I-BODIPY for excited state dynamics started in excited state  $S_1$  using scaling factor 5

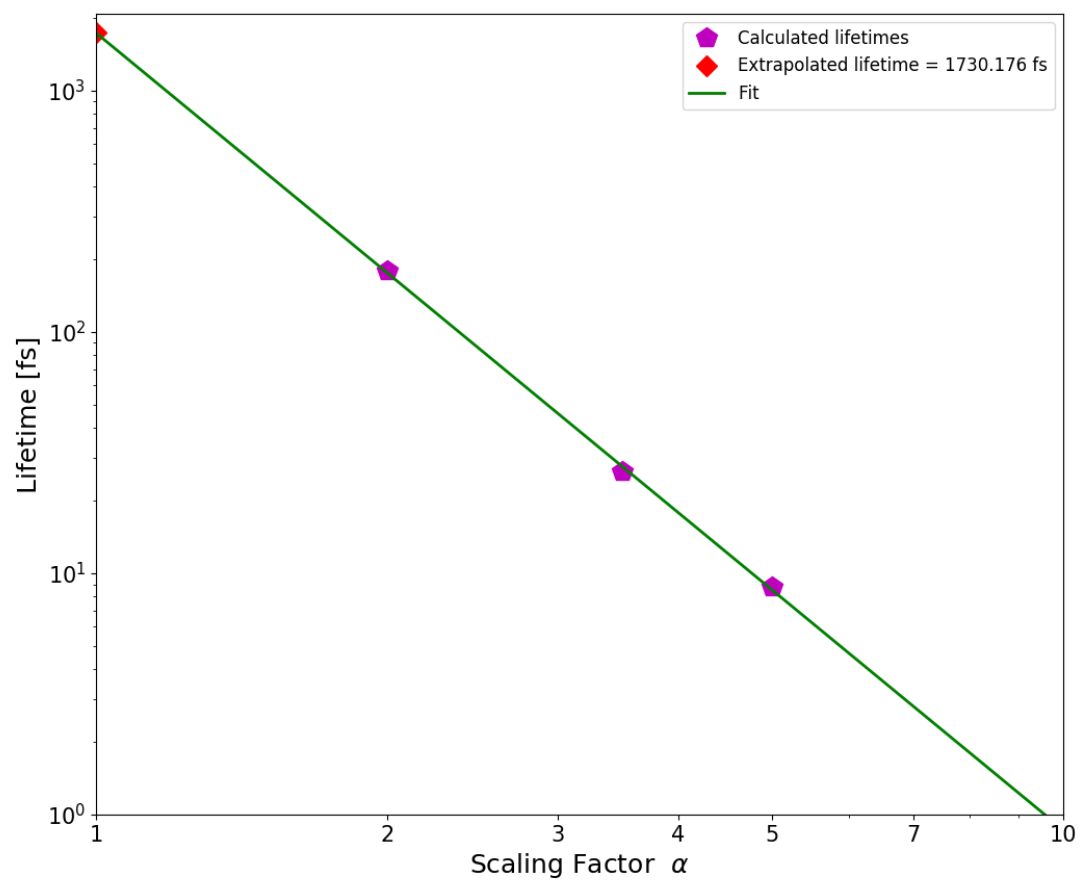

**Figure S28.** Extrapolation of the lifetime of the  $S_1$  state to unit scaling factor

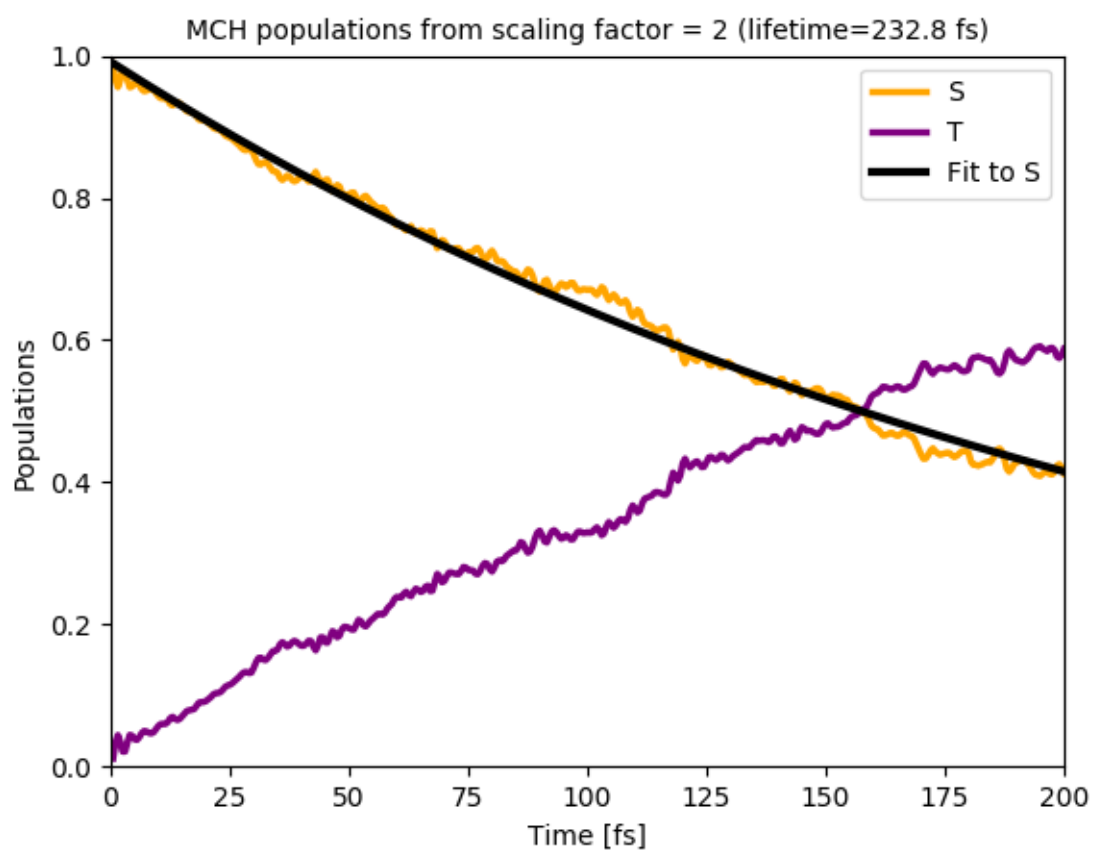

**Figure S29.** Time evolution of populations of singlets and triplets in I-BODIPY for excited state dynamics started in excited state  $S_1$  using scaling factor 2

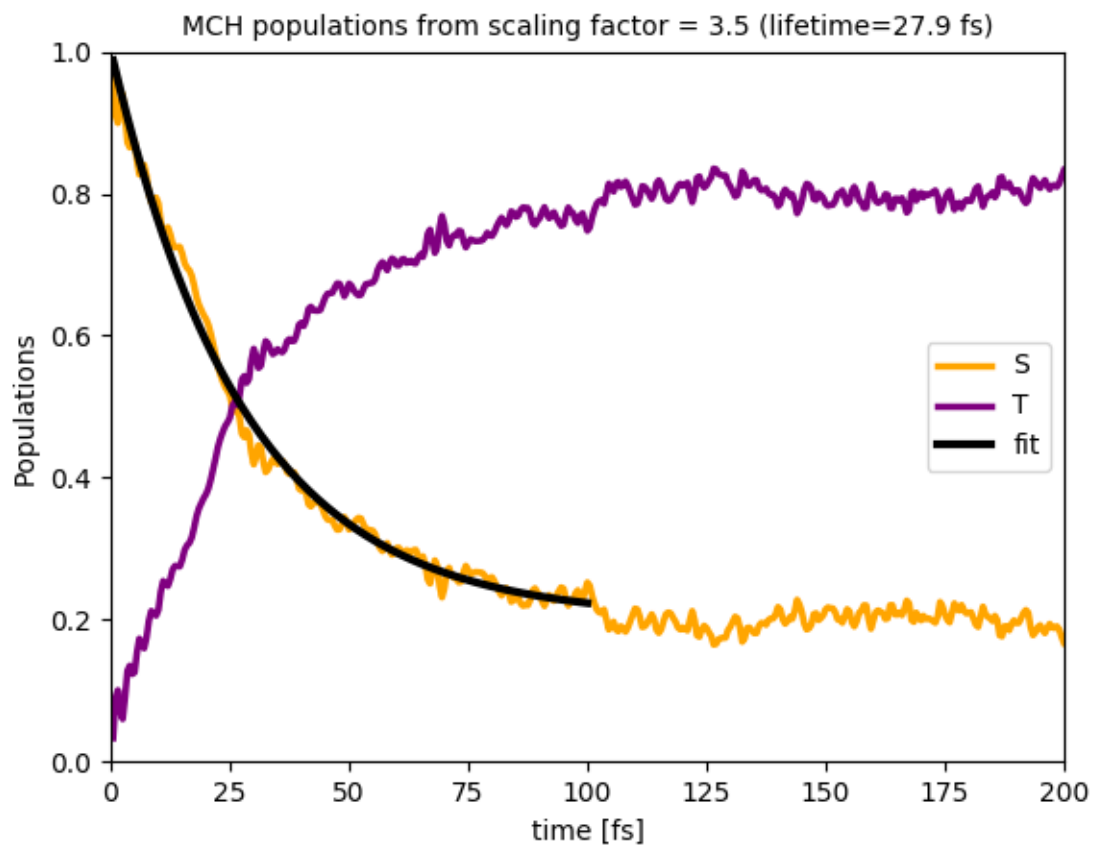

**Figure S30.** Time evolution of populations of singlets and triplets in I-BODIPY for excited state dynamics started in excited state  $S_1$  using scaling factor 3.5

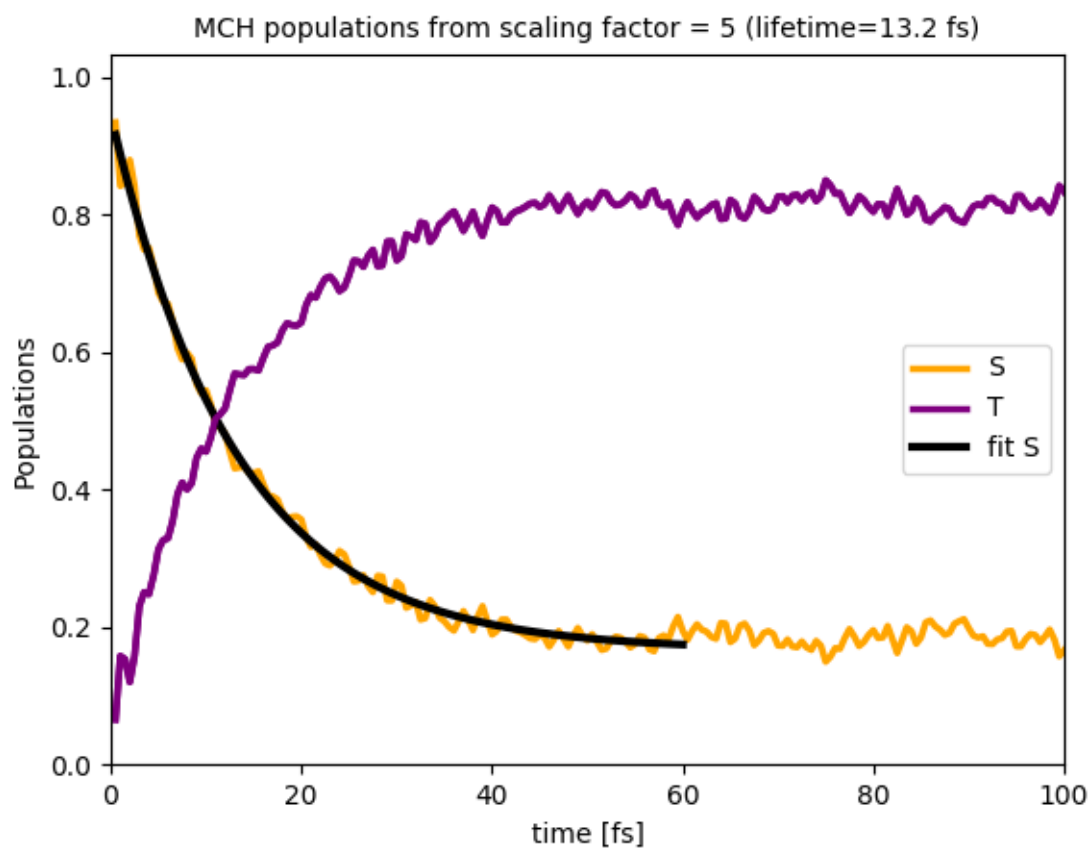

**Figure S31.** Time evolution of populations of singlets and triplets in I-BODIPY for excited state dynamics started in excited state  $S_1$  using scaling factor 5

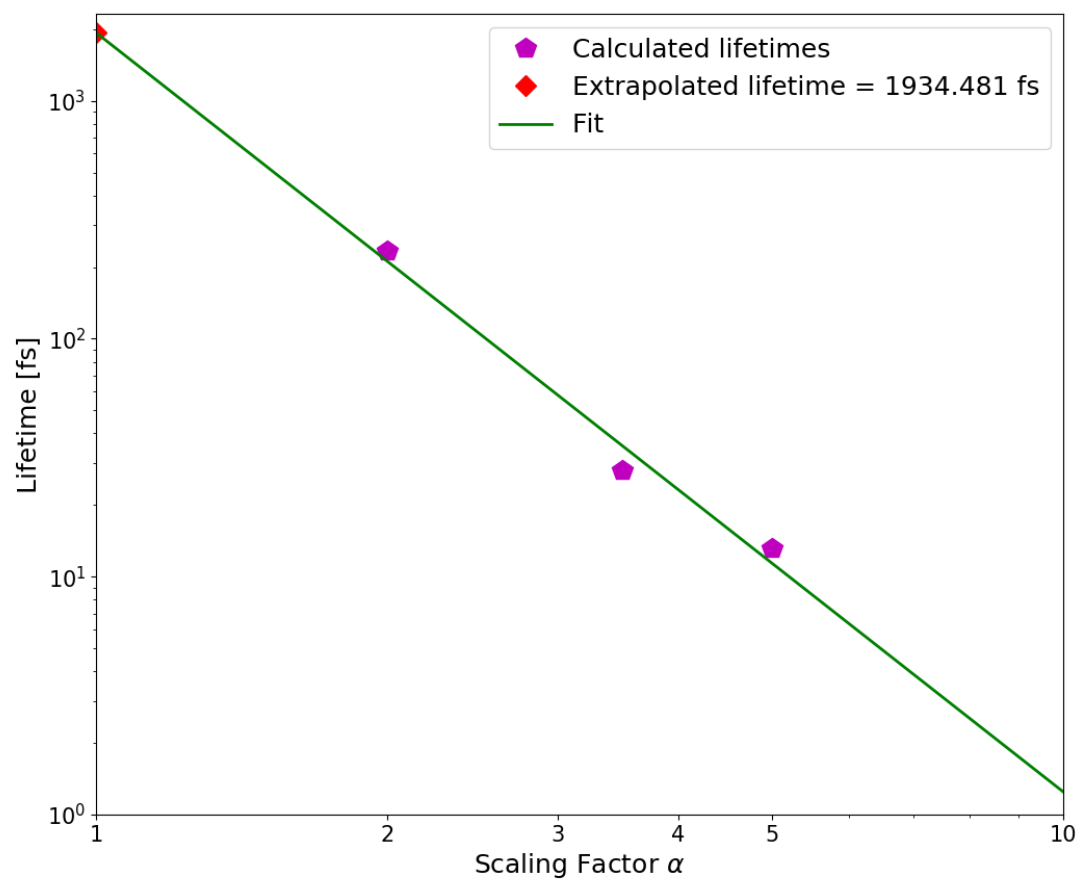

**Figure S32.** Extrapolation of the lifetime of the total singlet population to unit scaling factor

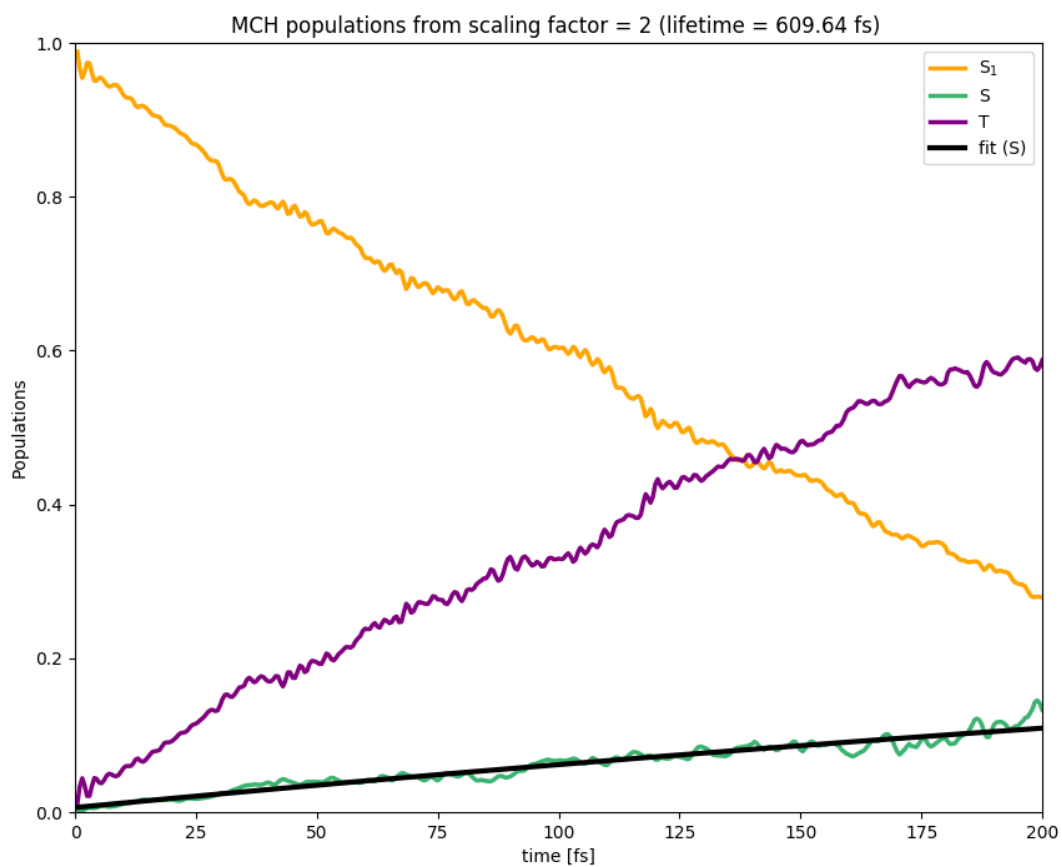

**Figure S33.** Time evolution of populations of singlets and triplets in I-BODIPY for excited state dynamics started in excited state  $S_1$  using scaling factor 2

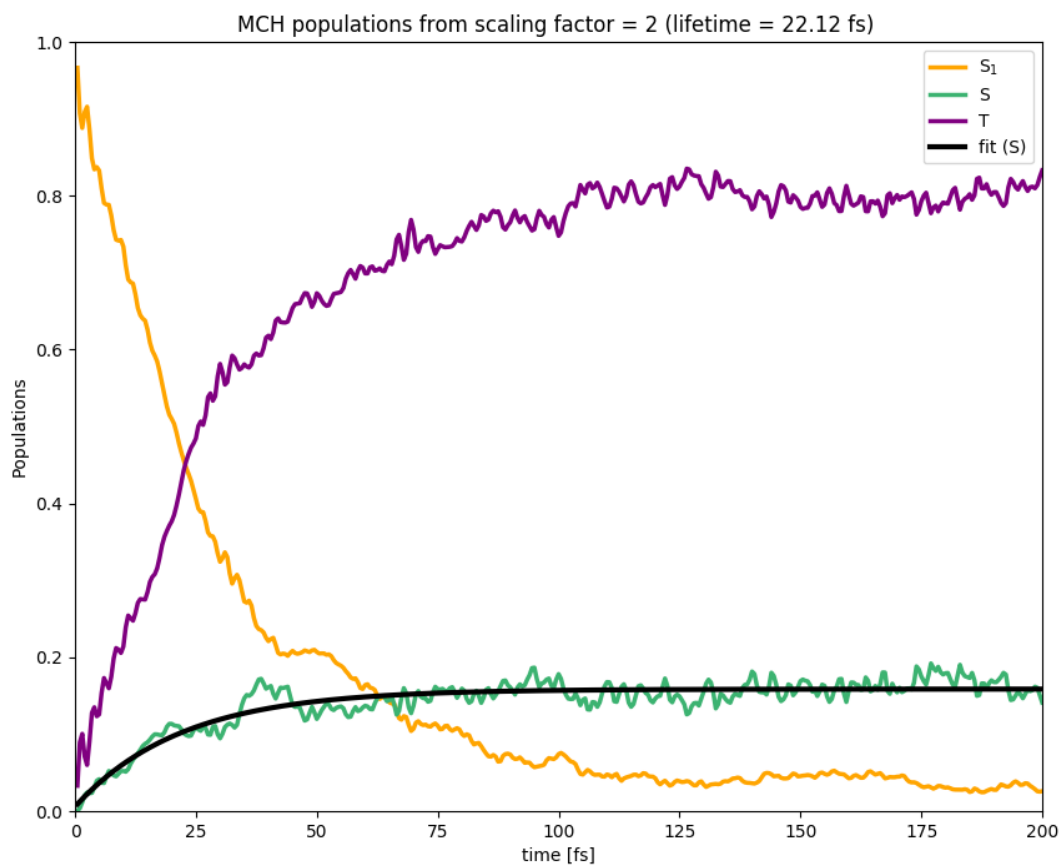

**Figure S34.** Time evolution of populations of singlets and triplets in I-BODIPY for excited state dynamics started in excited state  $S_1$  using scaling factor 3.5



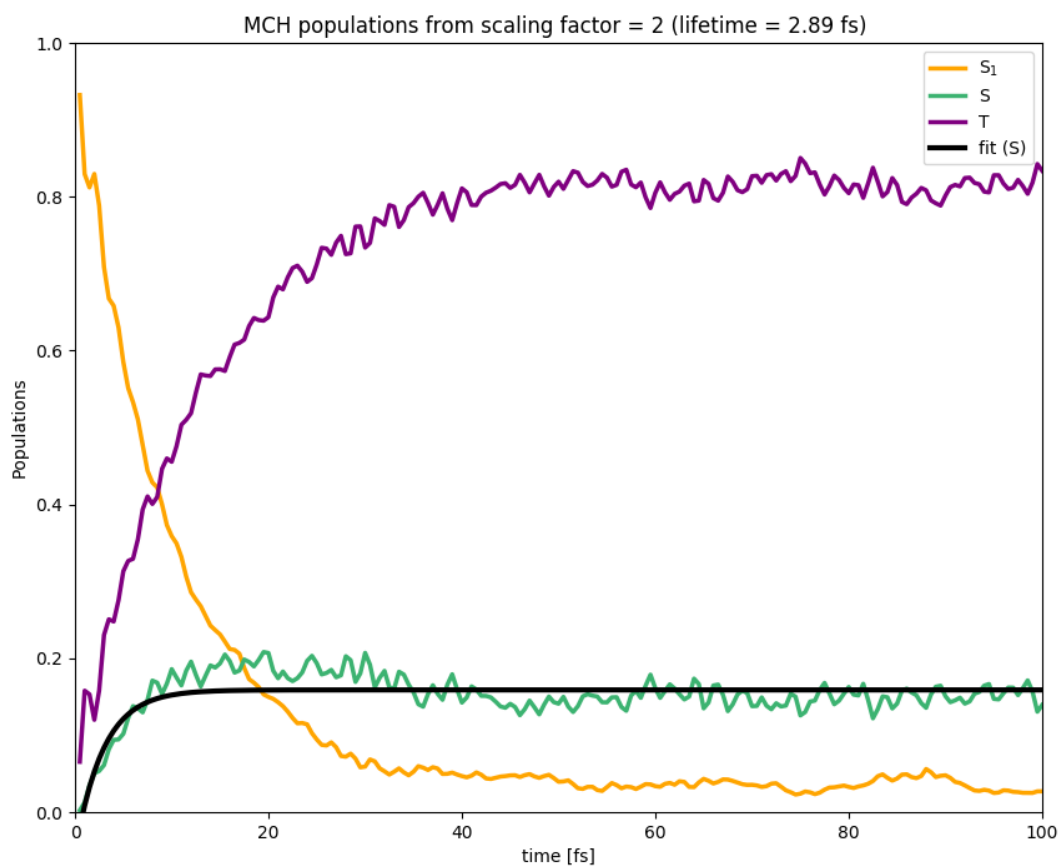

**Figure S35.** Time evolution of populations of singlets and triplets in I-BODIPY for excited state dynamics started in excited state  $S_1$  using scaling factor 5

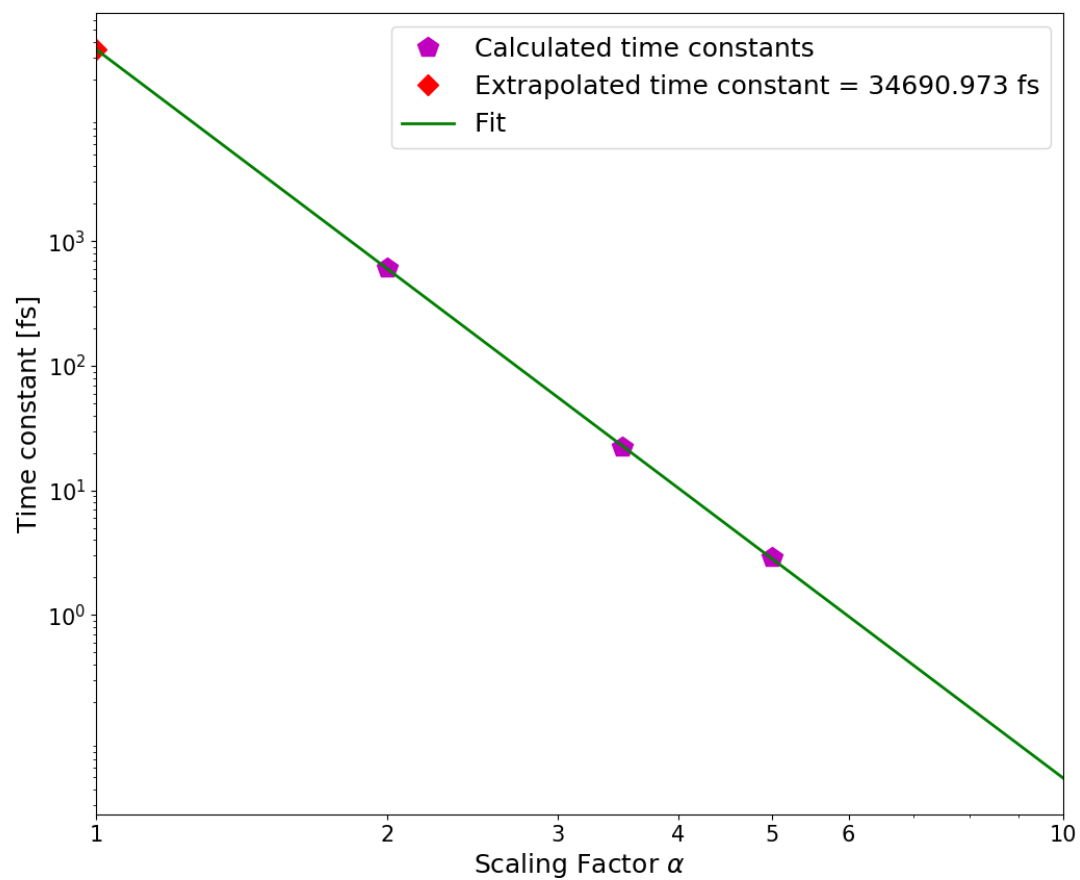

**Figure S36.** Extrapolation of the time constant of the overall singlet population except  $S_1$  to unit scaling factor

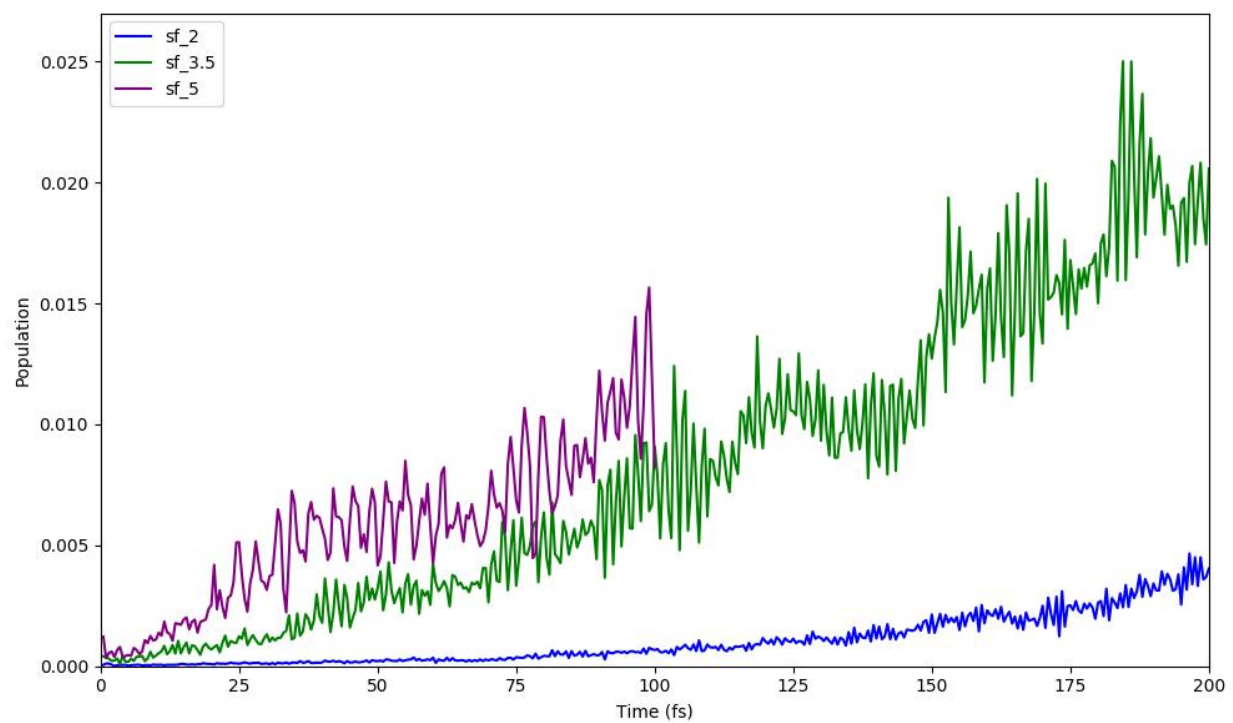

**Figure S37.** Evolution of populations  $S_0$  for all three scaling factors (sf) over the entire simulation time.

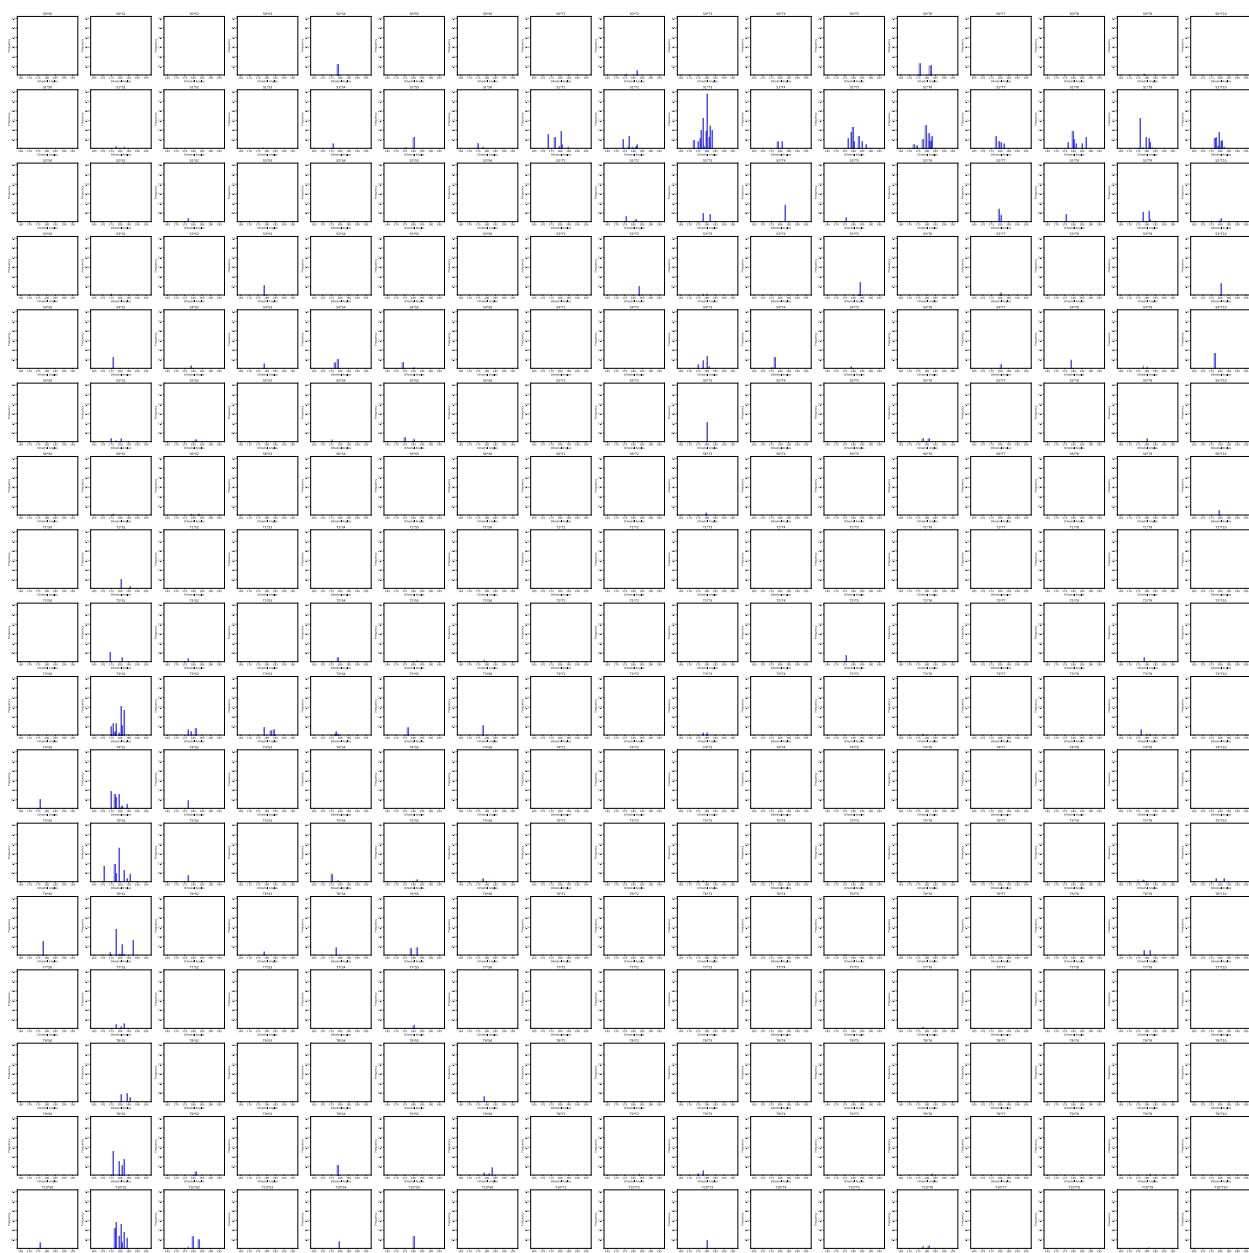

**Figure S38.** Matrix of histograms showing the fractional frequencies of transitions between all pairs of states (rows and columns ordered as  $S_0$ - $S_6$ ,  $T_1$ - $T_{10}$ ) as a function of the dihedral angle (see text for details)

**Table S22.** Fluorescence emission energy [eV] from electronic excited state S<sub>1</sub> to ground electronic state S<sub>0</sub> in I-BODIPY

| States                                          | Fluorescence emission energy<br>[eV]<br>( $E_F$ ) | Oscillator Strength ( $f$ ) |
|-------------------------------------------------|---------------------------------------------------|-----------------------------|
| S <sub>1</sub> $\longrightarrow$ S <sub>0</sub> | 2.25                                              | 0.06                        |

Rate constant for fluorescence is mathematically defined as;

$$k_F = \frac{2\pi e^2 E_F^2}{h^2 \epsilon_0 m c^3} f$$

**Table S23.** Rate constants for all possible radiative and non-radiative photochemical processes for I-BODIPY

| Photochemical phenomenon                                                                                      | Rate constant (s <sup>-1</sup> ) | Method Employed                                          |
|---------------------------------------------------------------------------------------------------------------|----------------------------------|----------------------------------------------------------|
| Intersystem Crossing from excited state S <sub>1</sub>                                                        | 1.65×10 <sup>11</sup>            | Trajectory Surface Hopping Method<br>( $k_{ISC}^{TSH}$ ) |
| Internal Conversion from excited state S <sub>1</sub> to all other singlets (S <sub>0</sub> -S <sub>6</sub> ) | 2.88×10 <sup>10</sup>            | Trajectory Surface Hopping Method<br>( $k_{IC}^{TSH}$ )  |
| Emissive decay from excited state S <sub>1</sub> to ground state S <sub>0</sub>                               | 1.32×10 <sup>7</sup>             | $k_F = \frac{2\pi e^2 E_F^2}{h^2 \epsilon_0 m c^3} f$    |

**Table S24.** Leading and second leading CASCI weights in the ground states of some planar unsaturated molecules calculated for state-specific CASSCF natural orbitals using the TZP contracted ANO-RCC basis set.

| Molecule                          | Active Space | Leading Weight | Second Leading Weight |
|-----------------------------------|--------------|----------------|-----------------------|
| BODIPY                            | (6,4)        | 0.9710         | 0.0170                |
|                                   | (12,11)      | 0.8394         | 0.0159                |
| Monoiodinated BODIPY (Position 2) | (6,4)        | 0.9707         | 0.0199                |
|                                   | (12,11)      | 0.8382         | 0.0161                |
|                                   | (16,14)      | 0.8205         | 0.0151                |
| Pyrrole                           | (6,5)        | 0.9339         | 0.0194                |
| 2-Iodopyrrole                     | (6,5)        | 0.9338         | 0.0190                |
|                                   | (10,8)       | 0.9143         | 0.0183                |
| Benzene                           | (6,6)        | 0.8886         | 0.0268                |
| Fulvene                           | (6,6)        | 0.8730         | 0.0234                |
| Naphtalene                        | (10,10)      | 0.8162         | 0.0195                |
| Azulene                           | (10,10)      | 0.7715         | 0.0300                |
| Anthracene                        | (14,14)      | 0.7404         | 0.0188                |
| Fluorene                          | (12,12)      | 0.7889         | 0.0174                |
| Phenalene                         | (12,12)      | 0.7798         | 0.0150                |

**Table S25.** Orbital entropies in monoiodinated BODIPY computed by DMRG.

| Orbital entropies computed by DMRG |
|------------------------------------|
| 0.00773208                         |
| 0.03760542                         |
| 0.00848550                         |
| 0.00661217                         |
| 0.00927742                         |
| 0.00895513                         |
| 0.04985414                         |
| 0.00442448                         |
| 0.00575732                         |
| 0.06601696                         |
| 0.11877988                         |
| 0.13721921                         |
| 0.12890688                         |
| 0.01368032                         |
| 0.11684634                         |
| 0.24945763                         |
| 0.29726541                         |
| 0.07475163                         |
| 0.00631764                         |
| 0.18092810                         |
| 0.00423184                         |
| 0.00426829                         |
| 0.13467771                         |
| 0.00474474                         |
| 0.00557975                         |
| 0.00379389                         |
| 0.12413380                         |
| 0.00630708                         |
| 0.03729784                         |
| 0.01836661                         |



**Table S26.** Orbital entropies in I-BODIPY computed by DMRG.

| Orbital entropies computed by DMRG |
|------------------------------------|
| 0.01167575                         |
| 0.01108050                         |
| 0.01904563                         |
| 0.01845215                         |
| 0.00621430                         |
| 0.01170264                         |
| 0.01115083                         |
| 0.02694420                         |
| 0.00889872                         |
| 0.01251517                         |
| 0.02629546                         |
| 0.02503590                         |
| 0.02861417                         |
| 0.05353056                         |
| 0.01867683                         |
| 0.08298607                         |
| 0.08727715                         |
| 0.13156104                         |
| 0.01876879                         |
| 0.09950085                         |
| 0.01964089                         |
| 0.11631518                         |
| 0.09400009                         |
| 0.24359040                         |
| 0.28950457                         |
| 0.09950810                         |
| 0.00967959                         |
| 0.08059509                         |
| 0.01786873                         |
| 0.13357890                         |
| 0.06745873                         |
| 0.02839748                         |
| 0.05850051                         |
| 0.08485443                         |
| 0.00619368                         |
| 0.02810880                         |
| 0.01354781                         |
| 0.06660888                         |
| 0.01369278                         |
| 0.02804484                         |
| 0.02551423                         |
| 0.01355629                         |
| 0.01428985                         |
| 0.03795330                         |
| 0.02676967                         |
| 0.03306580                         |

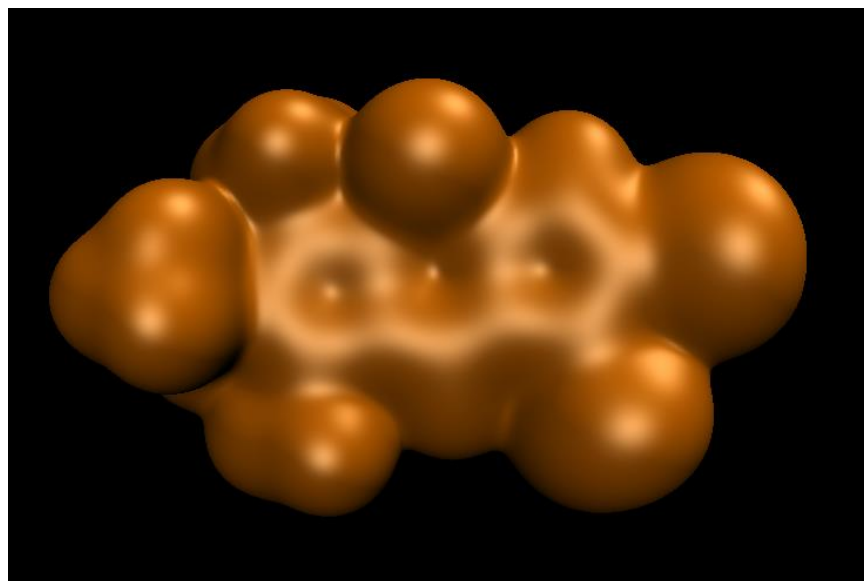

**Figure S39.** Electron density of ground state  $S_0$  computed at sf-X2C-S-TD-DFT/B3LYP/x2c-TZVPPall level for Br-BODIPY

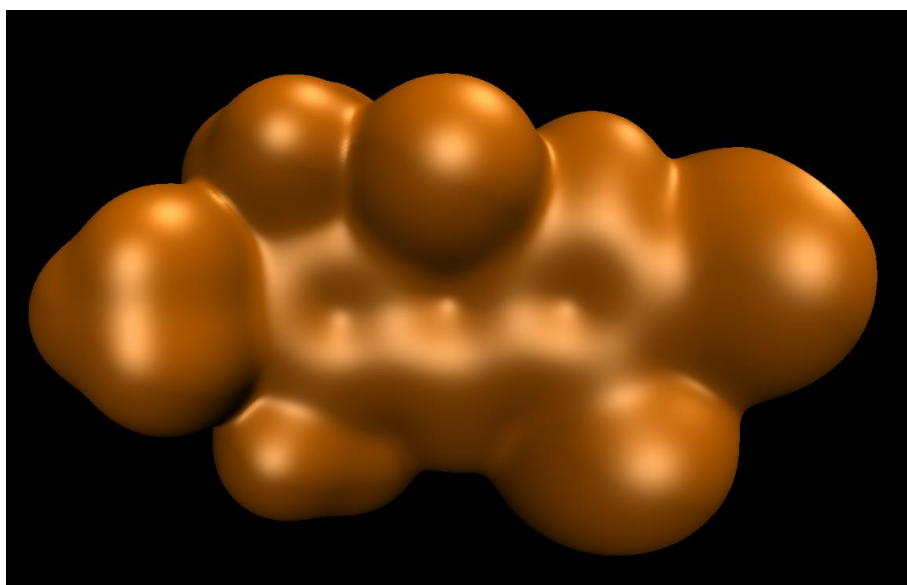

**Figure S40.** Electron density of ground state  $S_0$  computed at sf-X2C-S-TD-DFT/B3LYP/x2c-TZVPPall level for I-BODIPY

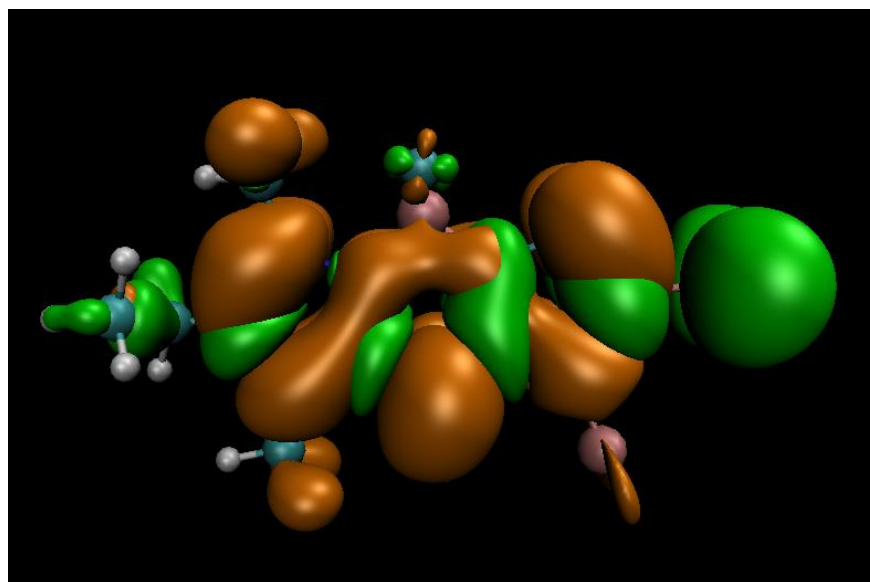

**Figure S41.** Differential Electron density between excited state  $S_1$  and ground state  $S_0$  computed at sf-X2C-S-TD-DFT/B3LYP/x2c-TZVPPall level for Br-BODIPY

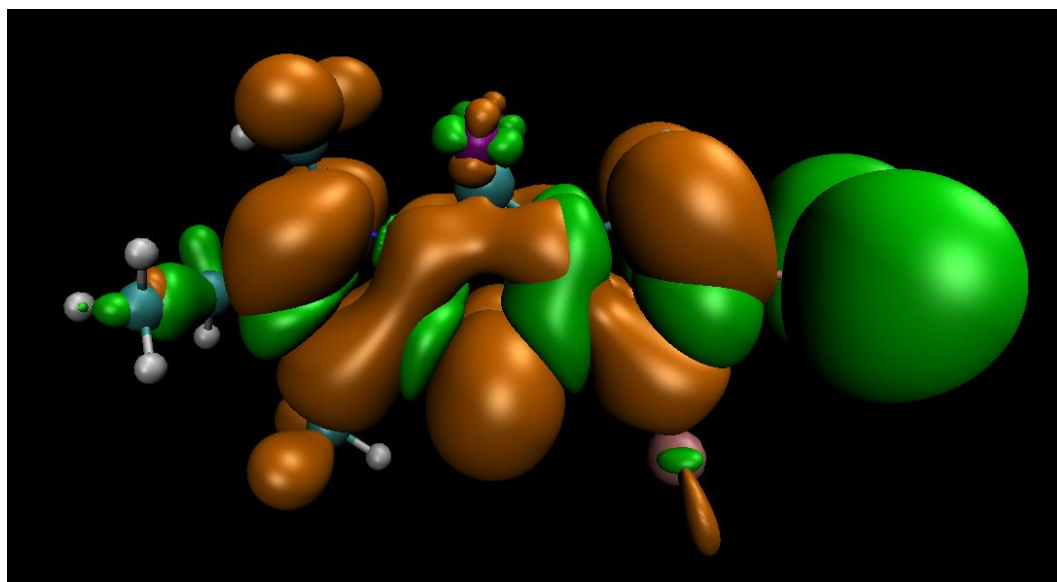

**Figure S42.** Differential Electron density between excited state  $S_1$  and ground state  $S_0$  computed at sf-X2C-S-TD-DFT/B3LYP/x2c-TZVPPall level for I-BODIPY

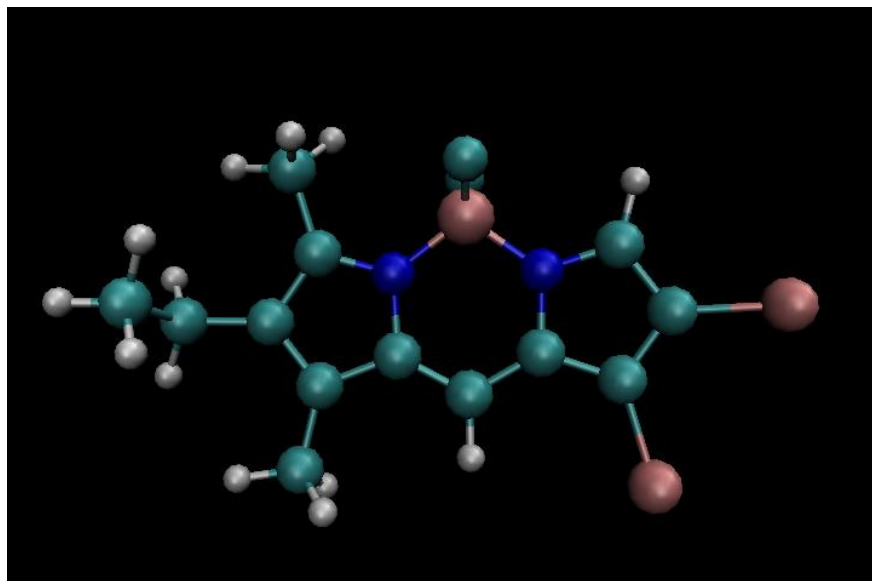

**Figure S43.** Optimized ground-state structure of Br-BODIPY

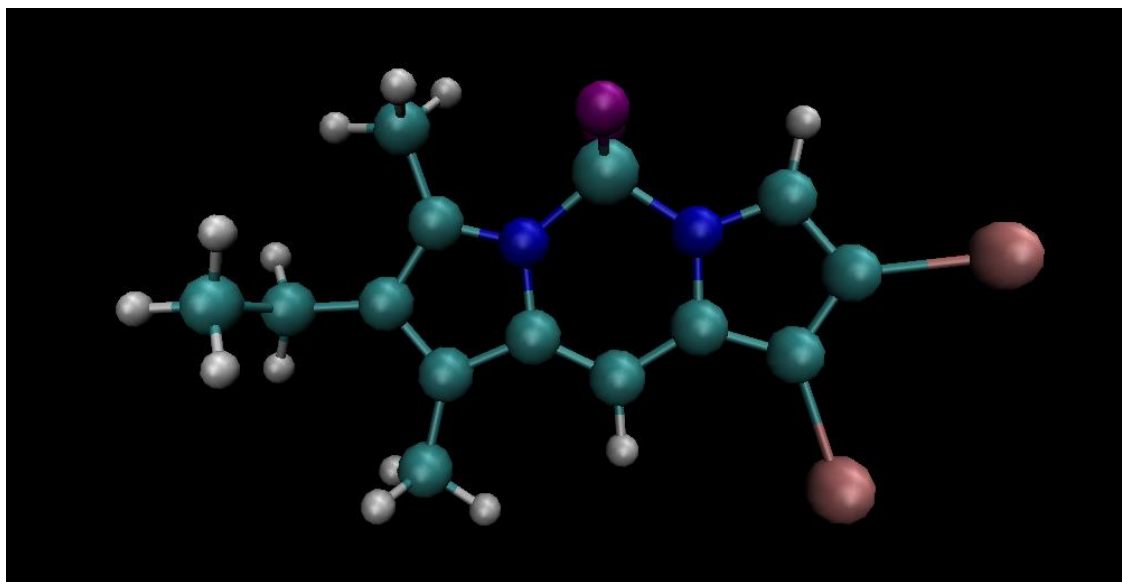

**Figure S44.** Optimized ground-state structure of I-BODIPY

**I-BODIPY S<sub>0</sub> optimized at TD-DFT/B3LYP/dhf-TZVP (-1428.75003134877 a.u.)**

|   |            |            |            |
|---|------------|------------|------------|
| C | 1.0310686  | 0.0026563  | -0.3128995 |
| C | -0.3840716 | 0.0761644  | -0.1380116 |
| N | -0.6564173 | 0.0322659  | 1.2297158  |
| C | 0.5067556  | -0.0593343 | 1.8839191  |
| C | 1.5853526  | -0.0848172 | 0.9527241  |
| C | -1.3993347 | 0.1794585  | -1.0577615 |
| C | -2.7396965 | 0.2512817  | -0.6715018 |
| C | -3.9295798 | 0.3421514  | -1.4296782 |
| C | -4.9890907 | 0.3706212  | -0.5187069 |
| C | -4.4220502 | 0.2981024  | 0.7610320  |
| N | -3.0883147 | 0.2285600  | 0.6675505  |
| I | -4.0148450 | 0.4121600  | -3.5083505 |
| B | -2.0832953 | 0.1339167  | 1.8687646  |
| F | -2.1657192 | 1.2774847  | 2.6511173  |
| I | -7.0385886 | 0.4930985  | -0.8758732 |
| C | 0.5785106  | -0.1004237 | 3.3680077  |
| C | 3.0398537  | -0.1347135 | 1.3058784  |
| C | 3.6029783  | 1.2408319  | 1.6947444  |
| F | -2.3644446 | -0.9996351 | 2.6196631  |
| H | 1.5723261  | -0.3893904 | 3.7047682  |
| H | 0.3425827  | 0.8846829  | 3.7798255  |
| H | -4.9214599 | 0.2932487  | 1.7160176  |
| H | -1.1667258 | 0.2066762  | -2.1132111 |
| H | 3.6043541  | -0.5311562 | 0.4581035  |
| H | 4.6628333  | 1.1743119  | 1.9488619  |
| H | 3.4920558  | 1.9504724  | 0.8723356  |
| H | 3.0721986  | 1.6499083  | 2.5567119  |
| H | 3.1989144  | -0.8372532 | 2.1289228  |
| H | -0.1597513 | -0.7957956 | 3.7684885  |
| C | 1.7597498  | 0.0286175  | -1.6154682 |
| H | 1.0787728  | 0.0082147  | -2.4656910 |
| H | 2.3742966  | 0.9285231  | -1.7036300 |
| H | 2.4314526  | -0.8284302 | -1.7063610 |

**I-BODIPY S<sub>0</sub> optimized at TD-DFT/B3LYP/aug-cc-pVDZ/aug-cc-pVDZ-PP  
(-1429.165398 a.u.)**

|   |           |           |           |
|---|-----------|-----------|-----------|
| C | 1.039148  | 0.003316  | -0.327268 |
| C | -0.382155 | 0.079785  | -0.153380 |
| N | -0.656011 | 0.052263  | 1.218436  |
| C | 0.510361  | -0.034239 | 1.879320  |
| C | 1.594282  | -0.068950 | 0.946567  |
| C | -1.404139 | 0.170759  | -1.077427 |
| C | -2.748481 | 0.242533  | -0.680002 |
| C | -3.949257 | 0.342506  | -1.431379 |
| C | -5.006140 | 0.380901  | -0.506250 |
| C | -4.425579 | 0.303658  | 0.775117  |
| N | -3.087790 | 0.222305  | 0.666338  |
| I | -4.049485 | 0.415874  | -3.523995 |
| B | -2.078737 | 0.113512  | 1.854499  |
| F | -2.190617 | 1.241793  | 2.681581  |
| I | -7.071553 | 0.524322  | -0.850323 |
| C | 0.574377  | -0.070072 | 3.367532  |
| C | 3.051646  | -0.123969 | 1.302982  |
| C | 3.610947  | 1.245328  | 1.730031  |
| F | -2.335097 | -1.055900 | 2.588523  |
| H | 1.590249  | -0.287116 | 3.711018  |
| H | 0.256038  | 0.898341  | 3.778997  |
| H | -4.917909 | 0.304217  | 1.741391  |
| H | -1.175365 | 0.189847  | -2.140670 |
| H | 3.620236  | -0.497928 | 0.440118  |
| H | 4.678088  | 1.174396  | 1.981122  |
| H | 3.494091  | 1.981448  | 0.922820  |
| H | 3.075923  | 1.628844  | 2.609526  |
| H | 3.209983  | -0.852113 | 2.112551  |
| H | -0.118513 | -0.824423 | 3.761190  |
| C | 1.772915  | 0.001819  | -1.632276 |
| H | 1.090669  | 0.071828  | -2.486921 |
| H | 2.474862  | 0.845980  | -1.691190 |
| H | 2.363683  | -0.918408 | -1.748570 |

**I-BODIPY S<sub>1</sub> optimized at TD-DFT/B3LYP/aug-cc-pVDZ/aug-cc-pVDZ-PP  
(-1429.155400 a.u.)**

|   |           |           |           |
|---|-----------|-----------|-----------|
| C | 1.056989  | 0.008523  | -0.313593 |
| C | -0.371234 | 0.097882  | -0.169584 |
| N | -0.667287 | 0.050424  | 1.204206  |
| C | 0.501044  | -0.063358 | 1.891642  |
| C | 1.589352  | -0.095822 | 0.974373  |
| C | -1.352472 | 0.212329  | -1.127391 |
| C | -2.742830 | 0.286532  | -0.713833 |
| C | -3.908913 | 0.401170  | -1.433359 |
| C | -5.012906 | 0.427567  | -0.437251 |
| C | -4.426811 | 0.326194  | 0.814437  |
| N | -3.081759 | 0.243236  | 0.639484  |
| I | -4.068919 | 0.514879  | -3.505626 |
| B | -2.062766 | 0.115504  | 1.829765  |
| F | -2.213692 | 1.239765  | 2.666777  |
| I | -7.028144 | 0.582307  | -0.804697 |
| C | 0.528575  | -0.128541 | 3.379201  |
| C | 3.039095  | -0.173560 | 1.356506  |
| C | 3.645644  | 1.207059  | 1.667379  |
| F | -2.372014 | -1.052785 | 2.555402  |
| H | 1.553315  | -0.237880 | 3.747390  |
| H | 0.087875  | 0.781738  | 3.811898  |
| H | -4.877008 | 0.308219  | 1.798343  |
| H | -1.105462 | 0.247893  | -2.182472 |
| H | 3.607305  | -0.647632 | 0.543832  |
| H | 4.706469  | 1.120956  | 1.941889  |
| H | 3.565932  | 1.869073  | 0.794129  |
| H | 3.111564  | 1.687379  | 2.498751  |
| H | 3.157511  | -0.829509 | 2.231305  |
| H | -0.078088 | -0.971073 | 3.741621  |
| C | 1.768382  | 0.036275  | -1.627827 |
| H | 1.438190  | -0.786126 | -2.282012 |
| H | 1.570176  | 0.974598  | -2.170049 |
| H | 2.853558  | -0.050758 | -1.500627 |

**I-BODIPY T<sub>2</sub> optimized at TD-DFT/B3LYP/aug-cc-pVDZ/aug-cc-pVDZ-PP  
(-1429.157633 a.u.)**

|   |           |           |           |
|---|-----------|-----------|-----------|
| C | 1.064983  | 0.002717  | -0.295870 |
| C | -0.384143 | 0.092645  | -0.117753 |
| N | -0.664395 | 0.053808  | 1.201935  |
| C | 0.542982  | -0.060385 | 1.907766  |
| C | 1.618507  | -0.094838 | 0.972719  |
| C | -1.401310 | 0.205936  | -1.109975 |
| C | -2.727130 | 0.278980  | -0.684839 |
| C | -3.960593 | 0.397832  | -1.443155 |
| C | -5.006215 | 0.430339  | -0.518883 |
| C | -4.430267 | 0.334120  | 0.765732  |
| N | -3.068004 | 0.244265  | 0.652213  |
| I | -4.039490 | 0.494725  | -3.528495 |
| B | -2.080263 | 0.122975  | 1.837390  |
| F | -2.177728 | 1.246409  | 2.681657  |
| I | -7.068809 | 0.588524  | -0.854828 |
| C | 0.560030  | -0.119818 | 3.389027  |
| C | 3.072356  | -0.171086 | 1.340193  |
| C | 3.661486  | 1.204191  | 1.701740  |
| F | -2.337385 | -1.046512 | 2.579037  |
| H | 1.581456  | -0.224164 | 3.766968  |
| H | 0.104585  | 0.789575  | 3.808506  |
| H | -4.920191 | 0.325637  | 1.732566  |
| H | -1.149739 | 0.234790  | -2.163485 |
| H | 3.637792  | -0.606266 | 0.505028  |
| H | 4.723190  | 1.118250  | 1.970095  |
| H | 3.573426  | 1.897984  | 0.854559  |
| H | 3.126025  | 1.647125  | 2.552599  |
| H | 3.201094  | -0.860231 | 2.187409  |
| H | -0.053506 | -0.961028 | 3.743219  |
| C | 1.727807  | 0.027203  | -1.632164 |
| H | 1.377657  | -0.804401 | -2.263715 |
| H | 1.489033  | 0.957013  | -2.172231 |
| H | 2.817433  | -0.043851 | -1.544956 |



**Br-BODIPY S<sub>0</sub> optimized at TD-DFT/B3LYP/aug-cc-pVDZ/aug-cc-pVDZ-PP  
( -1671.377451 a.u.)**

|    |           |           |           |
|----|-----------|-----------|-----------|
| C  | -3.773282 | 0.181774  | 0.787968  |
| N  | -2.440657 | 0.136357  | 0.623756  |
| C  | -2.167586 | 0.143250  | -0.748791 |
| C  | -3.415272 | 0.197951  | -1.452914 |
| C  | -4.417784 | 0.222950  | -0.488349 |
| B  | -1.370319 | 0.083988  | 1.758160  |
| F  | -1.553886 | -1.064687 | 2.543277  |
| C  | -0.866824 | 0.097620  | -1.210057 |
| C  | 0.219533  | 0.039746  | -0.324993 |
| N  | 0.020452  | 0.027599  | 1.048844  |
| C  | 1.217614  | -0.031775 | 1.660141  |
| C  | 2.240933  | -0.061033 | 0.694337  |
| C  | 1.616361  | -0.016011 | -0.559548 |
| Br | 4.087448  | -0.145955 | 1.075948  |
| Br | 2.431739  | -0.026589 | -2.257508 |
| C  | -3.592726 | 0.224562  | -2.939261 |
| C  | -5.901396 | 0.240462  | -0.717717 |
| C  | -6.542223 | -1.151302 | -0.568074 |
| C  | -4.403524 | 0.174355  | 2.138129  |
| F  | -1.449929 | 1.236892  | 2.555875  |
| H  | -5.480701 | 0.352956  | 2.068936  |
| H  | -4.230989 | -0.795419 | 2.626080  |
| H  | -2.633953 | 0.177810  | -3.467866 |
| H  | -4.206688 | -0.621909 | -3.278645 |
| H  | -4.106373 | 1.143913  | -3.256145 |
| H  | 1.308018  | -0.051137 | 2.740445  |
| H  | -0.663939 | 0.104097  | -2.278619 |
| H  | -6.106102 | 0.630719  | -1.724437 |
| H  | -7.625632 | -1.107531 | -0.744625 |
| H  | -6.103773 | -1.859782 | -1.284281 |
| H  | -6.374556 | -1.552212 | 0.440893  |
| H  | -6.378716 | 0.940216  | -0.015478 |
| H  | -3.942314 | 0.937047  | 2.778304  |

### Calculation of matrix elements of the spin-orbit Hamiltonian

A new program has been developed for the evaluation of matrix elements of an effective one-electron spin-orbit Hamiltonian between singlet and triplet (or triplet and another triplet) CIS (auxiliary) wave functions. The program deals with excitations from a closed-shell Slater determinant, as well as excitations from a triplet Slater determinant with two unpaired electrons, both spin restricted and unrestricted.

The singlet  $n$ -electron basis is formed from the spin-orbital basis  $\psi = (\phi\alpha \ \phi\beta)$ , where  $\phi$  is the basis of the  $m$  singlet molecular orbitals, and comprises the reference closed-shell Slater determinant

$$|\mathbf{t}\rangle \leftrightarrow |1 \ \dots \ p \ \bar{1} \ \dots \ \bar{p}|,$$

$n = 2p$ , together with all single excitations

$$\frac{1}{\sqrt{2}}(a_{j\alpha}^\dagger a_{i\alpha} + a_{j\beta}^\dagger a_{i\beta})|\mathbf{t}\rangle,$$

$i = 1, \dots, p, j = p+1, \dots, m$ .

The triplet  $n$ -electron basis (with maximum spin projection) is built up from the spin-orbital basis  $\xi = (\omega\alpha \ \tau\beta)$ , where  $\omega$  and  $\tau$  are the bases of the  $m$  alpha and  $m$  beta molecular orbitals, respectively, and consists *either* of all single  $\beta \rightarrow \alpha$  excitations from the closed-shell Slater determinant

$$|\mathbf{t}\rangle \leftrightarrow |1 \ \dots \ p \ \bar{1} \ \dots \ \bar{p}|,$$

$n = 2p$ ,

$$a_{j\alpha}^\dagger a_{i\beta}|\mathbf{t}\rangle,$$

$i = 1, \dots, p, j = p+1, \dots, m$ , or of the reference Slater determinant

$$a_{p+1,\alpha}^\dagger a_{p\beta}|\mathbf{t}\rangle,$$

all single  $\alpha \rightarrow \alpha$  excitations

$$a_{j\alpha}^\dagger a_{i\alpha} a_{p+1,\alpha}^\dagger a_{p\beta}|\mathbf{t}\rangle,$$

$i = 1, \dots, p+1, j = p+2, \dots, m$ , and all single  $\beta \rightarrow \beta$  excitations

$$a_{j\beta}^\dagger a_{i\beta} a_{p+1,\alpha}^\dagger a_{p\beta}|\mathbf{t}\rangle,$$

$i = 1, \dots, p-1, j = p, \dots, m$ . These bases are generally only pure triplet bases if  $\omega = \tau$ . For  $\omega \neq \tau$  the matrix of the total spin square operator  $\hat{S}^2$  is evaluated in the basis of the approximate ‘triplet’ eigenfunctions of the nonrelativistic Hamiltonian to check if it is reasonable to proceed with the calculation of the matrix elements of the spin-orbit Hamiltonian.

The admissible CIS wave functions are therefore of the general formulae

$$|\mathbf{S}; c_0, \mathbf{C}\rangle = c_0|\mathbf{t}\rangle + \frac{1}{\sqrt{2}} \sum_{i=1}^p \sum_{j=p+1}^m c_{ji} (a_{j\alpha}^\dagger a_{i\alpha} + a_{j\beta}^\dagger a_{i\beta})|\mathbf{t}\rangle, \quad (1)$$

where  $\mathbf{C}$  is the  $(m-p)$ -by- $p$  matrix of the singlet CI expansion coefficients,  $\mathbf{C} = \{c_{p+j,i}\}$ ,  $i = 1, \dots, p$ ,  $j = 1, \dots, m-p$ ,

$$|\mathbf{T}; \mathbf{C}\rangle = \sum_{i=1}^p \sum_{j=p+1}^m c_{ji} a_{j\alpha}^\dagger a_{i\beta} |\mathbf{t}\rangle, \quad (2)$$

where  $\mathbf{C}$  is the  $(m-p)$ -by- $p$  matrix of the triplet CI expansion coefficients,  $\mathbf{C} = \{c_{p+j,i}\}$ ,  $i = 1, \dots, p$ ,  $j = 1, \dots, m-p$ , and

$$|\mathbf{T}; c_0, \mathbf{C}_\alpha, \mathbf{C}_\beta\rangle = \left( c_0 + \sum_{i=1}^{p+1} \sum_{j=p+2}^m c_{\alpha ji} a_{j\alpha}^\dagger a_{i\alpha} + \sum_{i=1}^{p-1} \sum_{j=p}^m c_{\beta ji} a_{j\beta}^\dagger a_{i\beta} \right) a_{p+1,\alpha}^\dagger a_{p\beta} |\mathbf{t}\rangle, \quad (3)$$

where  $\mathbf{C}_\alpha$  is the  $(m-p-1)$ -by- $(p+1)$  matrix of the one set of the triplet CI expansion coefficients,  $\mathbf{C}_\alpha = \{c_{\alpha,p+j+1,i}\}$ ,  $i = 1, \dots, p+1$ ,  $j = 1, \dots, m-p-1$ , and  $\mathbf{C}_\beta$  is the  $(m-p+1)$ -by- $(p-1)$  matrix of the other set of the triplet CI expansion coefficients,  $\mathbf{C}_\beta = \{c_{\beta,p+j-1,i}\}$ ,  $i = 1, \dots, p-1$ ,  $j = 1, \dots, m-p+1$ .

While the wave functions (1) and (2) are both true restricted active space (RAS) wave functions [1], namely  $\text{RAS}(p : 1, 0, m-p : 1)$ , the wave function (3) is actually a full class subset of the  $\text{RAS}(p-1 : 1, 2, m-p-1 : 1)$  wave function. Although these wave functions may be built up from three different and independent sets of (singlet, alpha and beta) molecular orbitals, the related matrix elements are still calculated ‘exactly’, on the assumption that the triplet wave functions are eigenfunctions of the total spin square operator, through the biorthonormalization of the two pairs of sets of molecular orbitals (singlet/alpha and singlet/beta) followed by the counter-transformation of the corresponding singlet and triplet CIS expansion coefficients [2].

In a nutshell, if  $\phi \neq \omega$  and/or  $\phi \neq \tau$ , the pair of bases of the molecular orbitals  $\phi$  and  $\eta$  (either  $\omega$  or  $\tau$ ) is, through the LU decomposition of the transition overlap matrix  $\mathbf{S} = \langle \phi | \eta \rangle$ ,

$$\mathbf{PS} = \mathbf{LU}, \quad (4)$$

$l_{ii} = 1$ ,  $i = 1, \dots, m$ , transformed to the new pair of bases, say,

$$\vartheta = \phi \mathbf{P}^T \mathbf{L}^{-\dagger} \quad (5)$$

and

$$\varrho = \eta \mathbf{U}^{-1}, \quad (6)$$

which are mutually biorthonormal,

$$\langle \vartheta | \varrho \rangle = \mathbf{L}^{-1} \mathbf{P} \langle \phi | \eta \rangle \mathbf{U}^{-1} = \mathbf{L}^{-1} \mathbf{PS} \mathbf{U}^{-1} = \mathbf{1}. \quad (7)$$

This is the necessary first step towards the efficient evaluation of the matrix elements between eigenfunctions of the nonrelativistic Hamiltonian of different spin multiplicities (unless the molecular orbitals are not allowed to relax in the course of the HF or KS SCF calculations). The second step is the counter-transformation of the CI expansion coefficients of the singlet and triplet, whose effect is to compensate for the orbital alterations so as to keep the multielectron wave functions unchanged [3, 4, 5].

The employed effective one-electron spin-orbit Hamiltonian is the sum of the Breit-Pauli (or Douglas-Kroll-Hess) one-electron spin-orbit Hamiltonian [6] (which itself is a sum of contributions of individual atoms of a molecule) and an approximation to the “two-electron” part of the ‘exact’ Breit-Pauli (or Douglas-Kroll-Hess) one-electron mean-field spin-orbit Hamiltonian [7]. The approximation is a gentle modification of the so-called flexible nuclear screening spin-orbit (FNSSO) approximation [8] showing mean relative error below a few percent for virtually all elements of the periodic table in most bonding situations. The accuracy of the approximation has proven [8, 9] to be comparable to the popular, but significantly more expensive, atomic mean-field integral (AMFI) approximation [10]. The calculation of the demanding two-electron spin-orbit integrals is nevertheless completely avoided. As far as speed is concerned, the approximation almost comes up to the simplest one-electron effective nuclear charge approaches [11] from which it differs in two important aspects: the effective nuclear charge is represented by a continuous multivariable basis set independent function rather than by a single real number per element, and both one- and two-center contributions are taken into account.

A more descriptive view at the approximation is based on the explicit form of e.g. the Breit-Pauli one-electron spin-orbit Hamiltonian [6] (in SI units)

$$\hat{h}(1) = \frac{e^2}{8\pi\epsilon_0 m^2 c^2} \sum_C Z_C r_C^{-3} (\mathbf{r}_C \times \hat{\mathbf{p}}) \cdot \hat{\mathbf{s}}, \quad (8)$$

where  $\epsilon_0$  is the permittivity of vacuum,  $c$  is the velocity of light in vacuum,  $e$  is the charge and  $m$  is the mass of an electron,  $Z_C$  is the number of protons ( $Z_C e$  is the charge) of the nucleus  $C$ ,  $\mathbf{r}_C$  is the position vector of an electron with respect to the nucleus  $C$ ,  $r_C = |\mathbf{r}_C|$ , and  $\hat{\mathbf{p}}$  or  $\hat{\mathbf{s}}$  is the operator of the vector of linear momentum or spin angular momentum of an electron, respectively. Accordingly, the employed effective spin-orbit Hamiltonian is essentially the Breit-Pauli (or Douglas-Kroll-Hess) one-electron spin-orbit Hamiltonian in which, for each nucleus  $C$ , the true nuclear charge  $Z_C e$  has been replaced with an effective nuclear charge  $(1 - q_C)Z_C e$ , where the so-called screening quotient  $q_C \equiv q_C(l, \alpha, \beta) \in \langle 0, 1 \rangle$  depends not only on the nucleus  $C$ , but also on the two one-electron primitive Gaussian functions bracketing the operator in a particular one-center matrix element—through their common azimuthal quantum number  $l$  (describing their angular parts) and individual exponents  $\alpha$  and  $\beta$  (describing their radial parts). Clearly, an electron close enough to the atomic nucleus experiences only the electric field brought by the positive nuclear charge  $Z_C e$  (as the contributions of all the electrons of the atom to the spherically symmetric electric field at the position of the nucleus mutually cancel) while an electron in the infinity experiences just the zero electric field of the neutral atom. Therefore, the quotient  $q_C$  should almost vanish for the tightest basis functions and should approach 1 for the sufficiently diffuse ones. Moreover, the quotient  $q_C$  should never be lower than 0 or greater than 1 as the fictitious electron can nowhere in space experience a spherically symmetric electric field of a positive charge greater than  $Z_C e$  or of a negative charge.

The dependence of  $q_C$  on the variables  $l$ ,  $\alpha$  and  $\beta$  has been determined through nonrelativistic (or scalar relativistic) full-valence CASSCF calculations on the ground

states of neutral atoms (employing large *uncontracted* one-electron bases) followed by the evaluation of the nonzero matrix elements of the ‘exact’ Breit–Pauli (or Douglas–Kroll–Hess) one-electron mean-field spin–orbit Hamiltonian.

The contribution of a heavy atom on which a two-component (relativistic,  $j$ -dependent) pseudopotential [12] is defined (and a reduced number of basis functions are considered to represent just the pseudovalence orbitals instead of the full set of core and valence orbitals) to matrix elements of the effective one-electron spin–orbit Hamiltonian is best evaluated using an operator implicitly included in the two-component pseudopotential itself [13].

The central idea behind the pseudopotential approximation [14, 15, 16, 17, 18, 19, 20] is to select from the total number of  $n$  (actually indistinguishable!) electrons of a molecule the  $q$  valence electrons (responsible for all the chemistry) that are moving in the electric field of the remaining  $n - q$  core electrons and the positively charged nuclei (to which the core electrons are “stuck” in exactly the same way as in the isolated atoms). Heavy nuclei are thus replaced with spherical cores, while  $Q_C e$  is the charge of the core whose center is at the nucleus  $C$  with the charge  $Z_C e$ ,  $0 < Q_C < Z_C$ . Consequently,

$$q = n - \sum_C (Z_C - Q_C).$$

Point-like cores can be regarded as the roughest, zero-order, approximation. Therefore, the valence-only effective Hamiltonian of a molecule (in SI units)

$$\begin{aligned} \hat{H}(1, \dots, q) = & -\frac{\hbar^2}{2m} \sum_{i=1}^q \nabla_i^2 + \frac{e^2}{4\pi\epsilon_0} \left\{ \sum_{i=1}^q \sum_C \left[ -\frac{Q_C}{r_{iC}} + \Delta_{vC}(r_{iC}) \right] \right. \\ & \left. + \sum_{i=1}^q \sum_{j>i}^q \frac{1}{r_{ij}} + \sum_C \sum_{D>C} \frac{Q_C Q_D}{r_{CD}} \right\} \end{aligned} \quad (9)$$

may be introduced which, in its simplest practicable form, stands for kinetic energy of the valence electrons and potential energy of the Coulombic (*i*) attraction between the valence electrons and the cores (taking into account also the correction for the error of the zero-order approximation by means of pre-parameterized, through all-electron *relativistic* calculations on atoms or their ions, one-electron operators  $\Delta_{vC}$  called pseudopotentials), (*ii*) repulsion between the valence electrons, and (*iii*) repulsion between the (point-like) cores, where  $\hbar$  is the reduced Planck constant,  $\epsilon_0$  is the permittivity of vacuum,  $e$  is the charge and  $m$  is the mass of an electron,  $r_{iC}$  is the distance between the electron  $i$  and the nucleus  $C$  while  $r_{ij}$  or  $r_{CD}$  is the distance between two electrons or two nuclei (point-like cores), respectively. The energy of the cores themselves is supposed to be a constant and has been subtracted.

Pseudopotentials are thus intended to model, in a mean-field manner, core-valence interactions of electrons as well as core-valence orbital orthogonality constraints in atoms and molecules. The main benefit of using pseudopotentials is the reduction of computational demands of electronic structure calculations (largely due to the decrease of the number of one-electron basis functions) while nearly maintaining the accuracy of the

calculations. The added value is the fact that, for atoms of heavy elements, the most important relativistic effects are included in the pre-computed parameters and, in the case of scalar relativistic effects, do not even have to be treated explicitly.

For properly designed pseudopotentials, the lowest-energy eigenfunctions of the related one-electron mean-field (HF or KS) Hamiltonian describe valence states and have nodeless radial parts. Accordingly, a correctly parameterized pseudopotential effectively “shifts” relativistic effects (including, with a 2-component pseudopotential, also spin-orbit coupling) from the core to the valence region of the molecule.

The pseudopotential  $\Delta v_C$  is a smooth function of the distance of an electron from the nucleus  $C$  and is generally different for basis functions of different angular symmetries. It is repulsive in the short range (so as to keep the valence electrons out of the core) and attractive in the long range. Typically,  $Q_C$  differs from  $Z_C$  only for the atoms of the heaviest elements, often just one or two atoms in the molecule. For atoms with  $Q_C = Z_C$  the pseudopotential  $\Delta v_C$  clearly vanishes and full one-electron basis is required. The contribution of such an atom to matrix elements of the effective one-electron spin-orbit Hamiltonian is then calculated using the (Breit–Pauli variant of the) *one-center* FNSSO approximation described above. For atoms with  $Q_C < Z_C$  the related part of the *one-center* effective spin-orbit Hamiltonian is extracted from the two-component pseudopotential  $\Delta v_C$  by spin separation [13].

It should be mentioned that in the aforesaid typical case, where pseudopotentials are only defined for a subset of the atoms of a molecule, the one-center approximation to spin-orbit coupling seems to be the natural choice. Clearly, if the multicenter contributions were evaluated using an all-electron spin-orbit Hamiltonian on lighter atoms, they would be incomplete and thus incorrect due to the missing tight basis functions describing core orbitals on the heavy atoms with pseudopotentials. Then it is perhaps better not to calculate them at all. However, if the multicenter contributions are not calculated on the lighter atoms, they should probably not be calculated on the heavy atoms either to avoid unbalanced treatment.

one-component (nonrelativistic or scalar relativistic,  $l$ -dependent) pseudopotential

$$\Delta v(r) = \begin{pmatrix} \Delta v(r) & 0 \\ 0 & \Delta v(r) \end{pmatrix} \equiv \Delta v(r) = \sum_{l=0}^{\infty} v_l(r) \hat{P}_l$$

azimuthal quantum number  $l \geq 0$

$$\hat{P}_l = \sum_{m=-l}^l |l, m\rangle \langle l, m| = \sum_{m=-l}^l |l; m\rangle \langle l; m|$$

magnetic quantum number  $m \leq |l|$

$$|l, m\rangle \equiv Y_{lm}(\vartheta, \varphi)$$

common eigenfunctions of the operators  $\hat{l}^2$  and  $\hat{l}_z$ , the so-called spherical harmonics

$$|l; m\rangle \equiv S_{lm}(\vartheta, \varphi)$$

real linear combinations of (complex) spherical harmonics

$$S_{l0} = Y_{l0}$$

for  $m > 0$

$$S_{lm} = \frac{1}{\sqrt{2}}[(-1)^m Y_{lm} + Y_{l,-m}]$$

$$S_{l,-m} = -\frac{i}{\sqrt{2}}[(-1)^m Y_{lm} - Y_{l,-m}]$$

The projection operators  $\hat{P}_l$ ,  $l \geq 0$ , ensure that each of the operators  $\hat{v}_l(r)$  acts only on the components of the one-electron basis functions with the proper angular symmetry. Since spherical harmonics form a complete set of functions, the projection operators  $\hat{P}_l$  fulfill the completeness relation

$$\sum_{l=0}^{\infty} \hat{P}_l = 1.$$

for  $l > u \gg 0$ , where  $u - 1$  is the highest  $l$  found in the core

$$v_l(r) \doteq v_u(r)$$

avoiding infinite summation by exploiting the completeness relation for the projection operators  $\hat{P}_l$

$$\begin{aligned} \Delta v(r) &\doteq \sum_{l=0}^{u-1} v_l(r) \hat{P}_l + v_u(r) \sum_{l=u}^{\infty} \hat{P}_l \\ &= \sum_{l=0}^{u-1} v_l(r) \hat{P}_l + v_u(r) \sum_{l=u}^{\infty} \hat{P}_l + v_u(r) \left[ 1 - \sum_{l=0}^{\infty} \hat{P}_l \right] \\ &= \sum_{l=0}^{u-1} v_l(r) \hat{P}_l + v_u(r) - v_u(r) \sum_{l=0}^{u-1} \hat{P}_l \\ &= v_u(r) + \sum_{l=0}^{u-1} [v_l(r) - v_u(r)] \hat{P}_l \end{aligned}$$

two-component (relativistic,  $j$ -dependent) pseudopotential

$$\begin{aligned} \Delta v(r) &= \sum_{l=0}^{\infty} \sum_{j=|l-\frac{1}{2}|}^{l+\frac{1}{2}} v_{lj}(r) P_{lj} \\ &= v_{0,1/2}(r) P_{0,1/2} + \sum_{l=1}^{\infty} [v_{l,l-1/2}(r) P_{l,l-1/2} + v_{l,l+1/2}(r) P_{l,l+1/2}] \end{aligned}$$

spin quantum number  $s = \frac{1}{2}$ ,  $j = l \mp s = l \mp \frac{1}{2}$

$$P_{lj} = \sum_{m=-j}^j |l, j, m\rangle \langle l, j, m|$$

coupling of angular momenta

$$\hat{\mathbf{j}} = \hat{\mathbf{l}} + \hat{\mathbf{s}}$$

common eigenfunctions of the operators  $\hat{j}^2$  and  $\hat{j}_z$

$$|l, j, m\rangle \equiv |l, l \mp \frac{1}{2}, m\rangle = \mp \sqrt{\frac{l \mp m + \frac{1}{2}}{2l+1}} Y_{l, m-1/2} \alpha + \sqrt{\frac{l \pm m + \frac{1}{2}}{2l+1}} Y_{l, m+1/2} \beta$$

$$\leftrightarrow \frac{1}{\sqrt{2l+1}} \begin{pmatrix} \mp \sqrt{l \mp m + \frac{1}{2}} Y_{l, m-1/2} \\ \sqrt{l \pm m + \frac{1}{2}} Y_{l, m+1/2} \end{pmatrix}$$

the elementary spin functions  $\alpha$  and  $\beta$  are common eigenfunctions of the operators  $\hat{s}^2$  and  $\hat{s}_z$

$$|l, l \mp \frac{1}{2}, m\rangle \langle l, l \mp \frac{1}{2}, m| = \frac{1}{2l+1} \left\{ \begin{aligned} & (l \mp m + \frac{1}{2}) |l, m - \frac{1}{2}\rangle \langle l, m - \frac{1}{2}| \\ & \mp \sqrt{(l \mp m + \frac{1}{2})(l \pm m + \frac{1}{2})} |l, m + \frac{1}{2}\rangle \langle l, m - \frac{1}{2}| \\ & \mp \sqrt{(l \mp m + \frac{1}{2})(l \pm m + \frac{1}{2})} |l, m - \frac{1}{2}\rangle \langle l, m + \frac{1}{2}| \\ & (l \pm m + \frac{1}{2}) |l, m + \frac{1}{2}\rangle \langle l, m + \frac{1}{2}| \end{aligned} \right\}$$

$P_{lj}$  is a 2-by-2 matrix

$$\sum_{j=|l-\frac{1}{2}|}^{l+\frac{1}{2}} P_{lj} = \begin{pmatrix} \hat{P}_l & 0 \\ 0 & \hat{P}_l \end{pmatrix} \equiv \hat{P}_l$$

$$P_{0,1/2} = \hat{P}_0$$

for  $l > 0$

$$P_{l,l-1/2} + P_{l,l+1/2} = \hat{P}_l$$

$$P_{l,l-1/2} = \sum_{m=-l+1/2}^{l-1/2} |l, l - \frac{1}{2}, m\rangle \langle l, l - \frac{1}{2}, m| = \frac{1}{2l+1} (l\hat{P}_l - R_l)$$

$$P_{l,l+1/2} = \sum_{m=-l-1/2}^{l+1/2} |l, l + \frac{1}{2}, m\rangle \langle l, l + \frac{1}{2}, m| = \frac{1}{2l+1} [(l+1)\hat{P}_l + R_l]$$

$$R_l = lP_{l,l+1/2} - (l+1)P_{l,l-1/2} = \frac{1}{\hbar} (\hat{P}_l \hat{l}_x \hat{P}_l \sigma_x + \hat{P}_l \hat{l}_y \hat{P}_l \sigma_y + \hat{P}_l \hat{l}_z \hat{P}_l \sigma_z)$$

$$= \frac{1}{\hbar} \hat{P}_l \hat{\mathbf{l}} \hat{P}_l \cdot \boldsymbol{\sigma} \leftrightarrow \frac{2}{\hbar^2} \hat{P}_l \hat{\mathbf{l}} \hat{P}_l \cdot \hat{\mathbf{s}}$$

$$\hat{P}_l \hat{l}_u \hat{P}_l = \sum_{q=-l}^l \sum_{m=-l}^l |l, q\rangle \langle l, q| \hat{l}_u |l, m\rangle \langle l, m| = \sum_{q=-l}^l \sum_{m=-l}^l |l; q\rangle \langle l; q| \hat{l}_u |l; m\rangle \langle l; m|$$

$u = x, y, z$

$$\sigma_x = \begin{pmatrix} 0 & 1 \\ 1 & 0 \end{pmatrix}, \quad \sigma_y = \begin{pmatrix} 0 & -i \\ i & 0 \end{pmatrix}, \quad \sigma_z = \begin{pmatrix} 1 & 0 \\ 0 & -1 \end{pmatrix}$$

$\boldsymbol{\sigma}$  is the vector of 2-by-2 Pauli spin matrices  $\sigma_x$ ,  $\sigma_y$  and  $\sigma_z$

$$\frac{\hbar}{2} \boldsymbol{\sigma} \leftrightarrow \hat{\mathbf{s}}$$

a relation derived by comparing  $\boldsymbol{\sigma}$  with the 2-by-2 matrix of the operator  $\hat{\mathbf{s}}$  in the basis of the elementary spin functions  $\alpha$  and  $\beta$

$$\begin{pmatrix} \langle \alpha | \\ \langle \beta | \end{pmatrix} \hat{\mathbf{s}} \begin{pmatrix} | \alpha \rangle & | \beta \rangle \end{pmatrix} = \begin{pmatrix} \langle \alpha | \hat{\mathbf{s}} | \alpha \rangle & \langle \alpha | \hat{\mathbf{s}} | \beta \rangle \\ \langle \beta | \hat{\mathbf{s}} | \alpha \rangle & \langle \beta | \hat{\mathbf{s}} | \beta \rangle \end{pmatrix} = \frac{\hbar}{2} \boldsymbol{\sigma}$$



for  $l > u \gg 0$ , where  $u$  is typically one more than the highest  $l$  found in the core

$$v_{l,l-1/2}(r) \doteq v_{l,l+1/2}(r) \doteq v_l(r) \doteq v_u(r)$$

avoiding infinite summation by exploiting the completeness relation for the projection operators  $\hat{P}_l$

$$\begin{aligned}
\Delta v(r) &\doteq \sum_{l=0}^{u-1} \sum_{j=|l-\frac{1}{2}|}^{l+\frac{1}{2}} v_{lj}(r) P_{lj} + v_u(r) \sum_{l=u}^{\infty} \hat{P}_l \\
&= \sum_{l=0}^{u-1} \sum_{j=|l-\frac{1}{2}|}^{l+\frac{1}{2}} v_{lj}(r) P_{lj} + v_u(r) \sum_{l=u}^{\infty} \hat{P}_l + v_u(r) \left[ 1 - \sum_{l=0}^{\infty} \hat{P}_l \right] \\
&= \sum_{l=0}^{u-1} \sum_{j=|l-\frac{1}{2}|}^{l+\frac{1}{2}} v_{lj}(r) P_{lj} + v_u(r) - v_u(r) \sum_{l=0}^{u-1} \hat{P}_l \\
&= \sum_{l=0}^{u-1} \sum_{j=|l-\frac{1}{2}|}^{l+\frac{1}{2}} v_{lj}(r) P_{lj} + v_u(r) - v_u(r) \sum_{l=0}^{u-1} \sum_{j=|l-\frac{1}{2}|}^{l+\frac{1}{2}} P_{lj} \\
&= v_u(r) + \sum_{l=0}^{u-1} \sum_{j=|l-\frac{1}{2}|}^{l+\frac{1}{2}} [v_{lj}(r) - v_u(r)] P_{lj} \\
&= v_u(r) + [v_{0,1/2}(r) - v_u(r)] P_{0,1/2} \\
&+ \sum_{l=1}^{u-1} \left\{ [v_{l,l-1/2}(r) - v_u(r)] P_{l,l-1/2} + [v_{l,l+1/2}(r) - v_u(r)] P_{l,l+1/2} \right\} \\
&= v_u(r) + [v_{0,1/2}(r) - v_u(r)] \hat{P}_0 \\
&+ \sum_{l=1}^{u-1} \left\{ \frac{l}{2l+1} [v_{l,l-1/2}(r) - v_u(r)] + \frac{l+1}{2l+1} [v_{l,l+1/2}(r) - v_u(r)] \right\} \hat{P}_l \\
&+ \sum_{l=1}^{u-1} \left\{ \frac{1}{2l+1} [v_{l,l+1/2}(r) - v_u(r)] - \frac{1}{2l+1} [v_{l,l-1/2}(r) - v_u(r)] \right\} R_l \\
&= v_u(r) + [v_{0,1/2}(r) - v_u(r)] \hat{P}_0 \\
&+ \sum_{l=1}^{u-1} \left\{ \frac{1}{2l+1} [lv_{l,l-1/2}(r) + (l+1)v_{l,l+1/2}(r)] - v_u(r) \right\} \hat{P}_l \\
&+ \sum_{l=1}^{u-1} \frac{1}{2l+1} [v_{l,l+1/2}(r) - v_{l,l-1/2}(r)] R_l \\
&= v_u(r) + \sum_{l=0}^{u-1} [v_l(r) - v_u(r)] \hat{P}_l + \sum_{l=1}^{u-1} \frac{1}{2l+1} \Delta v_l(r) R_l
\end{aligned}$$

spin averaged

$$v_0(r) = v_{0,1/2}(r)$$

for  $l \in \langle 1, u \rangle$

$$v_l(r) = \frac{1}{2l+1} [lv_{l,l-1/2}(r) + (l+1)v_{l,l+1/2}(r)]$$

$$\Delta v_l(r) = v_{l,l+1/2}(r) - v_{l,l-1/2}(r)$$

convenient analytical form of both  $v_0(r)$  and  $v_{l,l\mp 1/2}(r)$ , and thus also of  $v_l(r)$  and  $\Delta v_l(r)$ ,  $l > 0$ , is

$$\frac{1}{r^2} \sum_{i=1}^k c_i r^{n_i} e^{-\alpha_i r^2}$$

$$n_i \in N$$

$$c_i, \alpha_i \in R$$

$$k \approx 4$$

$$n_i \in \{0, 1, \mathbf{2}, \mathfrak{3}, 4, \dots\}$$

$$\alpha_i > 0$$

Cartesian Gaussian functions

$$\xi(m, n, q, \alpha; \mathbf{r}) = x^m y^n z^q e^{-\alpha r^2} = x^m e^{-\alpha x^2} y^n e^{-\alpha y^2} z^q e^{-\alpha z^2}$$

*nonredundant* Cartesian Gaussian functions

$$\chi(l, m, \alpha; \mathbf{r}) = r^l e^{-\alpha r^2} S_{lm}(\vartheta, \varphi)$$

complex solid harmonics

$$r^l Y_{lm}(\vartheta, \varphi)$$

real solid harmonics

$$r^l S_{lm}(\vartheta, \varphi)$$

normalized atomic orbitals

$$2 \left[ \frac{(2\alpha)^3}{\pi} \right]^{\frac{1}{4}} \sqrt{\frac{2^l}{(2l+1)!!}} \left( \sqrt{2\alpha} r \right)^l e^{-\alpha r^2} S_{lm}(\vartheta, \varphi) = \frac{2^{l+1}}{\sqrt{(2l+1)!!}} \left( \frac{8}{\pi} \right)^{\frac{1}{4}} \alpha^{\frac{2l+3}{4}} \chi(l, m, \alpha; \mathbf{r})$$

the contribution of the atom to matrix elements of the effective spin-orbit Hamiltonian is calculated as a linear combination of one-center integrals

$$\begin{aligned} & \int_{-\infty}^{\infty} \int_{-\infty}^{\infty} \int_{-\infty}^{\infty} \chi(k, p, \alpha; \mathbf{r}) |l; q\rangle \langle l; q | \hat{l}_u | l; m\rangle \langle l; m | \chi(o, t, \beta; \mathbf{r}) r^{n-2} e^{-\gamma r^2} dx dy dz \\ &= \langle l; q | \hat{l}_u | l; m\rangle \int_0^{\infty} r^{k+n+o} e^{-(\alpha+\beta+\gamma)r^2} dr \int_0^{\pi} \left[ \int_0^{2\pi} S_{kp}(\vartheta, \varphi) S_{lq}(\vartheta, \varphi) d\varphi \right] \sin \vartheta d\vartheta \\ & \quad \times \int_0^{\pi} \left[ \int_0^{2\pi} S_{lm}(\vartheta, \varphi) S_{ot}(\vartheta, \varphi) d\varphi \right] \sin \vartheta d\vartheta \\ &= \delta_{kl} \delta_{lo} \delta_{pq} \delta_{mt} \langle l; q | \hat{l}_u | l; m\rangle \int_0^{\infty} r^{2l+n} e^{-(\alpha+\beta+\gamma)r^2} dr \end{aligned}$$

$u = x, y, z$

for  $n \geq 0$  and  $a > 0$

$$\int_0^{\infty} x^{2n} e^{-ax^2} dx = \frac{1}{2} \left( \frac{\pi}{a} \right)^{\frac{1}{2}} \frac{(2n-1)!!}{(2a)^n}$$

$$\int_0^\infty x^{2n+1} e^{-ax^2} dx = \frac{n!}{2a^{n+1}}$$

solution in a closed form

$$\frac{2^{2l+2}}{(2l+1)!!} \left(\frac{8}{\pi}\right)^{\frac{1}{2}} (\alpha\beta)^{\frac{2l+3}{4}} \int_0^\infty r^{2l+n} e^{-(\alpha+\beta+\gamma)r^2} dr = \dots$$

for even  $n$

$$\begin{aligned} \dots &= \frac{2^{2l+2}}{(2l+1)!!} \left(\frac{8}{\pi}\right)^{\frac{1}{2}} (\alpha\beta)^{\frac{2l+3}{4}} \frac{1}{2} \left(\frac{\pi}{\alpha+\beta+\gamma}\right)^{\frac{1}{2}} \frac{(2l+n-1)!!}{[2(\alpha+\beta+\gamma)]^{l+\frac{n}{2}}} \\ &= 2^{\frac{2l-n+5}{2}} \frac{(2l+n-1)!!}{(2l+1)!!} \frac{(\alpha\beta)^{\frac{2l+3}{4}}}{(\alpha+\beta+\gamma)^{\frac{2l+n+1}{2}}} \end{aligned}$$

special case for  $n = 2$

$$\dots = 2^{\frac{2l+3}{2}} \frac{(\alpha\beta)^{\frac{2l+3}{4}}}{(\alpha+\beta+\gamma)^{\frac{2l+3}{2}}} = \left[ \frac{2(\alpha\beta)^{\frac{1}{2}}}{\alpha+\beta+\gamma} \right]^{\frac{2l+3}{2}}$$

for odd  $n$

$$\begin{aligned} \dots &= \frac{2^{2l+2}}{(2l+1)!!} \left(\frac{8}{\pi}\right)^{\frac{1}{2}} (\alpha\beta)^{\frac{2l+3}{4}} \frac{\left(\frac{2l+n-1}{2}\right)!}{2(\alpha+\beta+\gamma)^{\frac{2l+n+1}{2}}} \\ &= 2^{\frac{4l+5}{2}} \frac{\left(\frac{2l+n-1}{2}\right)!}{(2l+1)!!} \frac{(\alpha\beta)^{\frac{2l+3}{4}}}{(\alpha+\beta+\gamma)^{\frac{2l+n+1}{2}}} \end{aligned}$$

In spite of all the uncommon features of our program, it turns out that the time spent by the calculation of spin-orbit couplings between multielectron wave functions is still a negligible fraction of the time needed for carrying out spin forbidden nonadiabatic molecular dynamics simulation as a whole.

## References

- [1] J. Olsen and B. O. Roos and P. Jørgensen and H. J. Aa. Jensen J. Chem. Phys. 89 1988 2185–2192
- [2] M. Kývala to be published
- [3] P. -Å. Malmqvist Int. J. Quantum Chem. 30 1986 479–494
- [4] T. Helgaker and P. Jørgensen and J. Olsen *Molecular Electronic-Structure Theory* Wiley Chichester 2000 569–573
- [5] M. Kývala Int. J. Quantum Chem. 109 2009 1200–1207
- [6] B. A. Hess and C. M. Marian and S. D. Peyerimhoff in *Modern Electronic Structure Theory Part I* D. R. Yarkony editor World Scientific Singapore 1995 152–278

- [7] B. A. Hess and C. M. Marian and U. Wahlgren and O. Gropen Chem. Phys. Lett. 251 1996 365–371
- [8] J. Chalupský and T. Yanai J. Chem. Phys. 139 2013 204106
- [9] M. Kývala unpublished
- [10] B. Schimmelpfennig PhD Thesis Stockholm University 1996
- [11] N. Matsunaga and S. Koseki in *Reviews in Computational Chemistry Volume 20* K. B. Lipkowitz and R. Larter and T. R. Cundari editors John Wiley & Sons New Jersey 2004 101–152
- [12] Y. S. Lee and W. C. Ermler and R. M. Pitzer J. Chem. Phys. 67 1977 5861–5876
- [13] R. M. Pitzer and N. W. Winter J. Phys. Chem. 92 1988 3061–3063
- [14] T. R. Cundari and M. T. Benson and M. L. Lutz and S. O. Sommerer in *Reviews in Computational Chemistry Volume 8* K. B. Lipkowitz and D. B. Boyd editors WCH Publishers New York 1996 145–202
- [15] M. Dolg in *Relativistic Electronic Structure Theory Part 1. Fundamentals* P. Schwerdtfeger editor Elsevier Amsterdam 2002 793–862
- [16] P. Schwerdtfeger in *Theoretical Chemistry and Physics of Heavy and Superheavy Elements* U. Kaldor and S. Wilson editors Kluwer Academic Publishers Dordrecht 2003 399–438
- [17] K. G. Dyall and K. Fægri, Jr. *Introduction to Relativistic Quantum Chemistry* Oxford University Press New York 2007 396–426
- [18] X. Cao and M. Dolg in *Relativistic Methods for Chemists* M. Barysz and Y. Ishikawa editors Springer Dordrecht 2010 215–277
- [19] P. Schwerdtfeger ChemPhysChem 12 2011 3143–3155
- [20] M. Dolg and X. Cao Chem. Rev. 112 2012 403–480
